# Supplementary material for: Harmonized Estimation of Subgroup-Specific Treatment Effects in Randomized Trials: The Use of External Control Data
Source: arXiv:2308.05073 ancillary file (2025-02-11)
Supplement: Supplementary file 1 [file RWD_Subgroup_Supplement.pdf]

# Supplementary Information for

## “Harmonized Estimation of Subgroup-Specific Treatment Effects in Randomized Trials: The Use of External Control Data”

Daniel Schwartz<sup>1,3</sup>, Riddhiman Saha<sup>1</sup>, Steffen Ventz<sup>2</sup>, and Lorenzo Trippa<sup>1,3</sup>

<sup>1</sup>Department of Biostatistics, Harvard T.H. Chan School of Public Health

<sup>2</sup>Division of Biostatistics, School of Public Health, University of Minnesota

<sup>3</sup>Department of Data Science, Dana-Farber Cancer Institute

January 29, 2025

### Contents

|                                                                                |           |
|--------------------------------------------------------------------------------|-----------|
| <b>S1 Full notation dictionary</b>                                             | <b>2</b>  |
| <b>S2 Additional material for Section 2</b>                                    | <b>7</b>  |
| S2.1 Proofs for Section 2.1 (derivation of the harmonized estimator) . . . . . | 7         |
| S2.2 Proofs for Section 2.2 (Proposition 1 and its generalization) . . . . .   | 8         |
| S2.2.1 Generalization . . . . .                                                | 8         |
| S2.2.2 Proposition 1 (special case) . . . . .                                  | 11        |
| S2.3 Replication of Figure 1 by simulation . . . . .                           | 12        |
| S2.4 Proofs for Section 2.3 (Bayesian interpretation) . . . . .                | 12        |
| S2.4.1 Main result . . . . .                                                   | 14        |
| S2.4.2 Approach of the derivation . . . . .                                    | 14        |
| S2.4.3 Computing the mean . . . . .                                            | 15        |
| S2.4.4 Computing the variance . . . . .                                        | 16        |
| S2.4.5 Condition for the cut estimator in Section 2.3 to be unbiased . . . . . | 18        |
| S2.5 Details for Figure 2 (Cut distribution example) . . . . .                 | 19        |
| S2.6 Proof for Section 2.4 (Interval estimation) . . . . .                     | 19        |
| S2.7 Splitting and merging subgroups . . . . .                                 | 20        |
| S2.8 Large sample behavior of harmonization . . . . .                          | 21        |
| <b>S3 Additional material for Section 3</b>                                    | <b>23</b> |
| S3.1 Proofs for Section 3.1 (linear regression) . . . . .                      | 23        |
| S3.1.1 Bias and variance of $\hat{\theta}_{1:K}^{(r+e)}$ . . . . .             | 23        |
| S3.1.2 Unbiasedness of $\hat{\theta}^{(r)}$ . . . . .                          | 24        |
| S3.1.3 Propositions 3-5 . . . . .                                              | 24        |

|           |                                                                                                  |           |
|-----------|--------------------------------------------------------------------------------------------------|-----------|
| S3.2      | Scatter plot comparing the BD harmonized and cut distribution estimators in 3.1 . . .            | 26        |
| S3.3      | Proofs for Section 3.2 (logistic regression) . . . . .                                           | 26        |
| S3.3.1    | Limiting value of $\hat{\theta}_{1:K}^{(r+e)}$ (results) . . . . .                               | 26        |
| S3.3.2    | Limiting value of $\hat{\theta}_{1:K}^{(r+e)}$ (proofs) . . . . .                                | 28        |
| S3.3.3    | Proof of Proposition 5 . . . . .                                                                 | 31        |
| S3.4      | Simulation details for Section 3.2 . . . . .                                                     | 31        |
| S3.4.1    | Taking $\Sigma$ as a variance estimate . . . . .                                                 | 31        |
| S3.4.2    | Simulation settings . . . . .                                                                    | 32        |
| S3.4.3    | Version of Figure 5 with $\delta_{1:K}$ varying across subgroup . . . . .                        | 32        |
| S3.5      | Computation of $B$ for Section 3.3 . . . . .                                                     | 32        |
| S3.6      | Generalized linear models . . . . .                                                              | 32        |
| S3.7      | Supplementary simulations for additional input estimators $\hat{\theta}_{1:K}^{(r+e)}$ . . . . . | 36        |
| S3.7.1    | Bayesian causal forests . . . . .                                                                | 36        |
| S3.7.2    | Bayesian logistic regression with borrowing across subgroups . . . . .                           | 36        |
| S3.7.3    | The propensity score adjusted power prior method . . . . .                                       | 38        |
| S3.8      | Testing the systematic distortion mechanism (SDM) assumption . . . . .                           | 40        |
| S3.9      | A bootstrap procedure to estimate and remove the bias $\psi_{1:K}$ of a pooled estimator . .     | 42        |
| S3.10     | BD harmonization of semiparametric and nonparametric estimators . . . . .                        | 42        |
| <b>S4</b> | <b>Additional material for Section 4</b>                                                         | <b>44</b> |
| S4.1      | Imputation of censored 12-month survival outcomes . . . . .                                      | 44        |
| S4.2      | Detailed results . . . . .                                                                       | 45        |
| <b>S5</b> | <b>Harmonization in the presence of omitted variable bias</b>                                    | <b>45</b> |

## S1 Full notation dictionary

Here we list all notation used in the *main text* of the paper, where more precise definitions are given. The order is alphabetical, with Roman and Greek letters intermixed and some numerical/math notation at the end.

- $a = 1, \dots, R$ : bootstrap replicates
- $A$ : generic set in  $\mathbb{R}^{K-1}$
- $(A1), (A2)$ : superscripts indicating probability with respect to Analyst 1's or Analyst 2's model
- $\alpha: \in (0, 1)$ , level of confidence interval
- $B$ : bias matrix in Proposition 3
- $\hat{B}$ : estimate of  $B$
- $B^h$ : bias of harmonized estimator in simple setting
- $b = (b_1, \dots, b_K) = B1_{K \times 1}$ : row sums of  $B$  matrix

- $\hat{b} = (\hat{b}_1, \dots, \hat{b}_K) = \hat{B}1_{K \times 1}$ : estimate of  $b$
- $\beta$ :  $d$ -dimensional vector of regression coefficients for covariate vector  $X$  (used in both linear and logit models)
- $\hat{\beta}^{(r+e)}$ : MLE of  $\beta$  under model (29) (pooled logistic regression at beginning of 3.2)
- $\hat{\beta}^{(r)}$ : MLE of  $\beta$  under version of logistic model (29) using RCT data only
- $\beta^\circ$ : limit in probability of  $\hat{\beta}^{(r+e)}$  in the logistic regression example (Section 3.2)
- $c = (\pi^\top \Sigma \pi)^{-1}$ : constant used in definition of harmonized estimator
- $c' = (\pi'^\top \Sigma' \pi')^{-1}$ : constant for harmonized estimator when groups  $K$  and  $K - 1$  are merged
- $Cov(Z, U)$ : covariance between random variables/vectors  $Z$  and  $U$ , i.e.  $E((Z - E(Z))(U - E(U))^\top)$
- $(cut)$ : superscript indicating probability with respect to the plug-in distribution in Section 2.3
- $\gamma_{1:K} = (\gamma_1, \dots, \gamma_K)$ : subgroup-specific mean outcome difference of EC vs. RCT controls
- $D^{(r)}, D^{(e)}$ : data sets for the RCT and EC respectively, including variables  $(T_i, W_i, Y_i, X_i)$
- $D_a^{(r)}, D_a^{(e)}$ : the  $a$ -th bootstrap replicate of  $D^{(r)}, D^{(e)}$
- $d$ : dimension of covariates  $X_i$
- $diag(a_k)$ : diagonal matrix with  $k \times k$ -th entry  $= a_k$
- $\Delta_\gamma$ : parameter controlling difference in  $\gamma_{1:K}$  between successive subgroups, i.e.  $\gamma_{1:K} = (\gamma + \Delta_\gamma, \gamma - \Delta_\gamma, \gamma + \Delta_\gamma, \dots)$  for  $\gamma \in \mathbb{R}$
- $\delta_{1:K} = (\delta_1, \dots, \delta_k)$ : subgroup-specific “bias” of EC data on logit scale
- $\frac{\partial v}{\partial z}$ : Jacobian matrix of some vector  $v \in \mathbb{R}^m$  with respect to some  $z \in \mathbb{R}^w$
- $E(\cdot)$ : expectation
- $(e)$ : superscript indicating EC data set
- $\hat{G}_k$ : bootstrap distribution of  $\hat{\theta}_k^h$
- $g$ : (logit) link function
- $h$ : superscript to indicate harmonized estimator
- $\eta_{1:K} = (\eta_1, \dots, \eta_K)$ : subgroup-specific treatment effect on logit scale
- $\hat{\eta}_{1:K}^{(r+e)}$ : MLE of  $\eta_{1:K}$  under (29) (pooled logistic regression at beginning of 3.2)
- $\hat{\eta}_{1:K}^{(r)}$ : MLE of  $\eta_{1:K}$  under version of logistic model (29) using RCT data only
- $\eta_{1:K}^\circ$ : limit in probability of  $\hat{\eta}_{1:K}^{(r+e)}$
- $i$ : subscript for person  $i$  (in either RCT or EC data)

- $I_K$ :  $K \times K$  identity matrix
- $k = 1, \dots, K$ : subgroup index
- $\kappa$ : real constant used in the equation  $\Sigma\pi = \kappa b$
- $\ell = 1, \dots, K - 1$ : subgroup index used to define invariance to merging subgroups
- $\lambda \in [0, \infty]$ : parameter used to define the harmonized estimator
- $M_1$ :  $n^{(r+e)} \times (2K + d)$  design matrix for the pooled linear/logistic regression model (21)/(29), with columns corresponding to  $\mu_{1:K}$ ,  $\theta_{1:K}$ , and  $\beta$  (linear case) or  $\nu_{1:K}$ ,  $\eta_{1:K}$ , and  $\beta$  (logistic case)
- $M_2$ :  $n^{(r+e)} \times K$  additional design matrix columns corresponding to  $\gamma_{1:K}$  (linear case) or  $\delta_{1:K}$  (logistic case), i.e. for model(S3.8.1)/(32) the design matrix is  $\begin{bmatrix} M_1 & M_2 \end{bmatrix}$
- $M_0$ :  $n^{(r)} \times (2 + d)$  design matrix for the RCT-only primary analysis linear model (20)
- $m^{(A1)}$ : prior mean of  $(\mu, \theta)$  in Analyst 1's model
- $m^{(A2)}$ : prior mean of  $(\mu_{1:K}, \theta_{1:K})$  in Analyst 2's model
- $\mu$ : overall mean of  $Y$  in the RCT control group (when  $X = 0$  for models with covariates)
- $\mu_{1:K}$ : subgroup-specific means of  $Y$  in the RCT control group (when  $X = 0$  for models with covariates)
- $N$ : univariate normal distribution, e.g.  $Y \sim N(0, 1)$
- $N_k$ :  $k$ -variate normal distribution, e.g.  $(\mu, \theta) \sim N_2(m^{(A1)}, \tau^{(A1)})$
- $n_{k,t}^{(s)}$ : number of patients in subgroup  $k = 1, \dots, K$ , treatment arm  $t \in \{0, 1\}$  (control and treatment respectively), and data set  $s \in \{r, e, r + e\}$  (RCT, EC, and RCT + EC combined)
- $n_{k,\cdot}^{(s)}$ : number of patients in subgroup  $k$  and data set  $s$
- $n_{\cdot,t}^{(s)}$ : number of patients in treatment arm  $t$  in data set  $s$
- $n^{(s)}$ : total number of patients in data set  $s$
- $\nu_{1:K} = (\nu_1, \dots, \nu_K)$ : subgroup-specific control group “mean” parameter on the logit scale
- $\hat{\nu}_{1:K}^{(r+e)}$ : MLE of  $\nu_{1:K}$  under (29) (pooled logistic regression at beginning of 3.2)
- $\hat{\nu}_{1:K}^{(r)}$ : MLE of  $\nu_{1:K}$  under version of logistic model (29) but using RCT data only
- $\nu_{1:K}^\circ$ : limit in probability of  $\hat{\nu}_{1:K}^{(r+e)}$  in the logistic regression example (Section 3.2)
- $p(\cdot)$ : in some cases probability density/mass of a value of a random variable, in other cases the probability of an event (may take a superscript to indicate the distribution)
- $P = \begin{bmatrix} I_K - u\pi^\top & u \end{bmatrix}$ , in Proposition 3

- $\phi^2$ : residual variance of  $Y$  given subgroup (in model (6), and also given covariates in model(S3.8.1))
- $\pi = (\pi_1, \dots, \pi_K)$ : subgroup prevalences in RCT
- $\Pi = \text{diag}(\pi_k)$
- $\pi' = (\pi_1, \dots, \pi_{K-2}, \pi_{K-1} + \pi_K)$
- $q = \frac{n_{\cdot,0}^{(r)}}{n_{\cdot,0}^{(r)} + n_{\cdot,0}^{(e)}}$ : proportion of controls in the RCT (vs. RCT + EC combined)
- $Q = \text{diag}(Q_{k,k})$  and  $Q_{k,K} = \frac{n_{k,0}^{(r)}}{n_{k,0}^{(r)} + n_{k,0}^{(e)}}$ : subgroup-specific proportions of controls in RCT (vs. RCT + EC combined)
- $\bar{q} = \sum_{k=1}^K \pi_k Q_{k,k}$
- $(r)$ : superscript indicating RCT data set
- $r_1(\delta_{1:K})$ : remainder term in the Taylor expansion of  $\theta_{1:K}^o$
- $r_2(\delta_{1:K})$ : remainder term in the Taylor expansion of the limit in probability of  $\hat{\theta}_{1:K}^h$  in Section 3.2 (logistic regression example)
- $R$ : number of replicates in the bootstrap
- $\hat{\rho}(X_i^{(e)})$ : estimate of the “sampling” propensity score, i.e. the probability that a patient with covariates  $X_i^{(e)}$  would be in the RCT as opposed to EC
- $(s)$ : data set index, for  $s \in \{r, e, r + e\}$
- $S = \text{Var}\left(\hat{\theta}_{1:K}^{(r+e)}, \hat{\theta}^{(r)}\right)$
- $\sigma^2$ : residual variance of  $Y$  *not* conditioning on subgroups  $W_i$
- $\Sigma$ : fixed positive-definite  $K \times K$  matrix used to define  $\hat{\theta}^h$
- $\hat{\Sigma}$ : random (estimated) positive-definite  $K \times K$  matrix used to define  $\hat{\theta}^h$  in Sections 3.2 and 3.3
- $\Sigma'$ : fixed positive-definite  $(K-1) \times (K-1)$  matrix used to define  $\hat{\theta}^h$  in Section 2.5 (version of  $\Sigma$  used after subgroups  $K$  and  $K-1$  are merged)
- $\Sigma_{1:K}^{(A2)}$ : posterior variance of  $\theta_{1:K}$  in Analyst 2’s model in the cut distribution discussions (Section 2.3 and 2.4)
- $\Sigma_{\theta}^{(A1)}$ : posterior variance of  $\theta$  in Analyst 1’s model in the cut distribution discussions (Section 2.3 and 2.4)
- $\Sigma_{\theta}^{(A2)}$ : posterior variance of  $\theta$  in Analyst 2’s model in the cut distribution discussions (Section 2.3 and 2.4)
- $T_i^{(s)}$ : binary treatment indicator of patient  $i$  in data set  $s$ , taking values  $t \in \{0, 1\}$

- $\tau^{(A1)}$ : prior variance of  $(\mu, \theta)$  in Analyst 1's model in the cut distribution discussions (Sections 2.3 and 2.4)
- $\tau^{(A2)}$ : prior variance of  $(\mu_{1:K}, \theta_{1:K})$  in Analyst 1's model in the cut distribution discussions (Sections 2.3 and 2.4)
- $\theta$ : overall treatment effect in RCT population, not conditioning on subgroup
- $\theta_{1:K}$ : subgroup-specific treatment effects in RCT population
- $\hat{\theta}^{(r)}$ : estimator of  $\theta$  using only  $D^{(r)}$
- $\hat{\theta}_{1:K}^{(r+e)}$ : estimator of  $\theta_{1:K}$  using both  $D^{(r)}$  and  $D^{(e)}$
- $\hat{\theta}_{1:K}^h$ : harmonized estimator of  $\theta_{1:K}$
- $\hat{\theta}_{1:K}^{(r)}$ : estimator of  $\theta_{1:K}$  using only  $D^{(r)}$
- $\hat{\theta}_{1:K}^{ora}$ : oracle estimator of  $\theta_{1:K}$  (with  $\mu_{1:K}$  known)
- $\hat{\theta}_{1:K}^{(A2)}$ : posterior mean of  $\theta_{1:K}$  under Analyst 2's model in the cut distribution discussions (Section 2.3)
- $\hat{\theta}_{1:K}$ : generic estimator of  $\theta_{1:K}$  used in definition of invariance to merging subgroups
- $\theta'_{1:K-1}$ : subgroup-specific treatment effects in RCT population after the original groups  $K$  and  $K - 1$  have been merged
- $\hat{\theta}'_{1:K-1}$ : generic estimator of  $\theta'_{1:K-1}$  used in definition of invariance to merging subgroups
- $\hat{\theta}'_{1:K-1}^{(r+e)}$ : estimator of  $\theta'_{1:K-1}$  using  $D^{(r)}$  and  $D^{(e)}$
- $\hat{\theta}'_{1:K-1}^h$ : harmonized estimator of  $\theta'_{1:K-1}$
- $\theta_{1:K}^\circ$ : limit in probability of  $\hat{\theta}_{1:K}^{(r+e)}$  in the logistic regression example (Section 3.2)
- $u = c \frac{\lambda}{\lambda+c} \Sigma \pi$
- $v$ : argument of the objective function defining  $\hat{\theta}_{1:K}^h$  in equation (1)
- $V^h$ : variance of  $\hat{\theta}_{1:K}^h$  in the simple example (Section 2.2)
- $V^{(cut)}$ : variance of the cut distribution in Sections 2.3 and 2.4
- $Var(U)$ : variance-covariance matrix of a random vector  $U$
- $W_i^{(s)}$ : subgroup membership for patient  $i$  in data set  $s$ , taking values in  $\{1, \dots, K\}$
- $w_{ik}^{(r)}$ : sampling propensity score weight for patient  $i$  in subgroup  $k$  in the RCT, proportional to 1
- $w_{ik}^{(e)}$ : sampling propensity score weight for patient  $i$  in subgroup  $k$  in the EC, depends on covariates and subgroup

- $X_i^{(s)}$ :  $d$ -dimensional pre-treatment covariate vector for patient  $i$  in data set  $s$  (excluding subgroup membership)
- $Y_i^{(s)}$ : (scalar) outcome for patient  $i$  in data set  $s$
- $Z$ : matrix describing the linear invariance relation  $\hat{\theta}'_{1:K-1} = Z\hat{\theta}_{1:K}$
- $1_{m \times w}, 0_{m \times w}$ :  $m \times w$  matrix in which all entries are 1 or 0 respectively
- $\begin{bmatrix} A_1 & A_2 \\ A_3 & A_4 \end{bmatrix}, \begin{bmatrix} A_1 & A_2 \end{bmatrix}, \begin{bmatrix} A_1 \\ A_3 \end{bmatrix}$ : generic notation for block matrices, where  $A_1, A_2, A_3, A_4$  are conformable matrices
- $\|\cdot\|_1$ :  $L^1$  norm of a vector

## S2 Additional material for Section 2

### S2.1 Proofs for Section 2.1 (derivation of the harmonized estimator)

The harmonized estimator is defined as

$$\hat{\theta}_{1:K}^h = \arg \min_v \left[ \left( v - \hat{\theta}_{1:K}^{(r+e)} \right)^\top \Sigma^{-1} \left( v - \hat{\theta}_{1:K}^{(r+e)} \right) + \lambda \left( \pi^\top v - \hat{\theta}^{(r)} \right)^2 \right]. \quad (\text{S2.1.1})$$

An explicit formula for the harmonized estimator can be found by taking the derivative of the objective function in (S2.1.1) with respect to  $v$ , setting it equal to zero, and solving. Writing  $h(v)$  for the objective function and  $0_K$  for a length- $K$  vector of zeros, at the minimizer  $\hat{\theta}_{1:K}^h$  we have

$$\begin{aligned} 0_K &= \nabla h(\hat{\theta}_{1:K}^h) \\ 0_K &= 2\Sigma^{-1} \left( \hat{\theta}_{1:K}^h - \hat{\theta}_{1:K}^{(r+e)} \right) + 2\lambda \left( \pi^\top \hat{\theta}_{1:K}^h - \hat{\theta}^{(r)} \right) \pi \\ 0_K &= \Sigma^{-1} \hat{\theta}_{1:K}^h - \Sigma^{-1} \hat{\theta}_{1:K}^{(r+e)} + \lambda \pi^\top \hat{\theta}_{1:K}^h \pi - \lambda \hat{\theta}^{(r)} \pi \\ \Sigma^{-1} \hat{\theta}_{1:K}^h + \lambda \pi^\top \hat{\theta}_{1:K}^h \pi &= \Sigma^{-1} \hat{\theta}_{1:K}^{(r+e)} + \lambda \hat{\theta}^{(r)} \pi \\ \Sigma^{-1} \hat{\theta}_{1:K}^h + \lambda \pi \left( \pi^\top \hat{\theta}_{1:K}^h \right) &= \Sigma^{-1} \hat{\theta}_{1:K}^{(r+e)} + \lambda \hat{\theta}^{(r)} \pi \\ \Sigma^{-1} \hat{\theta}_{1:K}^h + \left( \lambda \pi \pi^\top \right) \hat{\theta}_{1:K}^h &= \Sigma^{-1} \hat{\theta}_{1:K}^{(r+e)} + \lambda \hat{\theta}^{(r)} \pi \\ \left( \Sigma^{-1} + \lambda \pi \pi^\top \right) \hat{\theta}_{1:K}^h &= \Sigma^{-1} \hat{\theta}_{1:K}^{(r+e)} + \lambda \hat{\theta}^{(r)} \pi \\ \hat{\theta}_{1:K}^h &= \left( \Sigma^{-1} + \lambda \pi \pi^\top \right)^{-1} \left[ \Sigma^{-1} \hat{\theta}_{1:K}^{(r+e)} + \lambda \hat{\theta}^{(r)} \pi \right]. \end{aligned}$$

Since  $\pi^\top 1_K = 1$ , where  $1_K$  is a length- $K$  vector of ones, this estimator may also be written

$$\hat{\theta}_{1:K}^h = \left( \Sigma^{-1} + \lambda \pi \pi^\top \right)^{-1} \left[ \Sigma^{-1} \hat{\theta}_{1:K}^{(r+e)} + \lambda \pi \pi^\top \left( \hat{\theta}^{(r)} 1_K \right) \right]. \quad (\text{S2.1.2})$$

This corresponds to equation (4) in the text. The matrix inverse can also be written as

$$\left( \Sigma^{-1} + \lambda \pi \pi^\top \right)^{-1} = \Sigma - \frac{\lambda}{1 + \lambda \pi^\top \Sigma \pi} \Sigma \pi \pi^\top \Sigma$$

by the Sherman-Morrison inversion formula. Using this substitution we have

$$\begin{aligned}
\hat{\theta}_{1:K}^h &= \left( \Sigma - \frac{\lambda}{1 + \lambda \pi^\top \Sigma \pi} \Sigma \pi \pi^\top \Sigma \right) \left[ \Sigma^{-1} \hat{\theta}_{1:K}^{(r+e)} + \lambda \pi \pi^\top \left( \hat{\theta}^{(r)} \mathbf{1}_K \right) \right] \\
&= \hat{\theta}_{1:K}^{(r+e)} - \frac{\lambda}{1 + \lambda \pi^\top \Sigma \pi} \left( \pi^\top \hat{\theta}_{1:K}^{(r+e)} \right) \Sigma \pi + \lambda \hat{\theta}^{(r)} \Sigma \pi - \lambda \pi^\top \Sigma \pi \frac{\lambda}{1 + \lambda \pi^\top \Sigma \pi} \hat{\theta}^{(r)} \Sigma \pi \\
&= \hat{\theta}_{1:K}^{(r+e)} + \left[ \lambda - \lambda \pi^\top \Sigma \pi \frac{\lambda}{1 + \lambda \pi^\top \Sigma \pi} \right] \hat{\theta}^{(r)} \Sigma \pi - \frac{\lambda}{1 + \lambda \pi^\top \Sigma \pi} \left( \pi^\top \hat{\theta}_{1:K}^{(r+e)} \right) \Sigma \pi \\
&= \hat{\theta}_{1:K}^{(r+e)} + \left[ \frac{\lambda (1 + \lambda \pi^\top \Sigma \pi)}{1 + \lambda \pi^\top \Sigma \pi} - \frac{\lambda (\lambda \pi^\top \Sigma \pi)}{1 + \lambda \pi^\top \Sigma \pi} \right] \hat{\theta}^{(r)} \Sigma \pi - \frac{\lambda}{1 + \lambda \pi^\top \Sigma \pi} \left( \pi^\top \hat{\theta}_{1:K}^{(r+e)} \right) \Sigma \pi \\
&= \hat{\theta}_{1:K}^{(r+e)} + \frac{\lambda}{1 + \lambda \pi^\top \Sigma \pi} \hat{\theta}^{(r)} \Sigma \pi - \frac{\lambda}{1 + \lambda \pi^\top \Sigma \pi} \left( \pi^\top \hat{\theta}_{1:K}^{(r+e)} \right) \Sigma \pi \\
&\boxed{\hat{\theta}_{1:K}^h = \hat{\theta}_{1:K}^{(r+e)} + c \frac{\lambda}{\lambda + c} \left( \hat{\theta}^{(r)} - \pi^\top \hat{\theta}_{1:K}^{(r+e)} \right) \Sigma \pi,}
\end{aligned}$$

where  $c = (\pi^\top \Sigma \pi)^{-1}$ . This corresponds to equation (5) in the text.

## S2.2 Proofs for Section 2.2 (Proposition 1 and its generalization)

Here we first prove equation (10), which gives the bias and variance of  $\hat{\theta}_{1:K}^h$  in a more general setting. Then equations (7) and (8) in Proposition 1 are a special case.

### S2.2.1 Generalization

Equation (10) in the text gives the bias and variance of  $\hat{\theta}_{1:K}^h$  when:

1. The outcome is sampled according to the model

$$\begin{aligned}
Y_i^{(r)} | W_i^{(r)}, T_i^{(r)} &\stackrel{iid}{\sim} N \left( \mu_{W_i^{(r)}} + \theta_{W_i^{(r)}} T_i^{(r)}, \phi^2 \right), \text{ and} \\
Y_i^{(e)} | W_i^{(e)} &\stackrel{iid}{\sim} N \left( \mu_{W_i^{(e)}} + \gamma_{W_i^{(e)}}, \phi^2 \right).
\end{aligned} \tag{6}$$

2. The RCT trial design satisfies the condition

$$\pi_k = \frac{n_{k,\cdot}^{(r)}}{n^{(r)}} = \frac{n_{k,0}^{(r)}}{n_{\cdot,0}^{(r)}} = \frac{n_{k,1}^{(r)}}{n_{\cdot,1}^{(r)}}. \tag{S2.2.1}$$

This is satisfied when subgroups are recruited proportional to the true subpopulation sizes and randomization is blocked by subgroup (with the same randomization ratio in each subgroup).

3. The harmonized estimator  $\hat{\theta}^h$  uses as inputs

$$\hat{\theta}^{(r)} = \bar{Y}_{\cdot,1}^{(r)} - \bar{Y}_{\cdot,0}^{(r)}$$

and

$$\hat{\theta}_k^{(r+e)} = \bar{Y}_{k,1}^{(r)} - \bar{Y}_{k,0}^{(r+e)}.$$

**Claim S1.** *In this setting, we have*

$$\begin{aligned}
B^h &= \left( I_K - c \frac{\lambda}{\lambda + c} \Sigma \pi \pi^\top \right) (I_K - Q) \gamma_{1:K}, \text{ and} \\
V^h &= \phi^2 \left[ \frac{1}{n_{\cdot,1}^{(r)}} I_K + \frac{1}{n_{\cdot,0}^{(r)}} Q \right] \Pi^{-1} + \left( c \frac{\lambda}{\lambda + c} \right)^2 (1 - \bar{q}) \frac{1}{n_{\cdot,0}^{(r)}} \phi^2 \Sigma \pi \pi^\top \Sigma,
\end{aligned} \tag{10}$$

where  $B^h = \text{Bias}(\hat{\theta}_{1:K}^h, \theta_{1:K})$ ,  $V^h = \text{Var}(\hat{\theta}_{1:K}^h)$ , and  $Q$  is a diagonal  $K \times K$  matrix with elements  $Q_{k,k} = \frac{n_{k,0}^{(r)}}{n_{k,0}^{(r+e)}}$  (the fraction of subgroup  $k$ 's control patients in the RCT as opposed to the RCT and EC combined).

*Proof.* For the bias, first note that we may write  $\hat{\theta}_{1:K}^{(r+e)}$  as

$$\hat{\theta}_{1:K}^{(r+e)} = \bar{Y}_{1:K,1}^{(r)} - \bar{Y}_{1:K,0}^{(r+e)} = \bar{Y}_{1:K,1}^{(r)} - \left[ Q \bar{Y}_{1:K,0}^{(r)} + (I_K - Q) \bar{Y}_{1:K,\cdot}^{(e)} \right],$$

where  $\bar{Y}_{1:K,t}^{(s)}$  is a length- $K$  vector with components  $\bar{Y}_{k,t}^{(s)}$  for  $s \in \{r, e, r+e\}$  and  $t \in \{0, 1, \cdot\}$ . It thus has expectation

$$\begin{aligned} E(\hat{\theta}_{1:K}^{(r+e)}) &= E(\bar{Y}_{1:K,1}^{(r)}) - E(\bar{Y}_{1:K,0}^{(r+e)}) \\ &= \mu_{1:K} + \theta_{1:K} - E\left[Q \bar{Y}_{1:K,0}^{(r)} + (I_K - Q) \bar{Y}_{1:K,\cdot}^{(e)}\right] \\ &= \mu_{1:K} + \theta_{1:K} - [Q \mu_{1:K} + (I_K - Q)(\mu_{1:K} + \gamma_{1:K})] \\ &= \theta_{1:K} - (I_K - Q)\gamma_{1:K}. \end{aligned}$$

So

$$\begin{aligned} B^h &= E(\hat{\theta}_{1:K}^h) - \theta_{1:K} \\ &= \left(\Sigma + \lambda \pi \pi^\top\right)^{-1} \left[ \Sigma^{-1} E(\hat{\theta}_{1:K}^{(r+e)}) + \lambda \pi E(\hat{\theta}^{(r)}) \right] - \theta_{1:K} \\ &= \left(\Sigma + \lambda \pi \pi^\top\right)^{-1} \left[ \Sigma^{-1} \theta_{1:K} - \Sigma^{-1} (I_K - Q) \gamma_{1:K} + \lambda \pi \pi^\top \theta_{1:K} \right] - \theta_{1:K} \\ &= - \left(\Sigma + \lambda \pi \pi^\top\right)^{-1} \left[ \Sigma^{-1} (I_K - Q) \gamma_{1:K} \right] \\ &= - \left( \Sigma - c \frac{\lambda}{\lambda + c} \Sigma \pi \pi^\top \Sigma \right) \Sigma^{-1} (I_K - Q) \gamma_{1:K} \\ &= \boxed{B^h = - \left( I_K - c \frac{\lambda}{\lambda + c} \Sigma \pi \pi^\top \right) (I_K - Q) \gamma_{1:K}.} \end{aligned}$$

To find  $V^h$ , we take the variance of the expression

$$\hat{\theta}_{1:K}^h = \hat{\theta}_{1:K}^{(r+e)} + c \frac{\lambda}{\lambda + c} (\hat{\theta}^{(r)} - \bar{\theta}^{(r+e)}) \Sigma \pi,$$

where recall that we defined  $\bar{\theta}^{(r+e)} = \pi^\top \hat{\theta}_{1:K}^{(r+e)}$ . This requires computing

- (i)  $\text{Var}(\hat{\theta}_{1:K}^{(r+e)})$ ,
- (ii)  $\text{Var}(\hat{\theta}^{(r)} - \bar{\theta}^{(r+e)})$ , and
- (iii)  $\text{Cov}(\hat{\theta}_{1:K}^{(r+e)}, (\hat{\theta}^{(r)} - \bar{\theta}^{(r+e)}) \Sigma \pi)$ .

### Computing (i) $\text{Var}(\hat{\theta}_{1:K}^{(r+e)})$

Under model (6), we have

$$\text{Var}(\hat{\theta}_k^{(r+e)}) = \left[ \frac{1}{n_{k,1}^{(r)}} + \frac{1}{n_{k,0}^{(r+e)}} \right] \phi^2 = \left[ \frac{1}{n_{k,1}^{(r)}} + Q_{k,k} \frac{1}{n_{k,0}^{(r)}} \right] \phi^2 = \left[ \frac{1}{n_{\cdot,1}^{(r)}} + Q_{k,k} \frac{1}{n_{\cdot,0}^{(r)}} \right] \frac{1}{\pi_k} \phi^2,$$

where by definition  $Q_{k,k} = \frac{n_{\cdot,0}^{(r)}}{n_{k,0}^{(r+e)}}$ . Model (6) implies that  $\hat{\theta}_k^{(r+e)}$  is independent of  $\hat{\theta}_j^{(r+e)}$  for  $k \neq j$ , so

$$\text{Var} \left( \hat{\theta}_{1:K}^{(r+e)} \right) = \phi^2 \left[ \frac{1}{n_{\cdot,1}^{(r)}} I_K + \frac{1}{n_{\cdot,0}^{(r)}} Q \right] \Pi^{-1}, \quad (\text{S2.2.2})$$

where  $\Pi$  is a diagonal matrix with elements  $\Pi_{k,k} = \pi_k$ .

### Computing (ii) $\text{Var} \left( \hat{\theta}^{(r)} - \bar{\theta}^{(r+e)} \right)$

Note that  $\text{Var} \left( \hat{\theta}^{(r)} - \bar{\theta}^{(r+e)} \right) = \text{Var} \left( \hat{\theta}^{(r)} \right) + \text{Var} \left( \bar{\theta}^{(r+e)} \right) - 2\text{Cov} \left( \hat{\theta}^{(r)}, \bar{\theta}^{(r+e)} \right)$ , and  $\text{Var} \left( \hat{\theta}^{(r)} \right) = \left[ \frac{1}{n_{\cdot,1}^{(r)}} + \frac{1}{n_{\cdot,0}^{(r)}} \right] \phi^2$ , by model (6). From above we also have

$$\text{Var} \left( \bar{\theta}^{(r+e)} \right) = \pi^\top \text{Var} \left( \hat{\theta}_{1:K}^{(r+e)} \right) \pi = \sum_{k=1}^K \pi_k^2 \left[ \frac{1}{n_{\cdot,1}^{(r)}} + Q_{k,k} \frac{1}{n_{\cdot,0}^{(r)}} \right] \frac{1}{\pi_k} \phi^2 = \left[ \frac{1}{n_{\cdot,1}^{(r)}} + \bar{q} \frac{1}{n_{\cdot,0}^{(r)}} \right] \phi^2, \quad (\text{S2.2.3})$$

where we define  $\bar{q} = \sum_{k=1}^K \pi_k Q_{k,k}$ . Lastly, note that

$$\text{Cov} \left( \hat{\theta}^{(r)}, \bar{\theta}^{(r+e)} \right) = \sum_{k=1}^K \pi_k \text{Cov} \left( \hat{\theta}^{(r)}, \hat{\theta}_k^{(r+e)} \right)$$

and by model (6)

$$\begin{aligned} \text{Cov} \left( \hat{\theta}^{(r)}, \hat{\theta}_k^{(r+e)} \right) &= \text{Cov} \left( \bar{Y}_{\cdot,1}^{(r)} - \bar{Y}_{\cdot,0}^{(r)}, \bar{Y}_{k,1}^{(r)} - Q_{k,k} \bar{Y}_{k,0}^{(r)} - (1 - Q_{k,k}) \bar{Y}_{k,0}^{(e)} \right) \\ &= \text{Cov} \left( \bar{Y}_{\cdot,1}^{(r)}, \bar{Y}_{k,1}^{(r)} \right) + \text{Cov} \left( \bar{Y}_{\cdot,0}^{(r)}, Q_{k,k} \bar{Y}_{k,0}^{(r)} \right) \\ &= \text{Cov} \left( \pi_k \bar{Y}_{k,1}^{(r)}, \bar{Y}_{k,1}^{(r)} \right) + \text{Cov} \left( \pi_k \bar{Y}_{k,0}^{(r)}, Q_{k,k} \bar{Y}_{k,0}^{(r)} \right) \\ &= \pi_k \text{Var} \left( \bar{Y}_{k,1}^{(r)} \right) + \pi_k Q_{k,k} \text{Var} \left( \bar{Y}_{k,0}^{(r)} \right) \\ &= \pi_k \frac{1}{n_{k,1}^{(r)}} \phi^2 + \pi_k Q_{k,k} \frac{1}{n_{k,0}^{(r)}} \phi^2 \\ \text{Cov} \left( \hat{\theta}^{(r)}, \hat{\theta}_k^{(r+e)} \right) &= \left[ \frac{1}{n_{\cdot,1}^{(r)}} + Q_{k,k} \frac{1}{n_{\cdot,0}^{(r)}} \right] \phi^2. \end{aligned}$$

So we have

$$\text{Cov} \left( \hat{\theta}^{(r)}, \bar{\theta}^{(r+e)} \right) = \sum_{k=1}^K \pi_k \text{Cov} \left( \hat{\theta}^{(r)}, \hat{\theta}_k^{(r+e)} \right) = \sum_{k=1}^K \pi_k \left[ \frac{1}{n_{\cdot,1}^{(r)}} + Q_{k,k} \frac{1}{n_{\cdot,0}^{(r)}} \right] \phi^2 = \text{Var} \left( \pi^\top \hat{\theta}_{1:K}^{(r+e)} \right).$$

Hence

$$\text{Var} \left( \hat{\theta}^{(r)} - \bar{\theta}^{(r+e)} \right) = \text{Var} \left( \hat{\theta}^{(r)} \right) - \text{Var} \left( \bar{\theta}^{(r+e)} \right) = (1 - \bar{q}) \frac{1}{n_{\cdot,0}^{(r)}} \phi^2. \quad (\text{S2.2.4})$$

### Computing (iii) $\text{Cov} \left( \hat{\theta}_{1:K}^{(r+e)}, \left( \hat{\theta}^{(r)} - \bar{\theta}^{(r+e)} \right) \Sigma \pi \right)$

First, define  $\mu_{1:K}^{(r+e)} = E \left( \hat{\theta}_{1:K}^{(r+e)} \right)$  and  $\mu^{(dif)} = E \left( \hat{\theta}^{(r)} - \bar{\theta}^{(r+e)} \right)$ . Then we compute the matrix

$$\begin{aligned} \text{Cov} \left( \hat{\theta}_{1:K}^{(r+e)}, \left( \hat{\theta}^{(r)} - \bar{\theta}^{(r+e)} \right) \Sigma \pi \right) &= E \left[ \left( \hat{\theta}_{1:K}^{(r+e)} - \mu_{1:K}^{(r+e)} \right) \left( \left[ \hat{\theta}^{(r)} - \bar{\theta}^{(r+e)} \right] \Sigma \pi - \mu^{(dif)} \Sigma \pi \right)^\top \right] \\ &= \text{Cov} \left( \hat{\theta}_{1:K}^{(r+e)}, \hat{\theta}^{(r)} - \bar{\theta}^{(r+e)} \right) \pi^\top \Sigma. \end{aligned}$$

Here  $Cov\left(\hat{\theta}_{1:K}^{(r+e)}, \hat{\theta}^{(r)} - \bar{\theta}^{(r+e)}\right)$  is a column vector with the  $k$ -th element equal to

$$Cov\left(\hat{\theta}_k^{(r+e)}, \hat{\theta}^{(r)} - \bar{\theta}^{(r+e)}\right) = Cov\left(\hat{\theta}_k^{(r+e)}, \hat{\theta}^{(r)}\right) - Cov\left(\hat{\theta}_k^{(r+e)}, \bar{\theta}^{(r+e)}\right).$$

It is easy to see that  $Cov\left(\hat{\theta}_k^{(r+e)}, \hat{\theta}^{(r)}\right) = \pi_k Var\left(\hat{\theta}_k^{(r+e)}\right) = \left[\frac{1}{n_{\cdot,1}^{(r)}} + Q_{k,k} \frac{1}{n_{\cdot,0}^{(r)}}\right] \phi^2$ . Since  $Cov\left(\hat{\theta}_k^{(r+e)}, \bar{\theta}^{(r+e)}\right) = \left[\frac{1}{n_{\cdot,1}^{(r)}} + Q_{k,k} \frac{1}{n_{\cdot,0}^{(r)}}\right] \phi^2$  as well, and  $Cov\left(\hat{\theta}_k^{(r+e)}, \hat{\theta}^{(r)}\right) = 0$ , we thus have

$$Cov\left(\hat{\theta}_{1:K}^{(r+e)}, \left(\hat{\theta}^{(r)} - \bar{\theta}^{(r+e)}\right) \Sigma \pi\right) = 0_{K \times K}. \quad (\text{S2.2.5})$$

### Computing $Var\left(\hat{\theta}_{1:K}^h\right)$

We are finally ready to find  $Var\left(\hat{\theta}_{1:K}^h\right)$ . In particular, using (S2.2.2), (S2.2.4), and (S2.2.5) we have

$$Var\left(\hat{\theta}_{1:K}^h\right) = Var\left(\hat{\theta}_{1:K}^{(r+e)}\right) + \left(c \frac{\lambda}{\lambda + c}\right)^2 Var\left(\hat{\theta}^{(r)} - \pi^\top \hat{\theta}_{1:K}^{(r+e)}\right) \Sigma \pi \pi^\top \Sigma$$

$$Var\left(\hat{\theta}_{1:K}^h\right) = \phi^2 \left[ \frac{1}{n_{\cdot,1}^{(r)}} I_K + \frac{1}{n_{\cdot,0}^{(r)}} Q \right] \Pi^{-1} + \left(c \frac{\lambda}{\lambda + c}\right)^2 (1 - \bar{q}) \frac{1}{n_{\cdot,0}^{(r)}} \phi^2 \Sigma \pi \pi^\top \Sigma.$$

□

**Remark.** We note that this derivation of equation (10) uses the mean and covariance structure of model (6), but not its normality.

### S2.2.2 Proposition 1 (special case)

Proposition 1 assumes model (6) and the design condition (S2.2.1) just like equation (10) does, but it also makes the further design assumptions that:

1. randomization was balanced between treatment and control, i.e.

$$n_{\cdot,1}^{(r)} = n_{\cdot,0}^{(r)}, \quad (\text{S2.2.6})$$

2. subgroup proportions in the RCT are equal, i.e.

$$\pi = (1/K, \dots, 1/K), \quad (\text{S2.2.7})$$

3. and the EC has the same subgroup proportions as the RCT, i.e.

$$\frac{n_{k,\cdot}^{(e)}}{n^{(e)}} = \pi_k \quad \forall k = 1, \dots, K. \quad (\text{S2.2.8})$$

We use the notation  $1_{K \times K}$  to denote a  $K \times K$  matrix of 1's.

**Proposition 1.** Assume model (6) and design conditions (S2.2.1) and (S2.2.6)-(S2.2.8). If  $\Sigma^{-1} = I_K$ , then  $\hat{\theta}_{1:K}^h \sim N\left(\theta_{1:K} + B^h, V^h\right)$ , where the bias vector  $B^h$  is

$$B^h = -(1 - q) \left( I_K - \frac{1}{K} \frac{\lambda}{\lambda + K} 1_{K \times K} \right) \gamma_{1:K}$$

and the variance-covariance matrix is

$$V^h = K \frac{1}{n_{\cdot,0}^{(r)}} (1 + q) \phi^2 I_K + \left( \frac{\lambda}{\lambda + K} \right)^2 (1 - q) \frac{1}{n_{\cdot,0}^{(r)}} \phi^2 1_{K \times K}.$$

*Proof.*  $\hat{\theta}_{1:K}^h$  is normally distributed because it is a linear transformation (see (S2.1.2) and the definitions of  $\hat{\theta}_{1:K}^{(r+e)}$  and  $\hat{\theta}^{(r)}$  in this case) of normally distributed data under model (6).

In this simplified setting we have  $\Sigma = I_K$ ,  $c = (\pi^\top \pi)^{-1} = K$ ,  $\pi \pi^\top = \frac{1}{K^2} 1_{K \times K}$ ,  $Q_{k,k} = q = \frac{n_{\cdot,0}^{(r)}}{n_{\cdot,0}^{(r+e)}}$  for all  $k$ , and  $\Pi^{-1} = K I_K$ . Plugging these values in to (6), the bias becomes

$$B^h = - \left( I_K - c \frac{\lambda}{\lambda + c} \Sigma \pi \pi^\top \right) (I_K - Q) \gamma_{1:K} = -(1 - q) \left( I_K - \frac{1}{K} \frac{\lambda}{\lambda + K} 1_{K \times K} \right) \gamma_{1:K}$$

and the variance becomes

$$\begin{aligned} V^h &= \phi^2 \left[ \frac{1}{n_{\cdot,1}^{(r)}} I_K + \frac{1}{n_{\cdot,0}^{(r)}} Q \right] \Pi^{-1} + \left( c \frac{\lambda}{\lambda + c} \right)^2 (1 - \bar{q}) \frac{1}{n_{\cdot,0}^{(r)}} \phi^2 \Sigma \pi \pi^\top \Sigma \\ &= K \frac{1}{n_{\cdot,0}^{(r)}} (1 + q) \phi^2 I_K + \left( \frac{\lambda}{\lambda + K} \right)^2 (1 - q) \frac{1}{n_{\cdot,0}^{(r)}} \phi^2 1_{K \times K} \end{aligned}$$

since  $n_{\cdot,0}^{(r)} = n_{\cdot,1}^{(r)}$  by (S2.2.6). □

### S2.3 Replication of Figure 1 by simulation

We simulated data under exactly the same setting as Figure 1, with 2,000 replicates per scenario. As shown in Figure S1 the results are identical up to Monte Carlo error.

### S2.4 Proofs for Section 2.3 (Bayesian interpretation)

To review key notation, recall that Analyst 1 uses the following model for her primary analysis:

$$\text{Likelihood:} \quad Y_i^{(r)} | T_i^{(r)}, \mu, \theta \stackrel{\text{ind.}}{\sim} N \left( \mu + \theta T_i^{(r)}, \sigma^2 \right)$$

$$\text{Prior:} \quad (\mu, \theta) \sim N_2(m^{(A1)}, \tau^{(A1)})$$

$$\text{Posterior for } \theta: \quad \theta | Y^{(r)}, T^{(r)} \sim N \left( \theta^{(A1)}, \Sigma_\theta^{(A1)} \right).$$

And Analyst 2 uses the following model for his subgroup analysis:

$$\text{Likelihood:} \quad Y_i^{(r)} | T_i^{(r)}, W_i^{(r)}, \mu_{1:K}, \theta_{1:K} \stackrel{\text{ind.}}{\sim} N \left( \mu_{W_i^{(r)}} + \theta_{W_i^{(r)}} T_i^{(r)}, \phi^2 \right)$$

$$Y_j^{(e)} | W_j, \mu_{1:K} \stackrel{\text{ind.}}{\sim} N \left( \mu_{W_j^{(e)}}, \phi^2 \right)$$

$$\text{Prior:} \quad (\mu_{1:K}, \theta_{1:K}) \sim N_{2K} \left( m^{(A2)}, \tau^{(A2)} \right)$$

$$\text{Posterior for } \theta_{1:K}: \quad \theta_{1:K} | D^{(r)}, D^{(e)} \sim N_K \left( \theta_{1:K}^{(A2)}, \Sigma_{1:K}^{(A2)} \right)$$

$$\text{Posterior for } \theta: \quad \theta | D^{(r)}, D^{(e)} \sim N \left( \bar{\theta}^{(A2)}, \Sigma_\theta^{(A2)} \right).$$

Analyst 2's marginal posterior for  $\theta_{1:K}$  induces the posterior for  $\theta$  given the fixed  $\pi$ , with mean  $\bar{\theta}^{(A1)} = \pi^\top \theta_{1:K}^{(A2)}$  and variance  $\Sigma_\theta^{(A2)} = \pi^\top \Sigma_{1:K}^{(A2)} \pi$ .

The cut distribution combines these two models via the following joint distribution on  $(\theta_{1:K}, \theta)$ :

$$p^{\text{cut}} \left( \theta_{1:K}, \theta | D^{(r)}, D^{(e)} \right) = p^{(A2)} \left( \theta_{1:K} | \theta, D^{(r)}, D^{(e)} \right) \cdot p^{(A1)} \left( \theta | Y^{(r)}, T^{(r)} \right),$$

where the first factor is Analyst 2's conditional posterior for  $\theta_{1:K}$  given  $\theta$ , and the second factor is Analyst 1's posterior for  $\theta$ .

**A** Performance of four estimators in Scenarios 1, 2, and 3 (by simulation)

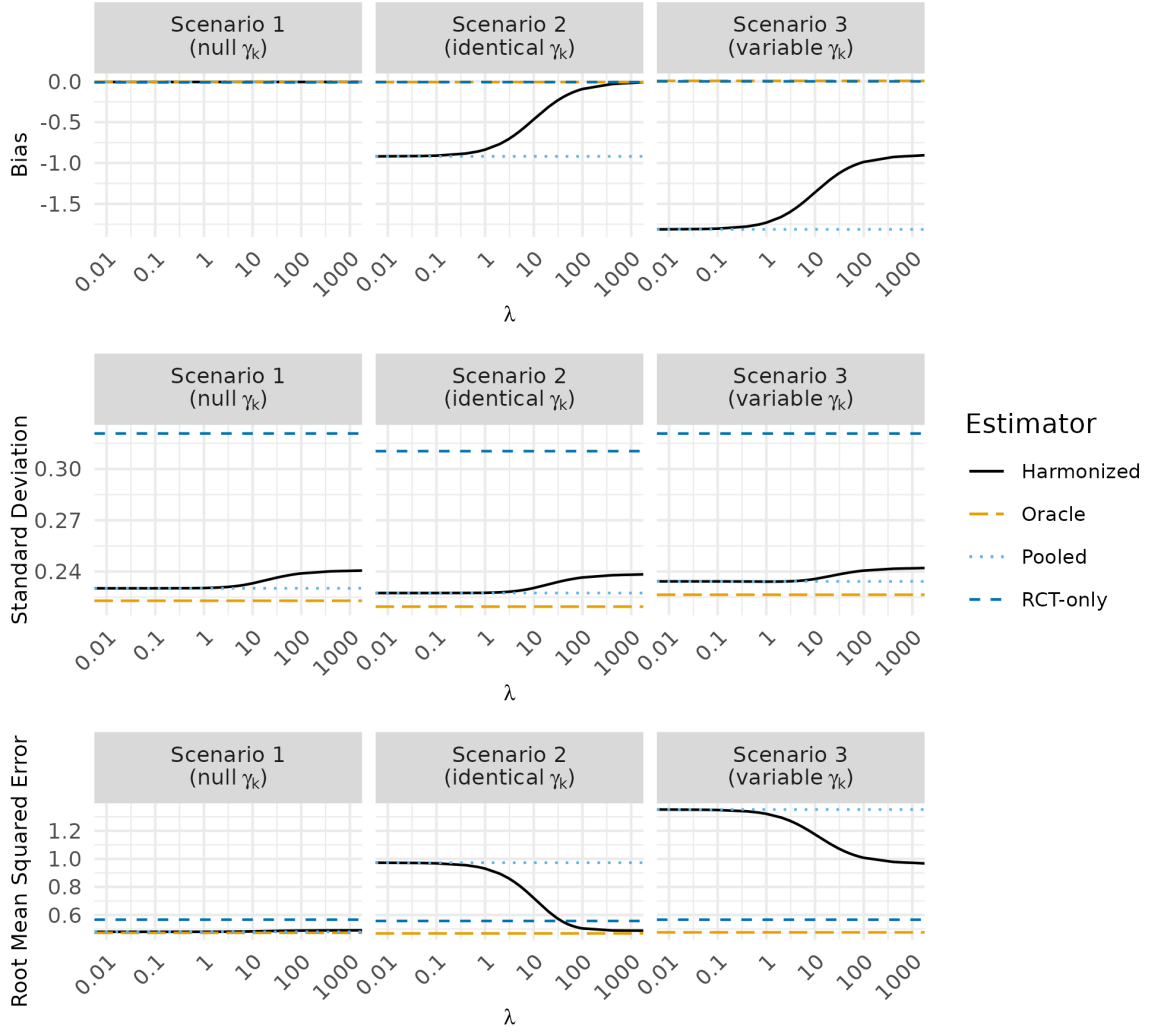

**B** Comparison of the four estimators in Scenario 3 (by simulation)

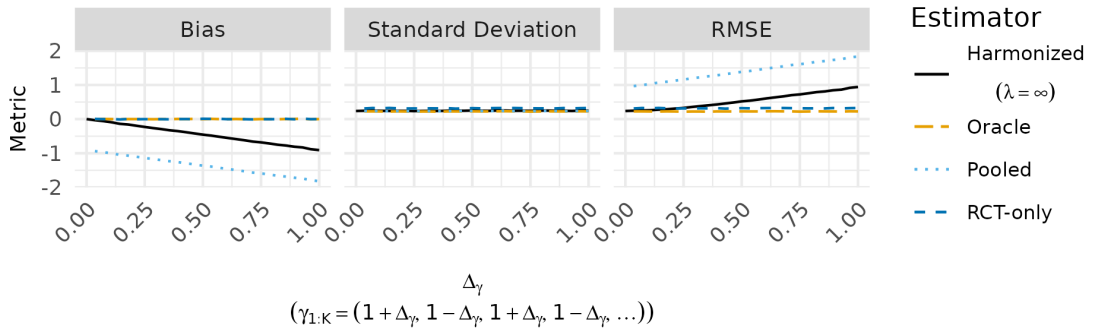

Figure S1: (A) Performance summaries of the harmonized estimator (see Proposition 1) and other estimators (analogous analytic results) for subgroup  $k = 1$ , computed by simulation of 2,000 replicated data sets per scenario. The  $\lambda$  value used to define the harmonized estimator varies on the x-axis. We illustrate the bias, standard deviation, and the root mean squared error (RMSE) of the estimator as a function of  $\lambda$ . The scenarios have different  $\gamma_{1:K}$  values:  $0_{K \times 1}$  (Scenario 1), constant across subgroups (Scenario 2), or varying across subgroups, with  $\gamma_{1:K} = (1 + \Delta_\gamma, 1 - \Delta_\gamma, 1 + \Delta_\gamma, 1 - \Delta_\gamma, \dots)$  and  $\Delta_\gamma = 1$  (Scenario 3). (B) The performance of the harmonized estimator (with  $\lambda = \infty$ ) for subgroup  $k = 1$  degrades when the subgroup-specific differences  $\gamma_{1:K}$  vary substantially across subgroups, i.e. as  $\Delta_\gamma$  grows.

### S2.4.1 Main result

In this section we find the marginal cut distribution for the subgroup effects  $\theta_{1:K}$ :

$$p^{\text{cut}}(\theta_{1:K}|D^{(r)}, D^{(e)}) = \int p^{(A2)}(\theta_{1:K}|\theta, D^{(r)}, D^{(e)}) \cdot p^{(A1)}(\theta|Y^{(r)}, T^{(r)}) d\theta.$$

The result is that under the cut distribution

$$\theta_{1:K} \sim N(\theta_{1:K}^{(\text{cut})}, \Sigma_{1:K}^{(\text{cut})}),$$

where

$$\begin{aligned} \theta_{1:K}^{(\text{cut})} &= \theta_{1:K}^{(A2)} + \frac{1}{\Sigma_{\theta}^{(A2)}} (\theta^{(A1)} - \bar{\theta}^{(A2)}) \Sigma_{1:K}^{(A2)} \pi, \quad \text{and} \\ \Sigma_{1:K}^{(\text{cut})} &= \Sigma_{1:K}^{(A2)} + \left( \frac{1}{\Sigma_{\theta}^{(A2)}} \right)^2 (\Sigma_{\theta}^{(A1)} - \Sigma_{\theta}^{(A2)}) \Sigma_{1:K}^{(A2)} \pi \pi^{\top} \Sigma_{1:K}^{(A2)}. \end{aligned}$$

### S2.4.2 Approach of the derivation

To derive this, it is important to keep in mind that the joint cut distribution  $p^{\text{cut}}(\theta_{1:K}, \theta|D^{(r)}, D^{(e)})$  is *not* fully normal or even continuous because of the deterministic relation  $\theta = \pi^{\top} \theta_{1:K}$  (since  $\pi$  is treated as known by Analyst 2). To avoid this issue, we find  $p^{\text{cut}}(\theta_{1:K}|D^{(r)}, D^{(e)})$  by first finding  $p^{\text{cut}}(\theta_{1:K-1}, \theta|D^{(r)}, D^{(e)})$  and then using the transformation

$$\theta_{1:K} = C \begin{bmatrix} \theta_{1:K-1} \\ \theta \end{bmatrix} \quad \text{where } C = \begin{bmatrix} I_{K-1} & 0_{1:K-1} \\ -\frac{1}{\pi_K} \pi_{1:K-1}^{\top} & \frac{1}{\pi_K} \end{bmatrix}.$$

In particular, we have

$$p^{\text{cut}}(\theta_{1:K-1}, \theta|D^{(r)}, D^{(e)}) = p^{(A2)}(\theta_{1:K-1}|\theta, D^{(r)}, D^{(e)}) \cdot p^{(A1)}(\theta|Y^{(r)}, T^{(r)}).$$

To find the first factor, note that under Analyst 2's posterior

$$(\theta_{1:K-1}, \theta) \sim N \left( \begin{bmatrix} \theta_{1:K-1}^{(A2)} \\ \bar{\theta}^{(A2)} \end{bmatrix}, \begin{bmatrix} \Sigma_{1:K-1}^{(A2)} & \Sigma_{1:K-1, \theta}^{(A2)} \\ \Sigma_{1:K-1, \theta}^{(A2)\top} & \Sigma_{\theta}^{(A1)} \end{bmatrix} \right),$$

where  $\bar{\theta}^{(A2)} = \pi^{\top} \theta_{1:K}^{(A2)}$ , and  $\Sigma_{1:K-1, \theta}^{(A2)} = \Sigma_{1:K-1, K}^{(A2)} \pi$  with  $\Sigma_{1:K-1, K}^{(A2)}$  being the first  $K-1$  rows of  $\Sigma_{1:K}^{(A2)}$ .

So by the conditioning property of the multivariate normal distribution, according to Analyst 2

$$\theta_{1:K-1}|\theta \sim N \left( \theta_{1:K-1}^{(A2)} + \Sigma_{1:K-1, \theta}^{(A2)} \Sigma_{\theta}^{-1} (\theta - \bar{\theta}^{(A2)}), \Sigma_{1:K-1}^{(A2)} - \Sigma_{1:K-1, \theta}^{(A2)} \Sigma_{\theta}^{-1} \Sigma_{1:K-1, \theta}^{(A2)\top} \right).$$

Since Analyst 1's posterior is  $\theta \sim N(\theta^{(A1)}, \Sigma_{\theta}^{(A1)})$ , under the cut distribution

$$(\theta_{1:K-1}, \theta) \sim N(m_{1:K-1, \theta}^{(\text{cut})}, \Sigma_{1:K-1, \theta}^{(\text{cut})}),$$

where we define

$$\begin{aligned} m_{1:K-1, \theta}^{(\text{cut})} &= \begin{bmatrix} \theta_{1:K-1}^{(A2)} + \Sigma_{1:K-1, \theta}^{(A2)} \Sigma_{\theta}^{(A1)-1} (\theta^{(A1)} - \bar{\theta}^{(A2)}) \\ \theta^{(A1)} \end{bmatrix}, \\ \Sigma_{1:K-1, \theta}^{(\text{cut})} &= \begin{bmatrix} \Sigma_{1:K-1}^{(A2)} + \Sigma_{\theta}^{-1} (r-1) \Sigma_{1:K-1, \theta}^{(A2)} \Sigma_{1:K-1, \theta}^{(A2)\top} & r \Sigma_{1:K-1, \theta}^{(A2)} \\ r \Sigma_{1:K-1, \theta}^{(A2)\top} & \Sigma_{\theta}^{(A1)} \end{bmatrix} \end{aligned}$$

and  $r = \Sigma_{\theta}^{(A1)} \Sigma_{\theta}^{(A2)-1}$  is the ratio of Analyst 1's posterior variance of  $\theta$  over Analyst 2's posterior variance of  $\theta$ .  $m_{1:K-1, \theta}^{(\text{cut})}$  can be computed by an application of the law of total expectation.  $\Sigma_{1:K-1, \theta}^{(\text{cut})}$

can be computed by the laws of total variance and covariance,

$$\begin{aligned}
Var^{(cut)}(\theta_{1:K-1}) &= E^{(A1)} \left[ Var^{(A2)}(\theta_{1:K-1}|\theta) \right] + Var^{(A1)} \left( E^{(A2)}[\theta_{1:K-1}|\theta] \right) \\
&= \Sigma_{1:K-1}^{(A2)} - \Sigma_{1:K-1,\theta}^{(A2)} \Sigma_{\theta}^{(A1)^{-1}} \Sigma_{1:K-1,\theta}^{(A2)\top} + Var^{(A1)} \left( \Sigma_{1:K-1,\theta}^{(A2)} \Sigma_{\theta}^{(A2)^{-1}} (\theta - \bar{\theta}^{(A2)}) \right) \\
&= \Sigma_{1:K-1}^{(A2)} - \Sigma_{1:K-1,\theta}^{(A2)} \Sigma_{\theta}^{-1} \Sigma_{1:K-1,\theta}^{(A2)\top} + \Sigma_{\theta}^{(A1)^{-1}} r \Sigma_{1:K-1,\theta}^{(A2)} \Sigma_{1:K-1,\theta}^{(A2)\top} \\
&= \Sigma_{1:K-1}^{(A2)} + \Sigma_{\theta}^{(A1)^{-1}} (r-1) \Sigma_{1:K-1,\theta}^{(A2)} \Sigma_{1:K-1,\theta}^{(A2)\top}
\end{aligned}$$

and

$$\begin{aligned}
Cov^{(cut)}(\theta_{1:K-1}, \theta) &= Cov^{(A1)} \left( E^{(A2)}(\theta_{1:K-1}|\theta), \theta \right) + E^{(A1)} \left( Cov^{(A2)}(\theta_{1:K-1}, \theta|\theta) \right) \\
&= Cov^{(A1)} \left( \Sigma_{1:K-1,\theta}^{(A2)} \Sigma_{\theta}^{(A2)^{-1}} (\theta - \bar{\theta}^{(A2)}), \theta \right) + 0 \\
&= \Sigma_{1:K-1,\theta}^{(A2)} \Sigma_{\theta}^{(A2)^{-1}} \Sigma_{\theta}^{(A1)} \\
&= r \Sigma_{1:K-1,\theta}^{(A2)}.
\end{aligned}$$

Since  $p^{(cut)}(\theta_{1:K-1}, \theta) | D^{(r)}, D^{(e)}$  is multivariate normal, we can find the marginal distribution  $p^{(cut)}(\theta_{1:K} | D^{(r)}, D^{(e)})$  using the linear transformation

$$\theta_{1:K} = \underbrace{\begin{bmatrix} I_{K-1} & 0_{1:K-1} \\ -\frac{1}{\pi_K} \pi_{1:K-1}^\top & \frac{1}{\pi_K} \end{bmatrix}}_{=C} \begin{bmatrix} \theta_{1:K-1} \\ \theta \end{bmatrix}.$$

So under the cut distribution,  $\theta_{1:K} \sim N \left( Cm_{1:K-1,\theta}^{(cut)}, C \Sigma_{1:K-1,\theta}^{(cut)} C^\top \right)$ .

### S2.4.3 Computing the mean

For the mean,

$$\begin{aligned}
Cm_{1:K-1,\theta}^{(cut)} &= \begin{bmatrix} I_{K-1} & 0_{1:K-1} \\ -\frac{1}{\pi_K} \pi_{1:K-1}^\top & \frac{1}{\pi_K} \end{bmatrix} \begin{bmatrix} \theta_{1:K-1}^{(A2)} + \Sigma_{1:K-1,\theta}^{(A2)} \Sigma_{\theta}^{(A1)^{-1}} (\theta^{(A1)} - \bar{\theta}^{(A2)}) \\ \theta^{(A1)} \end{bmatrix} \\
&= \begin{bmatrix} \theta_{1:K-1}^{(A2)} + \Sigma_{\theta}^{(A1)^{-1}} (\theta^{(A1)} - \bar{\theta}^{(A2)}) \Sigma_{1:K-1,\theta}^{(A2)} \\ -\frac{\pi_{1:K-1}^\top \theta_{1:K-1}^{(A2)}}{\pi_K} - \frac{\pi_{1:K-1}^\top \Sigma_{1:K-1,\theta}^{(A2)} \Sigma_{\theta}^{-1} (\theta^{(A1)} - \pi_{1:K-1}^\top \theta_{1:K-1}^{(A2)})}{\pi_K} + \frac{1}{\pi_K} \theta^{(A1)} \end{bmatrix}. \tag{S2.4.1}
\end{aligned}$$

To simplify the last entry of (S2.4.1) further, we will find the following substitutions useful:

- Recall that  $\bar{\theta}^{(A2)} = \pi^\top \theta_{1:K}^{(A2)}$  and notice that  $\theta_K^{(A2)} = \frac{\bar{\theta}^{(A2)} - \pi_{1:K-1}^\top \theta_{1:K-1}^{(A2)}}{\pi_K}$  implies

$$-\frac{\pi_{1:K-1}^\top \theta_{1:K-1}^{(A2)}}{\pi_K} = \theta_K^{(A2)} - \frac{\bar{\theta}^{(A2)}}{\pi_K}. \tag{S2.4.2}$$

- Note that  $\Sigma_{\theta}^{(A2)} = \pi^\top \Sigma_{1:K}^{(A2)} \pi$  (because  $\theta = \pi^\top \theta_{1:K}$  for fixed  $\pi$ ), and we can write

$$\pi^\top \Sigma_{1:K}^{(A2)} \pi = \pi_{1:K-1}^\top \Sigma_{1:K-1,1:K}^{(A2)} \pi + \pi_K \Sigma_{K,1:K}^{(A2)} \pi$$

where  $\Sigma_{1:K-1,1:K}^{(A2)}$  is the first  $K-1$  rows of  $\Sigma_{1:K}^{(A2)}$  and  $\Sigma_{K,1:K}^{(A2)}$  is the final row of  $\Sigma_{1:K}^{(A2)}$ . Rearranging, we can write

$$-\frac{\pi_{1:K-1}^\top \Sigma_{1:K-1,1:K}^{(A2)} \pi}{\pi_K} = \Sigma_{K,1:K} \pi - \frac{\pi^\top \Sigma_{1:K}^{(A2)} \pi}{\pi_K}$$

and recalling that we defined  $\Sigma_{1:K-1,\theta}^{(A2)} = \Sigma_{1:K-1,1:K}^{(A2)} \pi$  yields

$$-\frac{\pi_{1:K-1}^\top \Sigma_{1:K-1,1:K}^{(A2)} \pi}{\pi_K} = \Sigma_{K,1:K} \pi - \frac{\Sigma_\theta^{(A2)}}{\pi_K}. \quad (\text{S2.4.3})$$

Then the  $K$ -th entry of (S2.4.1) equals

$$\begin{aligned} &= \theta_K^{(A2)} - \frac{\bar{\theta}^{(A2)}}{\pi_K} + \left( \Sigma_{K,1:K} \pi - \frac{\Sigma_\theta^{(A2)}}{\pi_K} \right) \frac{1}{\Sigma_\theta^{(A2)}} \left( \theta^{(A1)} - \bar{\theta} \right) + \frac{1}{\pi_K} \theta^{(A1)} \\ &= \theta_K^{(A2)} + \Sigma_\theta^{(A2)-1} \Sigma_{K,1:K}^{(A2)} \pi \left( \theta^{(A1)} - \bar{\theta}^{(A2)} \right) + \frac{1}{\pi_K} \left( \theta^{(A1)} - \bar{\theta}^{(A2)} \right) - \frac{1}{\pi_K} \left( \theta^{(A1)} - \bar{\theta}^{(A2)} \right) \\ &= \theta_K^{(A2)} + \Sigma_\theta^{(A2)-1} \Sigma_{K,1:K}^{(A2)} \pi \left( \theta^{(A1)} - \bar{\theta}^{(A2)} \right). \end{aligned}$$

So (S2.4.1) becomes

$$m_{1:K}^{(cut)} = C m_{1:K-1,\theta}^{(cut)} = \theta_{1:K}^{(A2)} + \Sigma_\theta^{(A1)-1} \left( \theta^{(A1)} - \bar{\theta}^{(A2)} \right) \Sigma_{1:K}^{(A2)} \pi.$$

#### S2.4.4 Computing the variance

For the variance, writing  $S = \text{Var}^{(cut)} \left( \hat{\theta}_{1:K-1} \right) = \Sigma_{1:K-1}^{(A2)} + \Sigma_\theta^{(A1)-1} (r-1) \Sigma_{1:K-1,\theta}^{(A2)} \Sigma_{1:K-1,\theta}^{(A2)\top}$ ,

$$\begin{aligned} C \Sigma_{1:K-1,\theta}^{(cut)} C^\top &= \begin{bmatrix} I_{K-1} & 0_{1:K-1} \\ -\frac{1}{\pi_K} \pi_{1:K-1}^\top & \frac{1}{\pi_K} \end{bmatrix} \cdot \begin{bmatrix} S & r \Sigma_{1:K-1,\theta}^{(A2)} \\ r \Sigma_{1:K-1,\theta}^{(A2)\top} & \Sigma_\theta^{(A1)} \end{bmatrix} \cdot \begin{bmatrix} I_{K-1} & -\frac{1}{\pi_K} \pi_{1:K-1} \\ 0_{1:K-1}^\top & \frac{1}{\pi_K} \end{bmatrix} \\ &= \begin{bmatrix} S & r \Sigma_{1:K-1,\theta}^{(A2)} \\ -\frac{1}{\pi_K} \pi_{1:K-1}^\top S + \frac{1}{\pi_K} r \Sigma_{1:K-1,\theta}^{(A2)} & -\frac{1}{\pi_K} r \pi_{1:K-1}^\top \Sigma_{1:K-1,\theta}^{(A2)} + \frac{1}{\pi_K} \Sigma_\theta^{(A1)} \end{bmatrix} \begin{bmatrix} I_{K-1} & -\frac{1}{\pi_K} \pi_{1:K-1} \\ 0_{1:K-1}^\top & \frac{1}{\pi_K} \end{bmatrix} \\ &= \begin{bmatrix} S & A \\ A^\top & -\frac{1}{\pi_K} A^\top \pi_{1:K-1} - \frac{1}{\pi_K^2} r \pi_{1:K-1} \Sigma_{1:K-1,\theta}^{(A2)} + \frac{1}{\pi_K^2} \Sigma_\theta^{(A1)} \end{bmatrix} \quad (\text{S2.4.4}) \end{aligned}$$

where we write  $A = -\frac{1}{\pi_K} S \pi_{1:K-1} + \frac{1}{\pi_K} r \Sigma_{1:K-1,\theta}^{(A2)}$ .

To simplify this expression we use the following numbered substitutions:

- Rearranging substitution (S2.4.3) above from computing the mean, and using  $\Sigma_{K,\theta}^{(A2)} = \Sigma_{K,1:K}^{(A2)} \pi$ , we have

$$\pi_{1:K-1}^\top \Sigma_{1:K-1,\theta}^{(A2)} = \Sigma_\theta^{(A1)} - \pi_K \Sigma_{K,\theta}^{(A2)}. \quad (\text{S2.4.5})$$

- Note that

$$\begin{aligned} \Sigma_\theta^{(A2)} &= \pi^\top \Sigma_{1:K}^{(A2)} \pi = \begin{bmatrix} \pi_{1:K-1}^\top & \pi_K \end{bmatrix} \begin{bmatrix} \Sigma_{1:K-1}^{(A2)} & \Sigma_{1:K-1,K}^{(A2)} \\ \Sigma_{K,1:K-1}^{(A2)} & \Sigma_K^{(A2)} \end{bmatrix} \begin{bmatrix} \pi_{1:K-1} \\ \pi_K \end{bmatrix} \\ &= \pi_{1:K-1}^\top \Sigma_{1:K-1}^{(A2)} \pi_{1:K-1} + 2\pi_K \pi_{1:K-1}^\top \Sigma_{1:K-1,K}^{(A2)} + \pi_K^2 \Sigma_K^{(A2)} \end{aligned}$$

so

$$\pi_{1:K-1}^\top \Sigma_{1:K-1}^{(A2)} \pi_{1:K-1} = \Sigma_\theta^{(A2)} - 2\pi_K \pi_{1:K-1}^\top \Sigma_{1:K-1,K}^{(A2)} - \pi_K^2 \Sigma_K^{(A2)}. \quad (\text{S2.4.6})$$

- Note that we define  $\Sigma_{K,\theta}^{(A2)} = \Sigma_{K,1:K}^{(A2)} \pi$ , and  $\Sigma_{K,\theta}^{(A2)} = \pi^\top \Sigma_{1:K,K}^{(A2)} = \pi_{1:K-1}^\top \Sigma_{1:K-1,K}^{(A2)} + \pi_K \Sigma_K^{(A2)}$ , so

$$\pi_K \Sigma_K^{(A2)} = \pi^\top \Sigma_{1:K,K}^{(A2)} - \pi_{1:K-1}^\top \Sigma_{1:K-1,K}^{(A2)}. \quad (\text{S2.4.7})$$

To simplify the  $K \times K$ -th entry of (S2.4.4), i.e.  $\Sigma_K^{(cut)}$ , we may proceed:

$$\begin{aligned}
\Sigma_K^{(cut)} &= - \left[ \frac{-1}{\pi_K} \pi_{1:K-1}^\top S + \frac{1}{\pi_K} r \Sigma_{1:K-1,\theta}^{(A2)} \right] \frac{1}{\pi_K} \pi_{1:K-1} - \frac{1}{\pi_K^2} r \pi_{1:K-1} \Sigma_{1:K-1,\theta}^{(A2)} + \frac{1}{\pi_K^2} \Sigma_\theta^{(A1)} \\
&= \frac{1}{\pi_K^2} \pi_{1:K-1}^\top S \pi_{1:K-1} - 2 \frac{1}{\pi_K^2} r \pi_{1:K-1}^\top \Sigma_{1:K-1,\theta}^{(A2)} + \frac{1}{\pi_K^2} \Sigma_\theta^{(A1)} \\
&= \frac{1}{\pi_K^2} \pi_{1:K-1}^\top \left[ \Sigma_{1:K-1}^{(A2)} + \Sigma_\theta^{(A1)^{-1}} (r-1) \Sigma_{1:K-1,\theta}^{(A2)} \Sigma_{1:K-1,\theta}^{(A2)\top} \right] \pi_{1:K-1} \quad , \text{ plug in } S \\
&\quad - 2 \frac{1}{\pi_K^2} r \pi_{1:K-1}^\top \Sigma_{1:K-1,\theta}^{(A2)} + \frac{1}{\pi_K^2} \Sigma_\theta^{(A1)} \\
&= \frac{1}{\pi_K^2} \pi_{1:K-1}^\top \Sigma_{1:K-1}^{(A2)} \pi_{1:K-1} + \frac{1}{\pi_K^2} \Sigma_\theta^{(A2)^{-1}} (r-1) \left( \pi_{1:K-1}^\top \Sigma_{1:K-1,\theta}^{(A2)} \right)^2 \\
&\quad - 2 \frac{1}{\pi_K^2} r \left( \pi_{1:K-1}^\top \Sigma_{1:K-1,\theta}^{(A2)} \right) + \frac{1}{\pi_K^2} \Sigma_\theta^{(A1)} \\
&= \frac{1}{\pi_K^2} \pi_{1:K-1}^\top \Sigma_{1:K-1}^{(A2)} \pi_{1:K-1} + \frac{1}{\pi_K^2} \Sigma_\theta^{(A2)^{-1}} (r-1) \left( \Sigma_\theta^{(A2)} - \pi_K \Sigma_{K,\theta}^{(A2)} \right)^2 \quad , \text{ plug in (S2.4.5)} \\
&\quad - 2 \frac{1}{\pi_K^2} r \left( \Sigma_\theta^{(A2)} - \pi_K \Sigma_{K,\theta}^{(A2)} \right) + \frac{1}{\pi_K^2} \Sigma_\theta^{(A1)} \\
&= \frac{1}{\pi_K^2} \pi_{1:K-1}^\top \Sigma_{1:K-1}^{(A2)} \pi_{1:K-1} + \Sigma_\theta^{(A2)^{-1}} (r-1) \left[ \frac{1}{\pi_K^2} \Sigma_\theta^{(A2)^2} - 2 \frac{1}{\pi_K} \Sigma_\theta^{(A1)} \Sigma_{K,\theta}^{(A2)} + \Sigma_{K,\theta}^{(A2)^2} \right] \\
&\quad - 2 \frac{1}{\pi_K^2} r \left( \Sigma_\theta^{(A2)} - \pi_K \Sigma_{K,\theta}^{(A2)} \right) + \frac{1}{\pi_K^2} \Sigma_\theta^{(A1)} \\
&= \frac{1}{\pi_K^2} \left( \Sigma_\theta^{(A2)} - 2 \pi_K \pi_{1:K-1}^\top \Sigma_{1:K-1,\theta}^{(A2)} - \pi_K^2 \Sigma_{K,\theta}^{(A2)} \right) + \frac{1}{\pi_K^2} (r-1) \Sigma_\theta^{(A2)} \quad , \text{ plug in (S2.4.6)} \\
&\quad - 2 \frac{1}{\pi_K} (r-1) \Sigma_{K,\theta}^{(A2)} + \Sigma_\theta^{(A2)^{-1}} (r-1) \Sigma_{K,\theta}^{(A2)^2} - 2 \frac{1}{\pi_K^2} r \Sigma_\theta^{(A2)} \\
&\quad + 2 \frac{1}{\pi_K} r \Sigma_{K,\theta}^{(A2)} + \frac{1}{\pi_K^2} r \Sigma_\theta^{(A2)} \\
&= -\Sigma_K^{(A2)} + \Sigma_\theta^{(A2)^{-1}} (r-1) \Sigma_{K,\theta}^{(A2)^2} + \frac{1}{\pi_K^2} \Sigma_\theta^{(A2)} \underbrace{\left[ 1 + (r-1) - 2r + r \right]}_{=0} \\
&\quad - 2 \frac{1}{\pi_K} \left[ \pi_{1:K-1}^\top \Sigma_{1:K-1,\theta}^{(A2)} + (r-1) \Sigma_{K,\theta}^{(A2)} - r \Sigma_{K,\theta}^{(A2)} \right] \\
&= -\Sigma_K^{(A2)} + \Sigma_\theta^{(A2)^{-1}} (r-1) \Sigma_{K,\theta}^{(A2)^2} - 2 \frac{1}{\pi_K} \left[ \Sigma_{K,\theta}^{(A2)} - \pi_K \Sigma_K^{(A2)} - \Sigma_{K,\theta}^{(A2)} \right] \quad , \text{ plug in (S2.4.7)} \\
\Sigma_K^{(cut)} &= \Sigma_K + \Sigma_\theta^{(A2)^{-1}} (r-1) \Sigma_{K,\theta}^{(A2)^2}.
\end{aligned}$$

To simplify the off-diagonals of (S2.4.4), i.e.  $\Sigma_{1:K-1,K}^{(cut)}$ , we may proceed:

$$\begin{aligned}
\Sigma_{1:K-1,K}^{(cut)} &= \frac{-1}{\pi_K} \pi_{1:K-1}^\top S + \frac{1}{\pi_K} r \Sigma_{1:K-1,\theta}^{(A2)\top} \\
&= \frac{-1}{\pi_K} \pi_{1:K-1}^\top \left[ \Sigma_{1:K-1}^{(A2)} + \Sigma_\theta^{(A1)^{-1}} (r-1) \Sigma_{1:K-1,\theta}^{(A2)} \Sigma_{1:K-1,\theta}^{(A2)\top} \right] + \frac{1}{\pi_K} r \Sigma_{1:K-1,\theta}^{(A2)\top}, \quad \text{, plug in S} \\
&= \frac{-1}{\pi_K} \pi_{1:K-1}^\top \Sigma_{1:K-1}^{(A2)} - \frac{1}{\pi_K} \Sigma_\theta^{(A2)^{-1}} (r-1) \pi_{1:K-1}^\top \Sigma_{1:K-1,\theta}^{(A2)} \Sigma_{1:K-1,\theta}^{(A2)\top} + \frac{1}{\pi_K} r \Sigma_{1:K-1,\theta}^{(A2)\top} \\
&= \frac{-1}{\pi_K} \pi_{1:K-1}^\top \Sigma_{1:K-1}^{(A2)} - \frac{1}{\pi_K} \Sigma_\theta^{(A2)^{-1}} (r-1) \left( \Sigma_\theta^{(A2)} - \pi_K \Sigma_{K,\theta}^{(A2)} \right) \Sigma_{1:K-1,\theta}^{(A2)\top}, \quad \text{, plug in (S2.4.5)} \\
&\quad + \frac{1}{\pi_K} r \Sigma_{1:K-1,\theta}^{(A2)\top} \\
&= \frac{-1}{\pi_K} \pi_{1:K-1}^\top \Sigma_{1:K-1}^{(A2)} - \frac{1}{\pi_K} (r-1) \Sigma_{1:K-1,\theta}^{(A2)\top} + \frac{1}{\pi_K} (r-1) \left( \pi_K \Sigma_\theta^{(A2)^{-1}} \Sigma_{K,\theta}^{(A2)} \right) \Sigma_{1:K-1,\theta}^{(A2)\top} \\
&\quad + \frac{1}{\pi_K} r \Sigma_{1:K-1,\theta}^{(A2)\top} \\
&= \frac{-1}{\pi_K} \pi_{1:K-1}^\top \Sigma_{1:K-1}^{(A2)} + \frac{1}{\pi_K} \Sigma_{1:K-1,\theta}^{(A2)\top} + \Sigma_\theta^{(A2)^{-1}} (r-1) \Sigma_{K,\theta}^{(A2)} \Sigma_{1:K-1,\theta}^{(A2)\top} \\
&= \frac{1}{\pi_K} \left( \Sigma_{1:K-1,\theta}^{(A2)\top} - \pi_{1:K-1}^\top \Sigma_{1:K-1}^{(A2)} \right) + \Sigma_\theta^{(A2)^{-1}} (r-1) \Sigma_{K,\theta}^{(A2)} \Sigma_{1:K-1,\theta}^{(A2)\top} \\
&= \frac{1}{\pi_K} \left( \pi^\top \Sigma_{1:K-1,1:K}^{(A2)} - \pi_{1:K-1}^\top \Sigma_{1:K-1}^{(A2)} \right) + \Sigma_\theta^{(A2)^{-1}} (r-1) \Sigma_{K,\theta}^{(A2)} \Sigma_{1:K-1,\theta}^{(A2)\top} \\
&= \frac{1}{\pi_K} \left( \pi_K \Sigma_{1:K-1,K}^{(A2)} \right) + \Sigma_\theta^{(A2)^{-1}} (r-1) \Sigma_{K,\theta}^{(A2)} \Sigma_{1:K-1,\theta}^{(A2)\top} \\
\Sigma_{1:K-1,K}^{(cut)} &= \Sigma_{1:K-1,K}^{(A2)} + \Sigma_\theta^{(A2)^{-1}} (r-1) \Sigma_{K,\theta}^{(A2)} \Sigma_{1:K-1,\theta}^{(A2)\top}.
\end{aligned}$$

So (S2.4.4) becomes

$$\Sigma_{1:K}^{(cut)} = C \Sigma_{1:K-1,\theta}^{(cut)} C^\top = \Sigma_{1:K}^{(A2)} + \Sigma_\theta^{(A2)^{-1}} (r-1) \Sigma_{1:K}^{(A2)} \pi \pi^\top \Sigma_{1:K}^{(A2)},$$

since  $\Sigma_{1:K,\theta}^{(A2)} = \Sigma_{1:K}^{(A2)} \pi$  and  $\Sigma_{1:K}^{(A2)}$  is symmetric. This concludes the derivation.

### S2.4.5 Condition for the cut estimator in Section 2.3 to be unbiased

We consider data generated under model (6). If  $\gamma_1 = \dots = \gamma_K$  the cut estimator (equation (16), Section 2.3) is unbiased when  $\Sigma_{1:K}^{(A2)} \propto \text{diag} \left( \frac{q_k}{\pi_k} \right)$  (see equation (10)). The posterior variance  $\Sigma_{1:K}^{(A2)}$ , from conjugacy results (Lindley and Smith, 1972), is equal to

$$\Sigma_{1:K}^{(A2)} = \phi^2 \text{diag} \left( \frac{\sigma_\mu^{-2} + n_{k,\cdot}^{(r+e)}}{\left( \sigma_\mu^{-2} + n_{k,\cdot}^{(r+e)} \right) \left( \sigma_\theta^{-2} + n_{k,1}^{(r)} \right) - n_{k,1}^{(r)^2}} \right),$$

where  $\sigma_\mu^{-2}$  is the prior precision of  $\mu_k$  and  $\sigma_\theta^{-2}$  is the prior precision of  $\theta_k$ . When we consider a non-informative (flat) prior for the parameters  $\mu_{1:K}$  and  $\theta_{1:K}$  (i.e.,  $\sigma_\mu^{-2} = \sigma_\theta^{-2} = 0$ ), we have

$$\Sigma_{1:K}^{(A2)} = \phi^2 \text{diag} \left( \frac{n_{k,\cdot}^{(r+e)}}{n_{k,\cdot}^{(r+e)} n_{k,1}^{(r)} - n_{k,1}^{(r)^2}} \right) = \phi^2 \text{diag} \left( \frac{n_{k,\cdot}^{(r+e)}}{n_{k,1}^{(r)} n_{k,0}^{(r+e)}} \right).$$

Thus  $\Sigma_{1:K}^{(A2)} \propto \text{diag}\left(\frac{q_k}{\pi_k}\right)$  if

$$\frac{q_k}{\pi_k} \propto \frac{n_{k,0}^{(e)}}{n_{k,1}^{(r)} n_{k,0}^{(r+e)}}$$

for all  $k = 1, \dots, K$ . This condition is met when the ratios  $\frac{n_{k,0}^{(e)}}{n_{k,1}^{(r)}}$  and  $\frac{n_{k,1}^{(r)}}{n_{k,0}^{(r)}}$  remain the same across subgroups  $k = 1, \dots, K$ .

## S2.5 Details for Figure 2 (Cut distribution example)

To generate the data set used for Figure 2, we took a single sample from model (6), with parameter values  $\mu_{1:K} = (0, 0)$ ,  $\theta_{1:K} = (-1, 0)$ , and  $\gamma_{1:K} = (0.5, 0.5)$ . We have  $K = 2$  subgroups, with  $n^{(r)} = 100$ ,  $n^{(e)} = 500$ , and  $\pi = (0.4, 0.6)$ . As in the first part of Section 2.2, within each subgroup

$$\frac{n_{k,0}^{(r)}}{n_{\cdot,0}^{(r)}} = \frac{n_{k,1}^{(r)}}{n_{\cdot,1}^{(r)}} = \frac{n_{k,\cdot}^{(e)}}{n^{(e)}} = \pi_k.$$

To construct the cut distribution, for Analyst 1 we use the prior parameters  $m^{(A1)} = 0_{2 \times 1}$  and  $\tau^{(A1)} = 100 \cdot I_2$ , and for Analyst 2 we use the prior parameters  $m^{(A2)} = 0_{4 \times 1}$  and  $\tau^{(A2)} = 100 \cdot I_4$ .

## S2.6 Proof for Section 2.4 (Interval estimation)

Recall from Section S2.4.1 that

$$\Sigma_{1:K}^{(cut)} = \Sigma_{1:K}^{(A2)} + \left( \frac{1}{\Sigma_{\theta}^{(A2)}} \right)^2 \left( \Sigma_{\theta}^{(A1)} - \Sigma_{\theta}^{(A2)} \right) \Sigma_{1:K}^{(A2)} \pi \pi^{\top} \Sigma_{1:K}^{(A2)}.$$

Also recall from equation (10) that

$$V^h = \phi^2 \left[ \frac{1}{n_{\cdot,1}^{(r)}} I_K + \frac{1}{n_{\cdot,0}^{(r)}} Q \right] \Pi^{-1} + \left( c \frac{\lambda}{\lambda + c} \right)^2 (1 - \bar{q}) \frac{1}{n_{\cdot,0}^{(r)}} \phi^2 \Sigma \pi \pi^{\top} \Sigma.$$

**Claim S2.** Suppose that:

- (i) Analysts 1 and 2 use flat priors ( $\tau^{(A1)}$  and  $\tau^{(A2)}$  are diagonal with diverging diagonal entries),
- (ii) the variance parameters  $\sigma^2$  and  $\phi^2$  in models (12), (13), and (6) (underlying  $V^h$ ) are identical, and
- (iii)  $\hat{\theta}_{1:K}^h$  is defined with  $\lambda = \infty$  and  $\Sigma$  is diagonal with entries proportional to  $\frac{1}{n_{k,1}^{(r)}} + \frac{1}{n_{k,0}^{(r+e)}}$ .

Then  $V^{(cut)} = V^h$ .

*Proof.* Note that from equation (10) and assumption (iii) (i.e.  $\lambda = \infty$ ) we have

$$\begin{aligned} V^h &= \phi^2 \left[ \frac{1}{n_{\cdot,1}^{(r)}} I_K + \frac{1}{n_{\cdot,0}^{(r)}} Q \right] \Pi^{-1} + \left( \pi^{\top} \Sigma \pi \right)^{-1} (1 - \bar{q}) \frac{1}{n_{\cdot,0}^{(r)}} \phi^2 \Sigma \pi \pi^{\top} \Sigma \\ &= \phi^2 \text{diag} \left( \frac{n_{k,\cdot}^{(r+e)}}{n_{k,1}^{(r)} n_{k,0}^{(r+e)}} \right) + \left( \pi^{\top} \Sigma \pi \right)^{-1} (1 - \bar{q}) \frac{1}{n_{\cdot,0}^{(r)}} \phi^2 \Sigma \pi \pi^{\top} \Sigma. \end{aligned}$$

In addition, note from assumption (i) and Section S2.4.5 we have

$$\begin{aligned}\Sigma_{1:K}^{(A2)} &= \phi^2 \text{diag} \left( \frac{n_{k,\cdot}^{(r+e)}}{n_{k,1}^{(r)} n_{k,0}^{(r+e)}} \right) \\ &\propto \Sigma,\end{aligned}$$

where the second line follows by assumption (iii). Thus

$$V^h = \Sigma_{1:K}^{(A2)} + \left( \pi^\top \Sigma_{1:K}^{(A2)} \pi \right)^{-1} (1 - \bar{q}) \frac{1}{n_{\cdot,0}^{(r)}} \phi^2 \Sigma_{1:K}^{(A2)} \pi \pi^\top \Sigma_{1:K}^{(A2)}.$$

Also, from Section S2.4.3, recall that  $\pi^\top \Sigma_{1:K}^{(A2)} \pi = \Sigma_\theta^{(A2)}$ . Finally, note that  $\Sigma_\theta^{(A2)^{-1}} \left( \Sigma_\theta^{(A1)} - \Sigma_\theta^{(A2)} \right) = (1 - \bar{q}) \frac{1}{n_{\cdot,0}^{(r)}} \phi^2$  by assumption (ii) and standard conjugate Bayesian linear regression calculations (Lindley and Smith, 1972). Thus

$$\begin{aligned}V^h &= \Sigma_{1:K}^{(A2)} + \left( \frac{1}{\Sigma_\theta^{(A2)}} \right)^2 \left( \Sigma_\theta^{(A1)} - \Sigma_\theta^{(A2)} \right) \Sigma_{1:K}^{(A2)} \pi \pi^\top \Sigma_{1:K}^{(A2)} \\ &= V^{(cut)}.\end{aligned}$$

□

## S2.7 Splitting and merging subgroups

Harmonized estimates can be computed for various partitions that group patients in different ways. For example, a partition of the population can be changed by merging two biomarker subgroups into a single category. In this subsection we discuss the concept of *invariance* of the estimator across nested partitions.

**Definition** (Invariance). *Consider a population partitioned into  $K$  subgroups. Without loss of generality, the investigator merges subgroups  $K - 1$  and  $K$ , and creates a new partition of the patient population. A generic estimation procedure allows the investigator to compute  $\hat{\theta}_{1:K}$ , the subgroup-specific treatment effect estimates for the original partition, and the analogous  $\hat{\theta}'_{1:K-1}$  for the modified partition. The procedure is invariant if*

$$\hat{\theta}'_\ell = \begin{cases} \hat{\theta}_\ell, & \ell < K - 1, \\ \frac{\pi_{K-1}}{\pi_{K-1} + \pi_K} \hat{\theta}_{K-1} + \frac{\pi_K}{\pi_{K-1} + \pi_K} \hat{\theta}_K, & \ell = K - 1. \end{cases}$$

The invariance property that we defined can be summarized by the equation

$$\hat{\theta}'_{1:K-1} = Z \hat{\theta}_{1:K}, \text{ where}$$

$$Z = \begin{bmatrix} I_{K-2}, & 0_{(K-2) \times 2} \\ 0_{1 \times (K-2)}, & \frac{\pi_{K-1}}{\pi_{K-1} + \pi_K}, & \frac{\pi_K}{\pi_{K-1} + \pi_K} \end{bmatrix}, \text{ and}$$

$0_{m \times w}$  denotes an  $m \times w$  matrix of zeros.

The next proposition describes simple conditions for the harmonized estimator to be invariant when we merge subgroups.

**Proposition S1.** *Consider the harmonized estimators*

$$\hat{\theta}_{1:K}^h = \hat{\theta}_{1:K}^{(r+e)} + c \frac{\lambda}{\lambda + c} \left( \hat{\theta}^{(r)} + \pi^\top \hat{\theta}_{1:K}^{(r+e)} \right) \Sigma \pi$$

(see equation (5)) and

$$\hat{\theta}_{1:K-1}^h = \hat{\theta}_{1:K-1}^{(r+e)} + c' \frac{\lambda}{\lambda + c'} \left( \hat{\theta}^{(r)} + \pi'^\top \hat{\theta}_{1:K-1}^{(r+e)} \right) \Sigma' \pi',$$

where  $\pi' = (\pi_1, \dots, \pi_{K-2}, \pi_{K-1} + \pi_K)$ ,  $c = (\pi^\top \Sigma \pi)^{-1}$  and  $c' = (\pi'^\top \Sigma' \pi')^{-1}$ . If (a)  $\hat{\theta}_{1:K-1}^{(r+e)} = Z \hat{\theta}_{1:K}^{(r+e)}$ , and (b)  $\Sigma' = Z \Sigma Z^\top$ , then  $\hat{\theta}_{1:K-1}^h = Z \hat{\theta}_{1:K}^h$ .

*Proof.* By its invariance,  $\hat{\theta}_{1:K-1}^{(r+e)} = Z \hat{\theta}_{1:K}^{(r+e)}$ . Then

$$\begin{aligned} \hat{\theta}_{1:K-1}^h &= Z \hat{\theta}_{1:K}^{(r+e)} + c' \frac{\lambda}{\lambda + c'} \left( \hat{\theta}^{(r)} + \pi'^\top Z \hat{\theta}_{1:K}^{(r+e)} \right) \Sigma' \pi' \\ &= Z \hat{\theta}_{1:K}^{(r+e)} + c' \frac{\lambda}{\lambda + c'} \left( \hat{\theta}^{(r)} + \pi'^\top Z \hat{\theta}_{1:K}^{(r+e)} \right) Z \Sigma Z^\top \pi' \\ &= Z \hat{\theta}_{1:K}^{(r+e)} + c \frac{\lambda}{\lambda + c} \left( \hat{\theta}^{(r)} + \pi^\top \hat{\theta}_{1:K}^{(r+e)} \right) Z \Sigma \pi \\ &= Z \hat{\theta}_{1:K}^h. \end{aligned}$$

Here the second equation plugs in  $\Sigma' = Z \Sigma Z^\top$ , and the third line follows because  $Z^\top \pi' = \pi$  (by definition of  $Z$  and  $\pi'$ ), which also implies that  $c' = (\pi'^\top \Sigma' \pi')^{-1} = (\pi'^\top Z \Sigma Z^\top \pi')^{-1} = (\pi^\top \Sigma \pi)^{-1} = c$ . So  $\hat{\theta}_{1:K}^h$  is invariant to merging of subgroups.  $\square$

To summarize, if (a)  $\hat{\theta}_{1:K}^{(r+e)}$  is invariant to merging subgroups and (b)  $\Sigma$  is appropriately redefined after merging, then  $\hat{\theta}_{1:K}^h$  is also invariant. For example, consider harmonizing a Bayesian subgroup analysis. First, the investigator computes the posterior  $p(\theta_{1:K} | D^{(r)}, D^{(e)})$  and specifies  $\hat{\theta}_{1:K}^{(r+e)}$  in equation (5) equal to the posterior mean, and  $\Sigma$  equal to the posterior variance of  $\theta_{1:K}$ . After merging subgroups  $K$  and  $(K-1)$ , the investigator computes the posterior  $p(\theta'_{1:K-1} | D^{(r)}, D^{(e)})$  of  $\theta'_{1:K-1} = Z \theta_{1:K}$ , and plugs into equation (5) the posterior mean and the posterior variance of  $\theta'_{1:K-1}$ . Since the posterior  $p(\theta'_{1:K-1} | D^{(r)}, D^{(e)})$  has mean  $Z \hat{\theta}_{1:K}^{(r+e)}$  and variance  $Z \Sigma Z^\top$ , the harmonized estimates  $\hat{\theta}_{1:K}$  and  $\hat{\theta}'_{1:K-1}$  — before and after merging — are coherent; indeed Proposition 1 indicates that the invariance property holds.

In Section 3 we discussed several harmonized estimators; in some cases the input  $\hat{\theta}_{1:K}^{(r+e)}$  is invariant to the merging of subgroups. For example, with the linear model of Section 3.1 (treatment effect estimator: equation (21)) the estimator is invariant when the covariates and subgroup indicators are orthogonal, while in the Section 3.2 the estimator  $\hat{\theta}_{1:K}^{(r+e)}$  based on logistic regression is not invariant.

## S2.8 Large sample behavior of harmonization

As shown in equation (5), the harmonized estimator  $\hat{\theta}_{1:K}^h$  is a linear combination of  $\hat{\theta}_{1:K}^{(r+e)}$  and  $\hat{\theta}^{(r)}$ . This makes it simple to derive the limit in probability of  $\hat{\theta}_{1:K}^h$  when

- (i)  $\hat{\theta}_{1:K}^{(r+e)}$  converges in probability,
- (ii)  $\hat{\theta}^{(r)}$  converges in probability, and
- (iii)  $\hat{\theta}_{1:K}^h$  uses a (possibly data-driven, see for example Section 3.2)  $\hat{\Sigma}$  such that  $\hat{\Sigma} \xrightarrow{P} \Sigma$  for *some* invertible  $K \times K$  matrix  $\Sigma$ .

In particular if  $\hat{\theta}_{1:K}^{(r+e)} \xrightarrow{P} \theta_{1:K}$ ,  $\hat{\theta}^{(r)} \xrightarrow{P} \theta = \pi^\top \theta_{1:K}$ , and  $\hat{\Sigma} \xrightarrow{P} \Sigma$  then equation (5) implies that  $\hat{\theta}_{1:K}^h \xrightarrow{P} \theta_{1:K} + (\pi^\top \theta_{1:K} - \pi^\top \theta_{1:K}) c \frac{\lambda}{\lambda + c} \Sigma \pi = \theta_{1:K}$ . Note that the same arguments can be used to discuss the convergence of  $\hat{\theta}_{1:K}^h$  when the limit of  $\hat{\theta}_{1:K}^{(r+e)}$  or  $\hat{\theta}^{(r)}$  in probability is different from  $\theta_{1:K}$ .

and  $\pi^\top \theta_{1:K}$  respectively. To summarize, the use of a consistent  $\hat{\theta}_{1:K}^{(r+e)}$  estimator results in consistent harmonized estimators  $\hat{\theta}_{1:K}^h$  for any  $\lambda$  and  $\hat{\Sigma}$ , unless the primary analysis  $\hat{\theta}^{(r)}$  is inconsistent or  $\hat{\Sigma}$  does not converge in probability. For example, a subgroup-specific treatment effect estimator based on Bayesian model averaging ideas as in (Kotalik et al., 2021)) satisfies  $\hat{\theta}_{1:K}^{(r+e)} \xrightarrow{p} \theta_{1:K}$  in all three scenarios of Figure 1.

Figure S2 below is similar to Figure 1 (same scenarios and estimators) but we vary the sample sizes. Also,  $\lambda = \infty$ . We consider RCT sample sizes  $n^{(r)} \in [60, 1000]$ , with 1:1 randomization and an EC group 10 times the size of the RCT control group ( $n^{(e)} = 10 \cdot \frac{1}{2}n^{(r)}$ ). As the sample size increases, the biases of the estimators remain constant while the variances reduce.

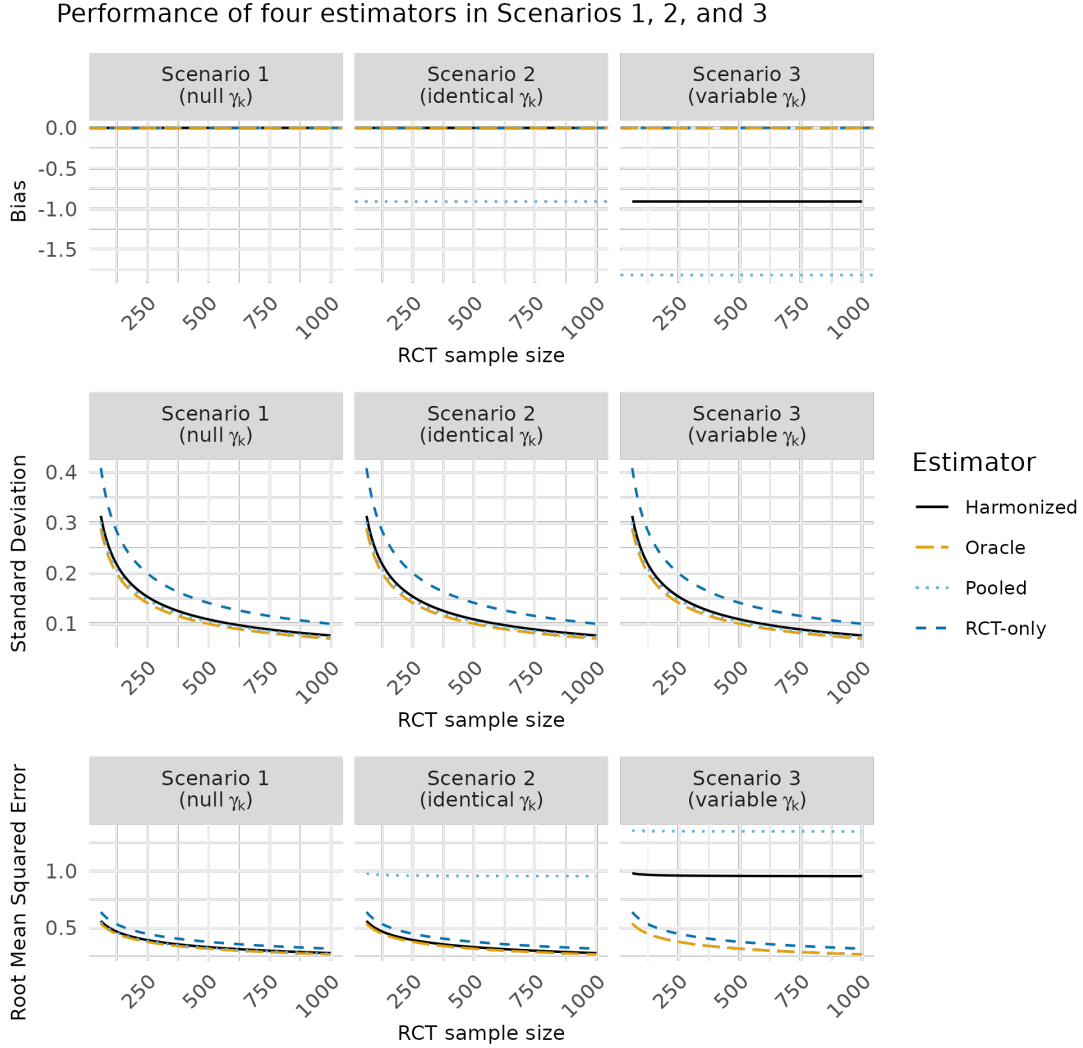

Figure S2: Performance summaries of the harmonized estimator (using Proposition 1) and other estimators (analogous analytic results) for subgroup  $k = 1$  as the total sample size  $n^{(r)}$  of the RCT varies (x-axis). The RCT has 1:1 randomization and the EC group was 10 times the size of the RCT control group ( $n^{(e)} = 10 \cdot \frac{1}{2}n^{(r)}$ ). We illustrate the bias, standard deviation, and the root mean squared error (RMSE) of the estimator as a function of  $n^{(r)}$ . The scenarios have different  $\gamma_{1:K}$  values:  $0_{K \times 1}$  (Scenario 1), constant across subgroups (Scenario 2), or varying across subgroups, with  $\gamma_{1:K} = (1 + \Delta_\gamma, 1 - \Delta_\gamma, 1 + \Delta_\gamma, 1 - \Delta_\gamma, \dots)$  and  $\Delta_\gamma = 1$  (Scenario 3).

In addition, we conducted additional simulations for Scenario 3 in Section 3.1 in which the RCT sample size  $n^{(r)}$  was fixed and the EC sample size  $n^{(e)}$  increased. Thus  $n^{(e)}/n^{(r)} \rightarrow \infty$ . Results are

Performance of the estimators by EC sample size  
in Scenario 3

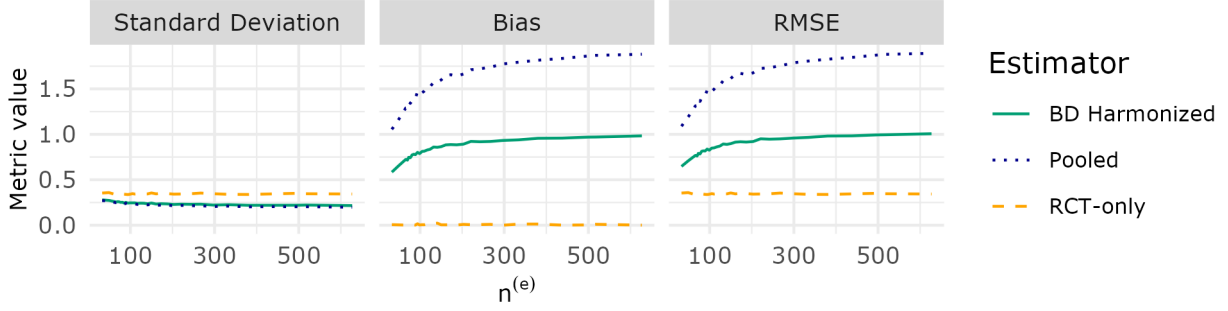

Figure S3: Violation of the SDM assumption. Standard deviation, bias, and RMSE of estimators of  $\theta_1$  (setting: linear model, Section 3.1) when the EC sample size varies. Results are based on 2,000 simulation replicates from the same data generating process used in Figure 4, Scenario 3 except that the EC sample size  $n^{(e)}$  varies. The RCT control group size is  $n_{\cdot,0}^{(r)} = 33$ , the RCT treatment group size is  $n_{\cdot,1}^{(r)} = 67$ .

shown in Figure S3. They show that the operating characteristics of  $\hat{\theta}_{1:K}^h$  and  $\hat{\theta}_{1:K}^{(r+e)}$ , especially bias and RMSE, depend on the relative size of  $n^{(e)}$  compared to the trial. As expected both estimators are relatively less biased when  $n^{(e)}$  is smaller. However, the ratio of the RMSEs of pooling and harmonization are relatively stable across all sample sizes we consider.

## S3 Additional material for Section 3

### S3.1 Proofs for Section 3.1 (linear regression)

#### S3.1.1 Bias and variance of $\hat{\theta}_{1:K}^{(r+e)}$

In this setting we have

$$\hat{\theta}_{1:K}^{(r+e)} = \begin{bmatrix} 0_{K \times K} & I_K & 0_{K \times d} \end{bmatrix} (M_1^\top M_1)^{-1} M_1^\top \begin{bmatrix} Y_{i:n(r)}^{(r)} \\ Y_{i:n(e)}^{(e)} \end{bmatrix},$$

where  $M_1$  is the design matrix for the pooled OLS model (20). Under model (S3.8.1),

$$E \left( \begin{bmatrix} Y_{i:n(r)}^{(r)} \\ Y_{i:n(e)}^{(e)} \end{bmatrix} \right) = M_1 \begin{bmatrix} \mu_{1:K} \\ \theta_{1:K} \\ \beta \end{bmatrix} + M_2 \gamma_{1:K},$$

where  $M_2$  are the design matrix columns corresponding to  $\gamma_{1:K}$  in model (S3.8.1). Thus

$$\begin{aligned} E \left( \hat{\theta}_{1:K}^{(r+e)} \right) &= \begin{bmatrix} 0_{K \times K} & I_K & 0_{K \times d} \end{bmatrix} (M_1^\top M_1)^{-1} M_1^\top \left( M_1 \begin{bmatrix} \mu_{1:K} \\ \theta_{1:K} \\ \beta \end{bmatrix} + M_2 \gamma_{1:K} \right) \\ &= \begin{bmatrix} 0_{K \times K} & I_K & 0_{K \times d} \end{bmatrix} \begin{bmatrix} \mu_{1:K} \\ \theta_{1:K} \\ \beta \end{bmatrix} + \begin{bmatrix} 0_{K \times K} & I_K & 0_{K \times d} \end{bmatrix} (M_1^\top M_1)^{-1} M_1^\top M_2 \gamma_{1:K}, \\ E \left( \hat{\theta}_{1:K}^{(r+e)} \right) &= \theta_{1:K} + \begin{bmatrix} 0_{K \times K} & I_K & 0_{K \times d} \end{bmatrix} (M_1^\top M_1)^{-1} M_1^\top M_2 \gamma_{1:K}. \end{aligned}$$

For the variance, recall that  $\text{Var} \left( \begin{bmatrix} Y_{i:n(r)}^{(r)} \\ Y_{i:n(e)}^{(e)} \end{bmatrix} \right) = \phi^2 I_{n(r)+n(e)}$ , so

$$\text{Var} \left( \hat{\theta}_{1:K}^{(r+e)} \right) = \phi^2 \begin{bmatrix} 0_{K \times K} & I_K & 0_{K \times d} \end{bmatrix} \left( M_1^\top M_1 \right)^{-1} \begin{bmatrix} 0_{K \times K} & I_K & 0_{K \times d} \end{bmatrix}^\top.$$

### S3.1.2 Unbiasedness of $\hat{\theta}^{(r)}$

Here we give sufficient conditions for the OLS estimator of  $\theta$  under model (S3.8.1) to be unbiased. Recall that we write  $M_0$  for the design matrix of model (20).

**Claim S3.** *Assume that the RCT outcome vector  $Y_{1:n(r)}^{(r)}$  is sampled independently according to model (S3.8.1),  $P(W_i^{(r)} = k | X_i^{(r)}, T_i^{(r)}) = \pi_k$  for all  $i$  and  $k$ , and  $M_0$  is invertible. Then the estimator  $\hat{\theta}^{(r)} = [0, 1, 0_{1 \times d}] (M_0^\top M_0)^{-1} M_0^\top Y_{1:n(r)}^{(r)}$  has bias*

$$E(\hat{\theta}^{(r)} | T_{1:n(r)}^{(r)}, X_{1:n(r)}^{(r)}) - \pi^\top \theta_{1:K} = 0.$$

*Proof.* By definition of  $\hat{\theta}^{(r)}$  we have

$$E(\hat{\theta}^{(r)} | T_{1:n(r)}^{(r)}, X_{1:n(r)}^{(r)}) = [0, 1, 0_{1 \times d}] (M_0^\top M_0)^{-1} M_0^\top E(Y_i^{(r)} | T_{1:n(r)}^{(r)}, X_{1:n(r)}^{(r)}). \quad (\text{S3.1.1})$$

Note that

$$\begin{aligned} E(Y_i^{(r)} | T_{1:n(r)}^{(r)}, X_{1:n(r)}^{(r)}) &= E(\mu_{W_i^{(r)}} + \theta_{W_i^{(r)}} T_i^{(r)} + \beta X_i^{(r)} | T_i^{(r)}, X_i^{(r)}) \\ &= \pi^\top \mu_{1:K} + \pi^\top \theta_{1:K} T_i^{(r)} + \beta X_i^{(r)}. \end{aligned}$$

Therefore  $E(Y_{1:n(r)}^{(r)} | T_{1:n(r)}^{(r)}, X_{1:n(r)}^{(r)}) = M_0 \begin{bmatrix} \pi^\top \mu_{1:K} \\ \pi^\top \theta_{1:K} \\ \beta \end{bmatrix}$  and plugging this in to equation (S3.1.1) concludes the proof.  $\square$

$$\text{The bias equals zero if } E(Y_{1:n(r)}^{(r)} | T_{1:n(r)}^{(r)}, X_{1:n(r)}^{(r)}) = M_0 \begin{bmatrix} \pi^\top \mu_{1:K} \\ \pi^\top \theta_{1:K} \\ \beta \end{bmatrix}.$$

### S3.1.3 Propositions 3-5

Recall that we use the notation  $S = \text{Var}(\hat{\theta}_{1:K}^{(r+e)}, \hat{\theta}^{(r)})$  and  $u = c \frac{\lambda}{\lambda+c} \Sigma \pi$ . The harmonized estimator can be rewritten as

$$\hat{\theta}_{1:K}^h = \hat{\theta}_{1:K}^{(r+e)} + (\hat{\theta}^{(r)} - \pi^\top \hat{\theta}_{1:K}^{(r+e)}) u.$$

**Proposition 2.** *If the following two assumptions hold*

$$(A1) \quad E(\hat{\theta}^{(r)}) - \pi^\top \theta_{1:K} = 0, \text{ and}$$

$$(A2) \quad E(\hat{\theta}_{1:K}^{(r+e)}) - \theta_{1:K} = B \gamma_{1:K}, \text{ where } B \text{ is a } K \times K \text{ matrix,}$$

then, with  $P = [I_K - u \pi^\top, \quad u]$ ,

$$\text{Bias}(\hat{\theta}_{1:K}^h, \theta_{1:K}) = (I_K - u \pi^\top) B \gamma_{1:K}, \quad (27)$$

$$\text{Var}(\hat{\theta}_{1:K}^h) = P S P^\top. \quad (28)$$

*Proof.* For the bias, note that

$$\begin{aligned}
E\left(\hat{\theta}_{1:K}^h\right) - \theta_{1:K} &= E\left(\hat{\theta}_{1:K}^{(r+e)}\right) - \theta_{1:K} + u \left[ E(\hat{\theta}^{(r)}) - \pi^\top E\left(\hat{\theta}_{1:K}^{(r+e)}\right) \right] \\
&= B\gamma_{1:K} + u \left[ \pi^\top \theta_{1:K} - \pi^\top \theta_{1:K} - \pi^\top B\gamma_{1:K} \right] \\
&= B\gamma_{1:K} - u\pi^\top B\gamma_{1:K} \\
&= (I_K - u\pi^\top)B\gamma_{1:K}.
\end{aligned}$$

For the variance, note that  $\hat{\theta}_{1:K}^h = P \begin{bmatrix} \hat{\theta}_{1:K}^{(r+e)} \\ \hat{\theta}^{(r)} \end{bmatrix}$ , so  $\text{Var}\left(\hat{\theta}_{1:K}^h\right) = P\text{Var}\left(\begin{bmatrix} \hat{\theta}_{1:K}^{(r+e)} \\ \hat{\theta}^{(r)} \end{bmatrix}\right)P^\top = PSP^\top$ .  $\square$

Recall that in the following proposition we use the notation  $b = (b_1, \dots, b_K) = B1_{K \times 1}$ .

**Proposition 3.** *If assumptions (A1) and (A2) are satisfied,  $\gamma_{1:K} = \gamma 1_{K \times 1}$  for some  $\gamma \in \mathbb{R}$ , and  $b \neq 0_{K \times 1}$ , then  $\hat{\theta}_{1:K}^h$  is unbiased (i.e.  $E\left(\hat{\theta}_{1:K}^h\right) = \theta_{1:K}$ ) if and only if  $\lambda = \infty$  and  $\Sigma\pi = \kappa b$  for some  $\kappa \neq 0$ .*

*Proof.* ( $\implies$ ): By Proposition 2 and the fact that  $\gamma_{1:K} \propto 1_{K \times 1}$ ,  $\hat{\theta}_{1:K}^h$  being unbiased implies that  $(I_K - u\pi^\top)b = 0_{K \times 1}$  and  $b = u\pi^\top b$ , so  $u$  is a multiple of  $b$ . Since  $\Sigma\pi$  is a multiple of  $u$ , it must also be a multiple of  $b$  (i.e.  $\Sigma\pi = \kappa b$  for some  $\kappa \neq 0$ ).

Further, we have

$$\begin{aligned}
b &= \left(\pi^\top \Sigma \pi\right)^{-1} \frac{\lambda}{\lambda + (\pi^\top \Sigma \pi)^{-1}} \Sigma \pi \left(\pi^\top b\right) \\
b\pi^\top &= \left(\pi^\top \Sigma \pi\right)^{-1} \frac{\lambda}{\lambda + (\pi^\top \Sigma \pi)^{-1}} \Sigma \pi \pi^\top \left(\pi^\top b\right)
\end{aligned}$$

( $\impliedby$ ): By Proposition 2, we have  $(I_K - u\pi^\top)b = 0_{K \times 1}$ .  $\square$

**Proposition 4.** *There exists a positive definite matrix  $\Sigma \in \mathbb{R}^{K \times K}$  such that  $\Sigma\pi = \kappa b$  for some  $\kappa \neq 0$  if and only if  $\pi^\top b \neq 0$ .*

*Proof.* ( $\implies$ ): Since  $\Sigma$  is positive definite,  $\pi^\top \Sigma \pi = \kappa \pi^\top b > 0$ . Therefore  $\pi^\top b \neq 0$ .

( $\impliedby$ ): For convenience we introduce the notation  $z = \frac{b}{\pi^\top b}$ .

Suppose  $z$  is a multiple of  $\pi$ . By definition  $\pi^\top z = 1$  and since  $\pi$  has all positive entries,  $z$  must be a positive multiple of  $\pi$ . Then  $\Sigma$  can be chosen as  $\Sigma = \text{diag}\left(\left(\frac{z_k}{\pi_k}\right)_{1:K}\right)$ . Trivially  $\Sigma\pi = z$ .

Suppose  $z$  is not a multiple of  $\pi$ . Then by Cauchy-Schwartz inequality  $1 = (\pi^\top z)^2 < \|\pi\|_2^2 \|z\|_2^2$ . Hence  $\|z\|_2 > 1$ . Define  $v_1 = \frac{2z - \pi}{\|2z - \pi\|_2}$ . Take  $\tilde{v}_2 = -\frac{1 - 2\|z\|_2^2}{2 - \|\pi\|_2^2} \pi - z$  and define  $v_2 = \frac{\tilde{v}_2}{\|\tilde{v}_2\|_2}$ . It is easy to verify that  $\{v_1, v_2\}$  is an orthonormal set, because

$$v_1^\top \tilde{v}_2 = \frac{1}{\|2z - \pi\|_2} (2z - \pi)^\top \tilde{v}_2 = \frac{-1}{\|2z - \pi\|_2} \left( 2 \times \frac{1 - 2\|z\|_2^2}{2 - \|\pi\|_2^2} + 2\|z\|_2^2 - \frac{1 - 2\|z\|_2^2}{2 - \|\pi\|_2^2} \cdot \|\pi\|_2^2 - 1 \right) = 0.$$

Extend this collection to an orthonormal basis  $\{v_1, v_2, \dots, v_K\}$  of  $\mathbb{R}^K$ . Take  $\lambda_1 = \frac{z^\top v_1}{\pi^\top v_1}$  and  $\lambda_2 = \frac{z^\top v_2}{\pi^\top v_2}$ . It can be verified that  $\lambda_1 > 0, \lambda_2 > 0$  (using the facts  $\|\pi\|_2 < 1, \|z\|_2 > 1$ ). For  $3 \leq i \leq K$ , choose any  $\lambda_i > 0$ . Define  $\Sigma = \sum_{i=1}^K \lambda_i v_i v_i^\top$ . Then  $\Sigma$  is a positive definite matrix and

$$\Sigma\pi = \left( \sum_{i=1}^K \lambda_i v_i v_i^\top \right) \pi = \lambda_1 v_1 (v_1^\top \pi) + \lambda_2 v_2 (v_2^\top \pi) = (z^\top v_1) v_1 + (z^\top v_2) v_2 = z,$$

as  $z \in \text{span}\{v_1, v_2\}$  and  $v_1, v_2$  are orthonormal.  $\square$

### S3.2 Scatter plot comparing the BD harmonized and cut distribution estimators in 3.1

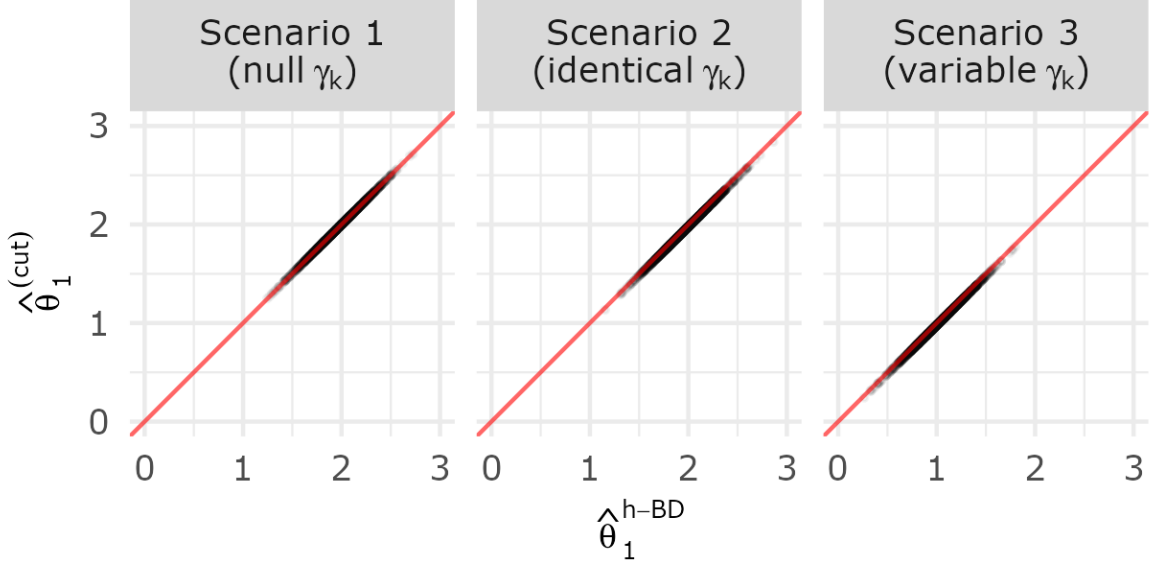

Figure S4: Scatter plots comparing the BD harmonized estimator ( $\hat{\theta}_1^{h-B}$ ) and the cut distribution estimator ( $\hat{\theta}_1^{(cut)}$ ) in the linear model simulations of paper section 3.1. The simulation settings are identical to those in Figure 4. The 45° line is drawn in red.

### S3.3 Proofs for Section 3.2 (logistic regression)

#### S3.3.1 Limiting value of $\hat{\theta}_{1:K}^{(r+e)}$ (results)

Recall that in Section 3.2  $\hat{\theta}_{1:K}^{(r+e)}$  is defined by first computing the maximum likelihood (MLE) estimates  $(\hat{\nu}_{1:K}^{(r+e)}, \hat{\eta}_{1:K}^{(r+e)}, \hat{\beta}^{(r+e)})$  of the pooled logistic regression *working* model

$$\begin{aligned} p(Y_i^{(r)} = 1 | W_i^{(r)}, T_i^{(r)}, X_i^{(r)}) &= g(\nu_{W_i^{(r)}} + \eta_{W_i^{(r)}} T_i^{(r)} + \beta^\top X_i^{(r)}), \\ p(Y_i^{(e)} = 1 | W_i^{(e)}, X_i^{(e)}) &= g(\nu_{W_i^{(e)}} + \beta^\top X_i^{(e)}), \end{aligned} \quad (29)$$

where  $g(x) = \frac{1}{1+e^{-x}}$  and the outcomes are independent, and then taking

$$\hat{\theta}_k^{(r+e)} = \frac{1}{n_{k,\cdot}^{(r)}} \sum_{i:W_i^{(r)}=k} \left[ g(\hat{\nu}_k^{(r+e)} + \hat{\eta}_k^{(r+e)} + \hat{\beta}^{(r+e)\top} X_i^{(r)}) - g(\hat{\nu}_k^{(r+e)} + \hat{\beta}^{(r+e)\top} X_i^{(r)}) \right]. \quad (31)$$

Our logistic regression results assume that the *true* data-generating outcome model is

$$\begin{aligned} p(Y_i^{(r)} = 1 | W_i^{(r)}, T_i^{(r)}, X_i^{(r)}) &= g(\nu_{W_i^{(r)}} + \eta_{W_i^{(r)}} T_i^{(r)} + \beta^\top X_i^{(r)}), \text{ and} \\ p(Y_i^{(e)} = 1 | W_i^{(e)}, X_i^{(e)}) &= g(\nu_{W_i^{(e)}} + \delta_{W_i^{(e)}} + \beta^\top X_i^{(e)}), \end{aligned} \quad (32)$$

and the outcomes are independent. Under this model, the parameter of interest is defined as

$$\begin{aligned} \theta_k &= \mathbb{E}(Y_i^{(r)} | T_i^{(r)} = 1, W_i^{(r)} = k) - \mathbb{E}(Y_i^{(r)} | T_i^{(r)} = 0, W_i^{(r)} = k) \\ &= \int_{\mathcal{X}} g(\nu_k + \eta_k + \beta^\top x) f_k^{(r)}(x) dx - \int_{\mathcal{X}} g(\nu_k + \beta^\top x) f_k^{(r)}(x) dx, \end{aligned} \quad (30)$$

where the expectation is taken over both the outcome and covariates, with  $X_i^{(r)}|W_i^{(r)} = k \stackrel{iid}{\sim} f_k^{(r)}$  and  $X_i^{(e)}|W_i^{(e)} = k \stackrel{iid}{\sim} f_k^{(e)}$  for appropriate densities  $f_k^{(r)}, f_k^{(e)}$  defined on some space  $\mathcal{X}$  and  $k = 1, \dots, K$ .

We also use the following regularity conditions for our asymptotics:

(B1) Both  $n^{(r)} \rightarrow \infty$  and  $n^{(e)} \rightarrow \infty$ . The ratios  $\frac{n_{\cdot,1}^{(r)}}{n^{(r+e)}} \rightarrow q_{1,*}^{(r)} \in (0, 1)$ ,  $\frac{n_{\cdot,0}^{(r)}}{n^{(r+e)}} \rightarrow q_{0,*}^{(r)} \in (0, 1)$ ,  $\frac{n_{\cdot,0}^{(e)}}{n^{(r+e)}} \rightarrow q_{0,*}^{(e)} \in (0, 1)$  for each  $k = 1, \dots, K$ . Also,  $\frac{n_{k,1}^{(r)}}{n_{\cdot,1}^{(r)}} \rightarrow \pi_k$ ,  $\frac{n_{k,0}^{(r)}}{n_{\cdot,0}^{(r)}} \rightarrow \pi_k$ ,  $\frac{n_{k,0}^{(e)}}{n_{\cdot,0}^{(e)}} \rightarrow \pi_k$  for each  $k = 1, \dots, K$ . (The convergence of these fractions to  $\pi_k$  in particular is primarily for simplicity).

(B3) The covariates are *iid* within each data set and subgroup  $k = 1, \dots, K$ , that is  $X_i^{(r)}|W_i^{(r)} = k \stackrel{iid}{\sim} f_k^{(r)}$  and  $X_i^{(e)}|W_i^{(e)} = k \stackrel{iid}{\sim} f_k^{(e)}$ . Here  $f_k^{(r)}$  and  $f_k^{(e)}$  are densities on  $\mathcal{X}$  such that, jointly with model (32),  $\mathbb{E} \left| Y_i \log g \left( \nu_{W_i}^* + \tau_{W_i}^* 1\{T_i = 1\} + \beta^* X_i^{(s)} \right) \right| < \infty$  for each  $i$  and  $s = r, e$ .

(B4) In model (32), the parameters  $(\nu_{1:K}, \eta_{1:K}, \beta)$  belong to a compact set.

(B5) The matrix  $\lim_{n \rightarrow \infty} \frac{1}{n^{(r+e)}} \mathbb{E}(M_1^\top D M_1)$  is invertible, where  $M_1$  is the design matrix corresponding to model (29) and  $D$  is an  $n^{(r+e)} \times n^{(r+e)}$  matrix with  $D_{ii} = g'(\nu_{W_i} + \eta_{W_i} T_i + \beta X_i)$  for  $g'(x) = \frac{d}{dx} g(x)$ .

As we will show, assumptions (B3)-(B5) imply (B2) in the text.

**Proposition S2.** *Under model (32) and assumptions (B1)-(B5), there exists a fixed vector  $\theta_{1:K}^\circ$  in  $\mathbb{R}^K$  such that*

$$\hat{\theta}_{1:K}^{(r+e)} \xrightarrow{p} \theta_{1:K}^\circ = \theta_{1:K} + B \delta_{1:K} + r_1(\delta_{1:K}), \quad (\text{S3.3.1})$$

where the remainder term  $r_1(\delta_{1:K})$  satisfies

$$\lim_{\delta_{1:K} \rightarrow 0_{K \times 1}} \frac{r_1(\delta_{1:K})}{\|\delta_{1:K}\|_1} = 0_{K \times 1}.$$

Here  $B = \frac{\partial \theta_{1:K}^\circ}{\partial \delta_{1:K}} \Big|_{(\nu_{1:K}, \eta_{1:K}, \beta, 0_{K \times 1})}$  is the Jacobian matrix of  $\theta_{1:K}^\circ$  with respect to  $\delta_{1:K}$ , evaluated at the point  $(\nu_{1:K}, \eta_{1:K}, \beta, \delta_{1:K} = 0_{K \times 1})$ . Further, we may write

$$B = \frac{\partial \theta_{1:K}^\circ}{\partial (\nu_{1:K}^\circ, \eta_{1:K}^\circ, \beta^\circ)} \Big|_{(\nu_{1:K}, \eta_{1:K}, \beta, 0_{K \times 1})} \cdot \frac{\partial (\nu_{1:K}^\circ, \eta_{1:K}^\circ, \beta^\circ)}{\partial \delta_{1:K}} \Big|_{(\nu_{1:K}, \eta_{1:K}, \beta, 0_{K \times 1})}. \quad (36)$$

**Claim S4.** *The first term in (36) is given by*

$$\begin{aligned} \frac{\partial \theta_k^\circ}{\partial \nu_k^\circ} \Big|_{(\nu_{1:K}, \eta_{1:K}, \beta, 0_{K \times 1})} &= \int_{\mathcal{X}} (g'(\nu_k + \eta_k + \beta x) - g'(\nu_k + \beta x)) f_k^{(r)}(x) dx, \\ \frac{\partial \theta_k^\circ}{\partial \eta_k^\circ} \Big|_{(\nu_{1:K}, \eta_{1:K}, \beta, 0_{K \times 1})} &= \int_{\mathcal{X}} g'(\nu_k + \eta_k + \beta x) f_k^{(r)}(x) dx, \\ \frac{\partial \theta_k^\circ}{\partial \beta^\circ} \Big|_{(\nu_{1:K}, \eta_{1:K}, \beta, 0_{K \times 1})} &= \int_{\mathcal{X}} (g'(\nu_k + \eta_k + \beta x) - g'(\nu_k + \beta x)) x f_k^{(r)}(x) dx, \end{aligned} \quad (\text{S3.3.2})$$

for  $k = 1, \dots, K$ , where we use the notation  $g'(x) = \frac{d}{dx} g(x)$ . All other partial derivatives in the first term of (36) are 0.

The second term in (36) is given by

$$\frac{\partial (\nu_{1:K}^\circ, \eta_{1:K}^\circ, \beta^\circ)}{\partial \delta_{1:K}} \Big|_{(\nu_{1:K}, \eta_{1:K}, \beta, 0_{K \times 1})} = \lim_{n \rightarrow \infty} \left[ \mathbb{E} \left( M_1^\top D M_1 \right) \right]^{-1} \mathbb{E} \left( M_1^\top D M_2 \right), \quad (\text{S3.3.3})$$

where

- $M_1$  is the  $n^{(r+e)} \times (2K + d)$  design matrix for model (29), containing columns corresponding to  $(\nu_{1:K}, \eta_{1:K}, \beta)$ ,

- The full design matrix is  $[M_1, M_2]$ , with the  $n^{(r+e)} \times K$  matrix  $M_2$  containing columns corresponding to  $\delta_{1:K}$ , and
- $D$  is a diagonal  $n^{(r+e)} \times n^{(r+e)}$  matrix with  $D_{ii} = g'(\nu_{W_i} + \eta_{W_i} T_i + \beta X_i)$ .

**Remark S1.** The Jacobians in  $B$ ,  $\frac{\partial \theta_{1:K}^\circ}{\partial(\nu_{1:K}^\circ, \eta_{1:K}^\circ, \beta^\circ)}$  and  $\frac{\partial(\nu_{1:K}^\circ, \eta_{1:K}^\circ, \beta^\circ)}{\partial \delta_{1:K}}$  depend on the unknown parameters  $(\nu_{1:K}, \eta_{1:K}, \beta)$  and the unknown RCT covariate distributions  $f_k^{(r)}$  for  $k = 1, \dots, K$ . Therefore  $B$  is unobserved. However, we can use a plug-in estimation strategy to estimate  $B$  consistently. In particular, suppose that  $(\hat{\nu}_{1:K}, \hat{\eta}_{1:K}, \hat{\beta})$  is a consistent estimator of  $(\nu_{1:K}, \eta_{1:K}, \beta)$  and  $\hat{f}_k^{(r)}$  is the empirical distribution of  $X_i^{(r)} | W_i^{(r)} = k$ . Plugging these estimators into (S3.3.2) gives a consistent estimator of  $\frac{\partial \theta_{1:K}^\circ}{\partial(\nu_{1:K}^\circ, \eta_{1:K}^\circ, \beta^\circ)}$ . Similarly, if the diagonal matrix  $\hat{D}$  is defined as  $\hat{D}_{ii} = g'(\hat{\nu}_{W_i} + \hat{\eta}_{W_i} T_i + \hat{\beta} X_i)$  then  $(M_1^\top \hat{D} M_1)^{-1} (M_1^\top \hat{D} M_2)$  is a consistent estimator of  $\frac{\partial(\nu_{1:K}^\circ, \eta_{1:K}^\circ, \beta^\circ)}{\partial \delta_{1:K}}$  in (S3.3.3). Plugging both into (36) gives a consistent estimator  $\hat{B}$  of  $B$ .

**Remark S2.** Proposition S2 and Claim S4 also hold for data generated from generalized linear models if  $g$  is appropriately changed in each expression. In particular, suppose that the density of  $Y_i^{(r)}, Y_i^{(e)}$  is from an overdispersed exponential family (not necessarily binomial) and  $g$  is the canonical (and continuously differentiable) function such that

$$\begin{aligned} \mathbb{E}\left(Y_i^{(r)} | W_i^{(r)}, T_i^{(r)}, X_i^{(r)}\right) &= g\left(\nu_{W_i^{(r)}} + \eta_{W_i^{(r)}} T_i^{(r)} + \beta^\top X_i^{(r)}\right), \\ \mathbb{E}\left(Y_i^{(e)} | W_i^{(e)}, X_i^{(e)}\right) &= g\left(\nu_{W_i^{(e)}} + \delta_{W_i^{(e)}} + \beta^\top X_i^{(e)}\right). \end{aligned}$$

For example, we might have a Poisson count outcome model with log link function. Then Proposition S2 and Claim S4 still hold, with  $g(x) = e^x$  instead of  $g(x) = \frac{1}{1+e^{-x}}$ . The proofs are identical, except that  $\mathcal{O}_n$  and  $\mathcal{L}$  (see below) must have the appropriate form for the generalized linear model (because of the canonical link function this does not affect later steps in the derivation).

### S3.3.2 Limiting value of $\hat{\theta}_{1:K}^{(r+e)}$ (proofs)

**Proof (Proposition S2).** To derive the result we proceed in two steps. First, we show that the MLE  $(\hat{\nu}_{1:K}^{(r+e)}, \hat{\eta}_{1:K}^{(r+e)}, \hat{\beta}^{(r+e)})$  of model (29) converges in probability to some limit  $(\nu_{1:K}^\circ, \eta_{1:K}^\circ, \beta^\circ)$ . As a result  $\hat{\theta}_{1:K}^{(r+e)}$  converges in probability to a limit  $\theta_{1:K}^\circ$ . Then we show that  $\theta_{1:K}^\circ$  has the desired form.

For ease of exposition, we introduce notation for the outcomes that is slightly different from what is used in the rest of the paper. Let  $Y_{i,k,1}^{(r)}$  denote the outcome of the  $i^{th}$  individual in the RCT treatment group and subgroup  $k$ , and let  $X_{i,k,1}^{(r)}$  denote the corresponding covariate. Similarly define  $Y_{i,k,0}^{(r)}, X_{i,k,0}^{(r)}, Y_{i,k,0}^{(e)}, X_{i,k,0}^{(e)}$ .

To see the convergence of  $(\hat{\nu}_{1:K}^{(r+e)}, \hat{\eta}_{1:K}^{(r+e)}, \hat{\beta}^{(r+e)})$ , note that by definition they maximize the following objective function with respect to  $(\nu'_{1:K}, \eta'_{1:K}, \beta')$ :

$$\begin{aligned} \mathcal{O}_n &:= \frac{1}{n^{(r+e)}} \sum_{k=1}^K \sum_i \left[ Y_{i,k,1}^{(r)} \ln \left( g(\nu'_k + \eta'_k + \beta' X_{i,k,1}^{(r)}) \right) + \left( 1 - Y_{i,k,1}^{(r)} \right) \ln \left( 1 - g(\nu'_k + \eta'_k + \beta' X_{i,k,1}^{(r)}) \right) \right] + \\ &\quad \frac{1}{n^{(r+e)}} \sum_{k=1}^K \sum_i \left[ Y_{i,k,0}^{(r)} \ln \left( g(\nu'_k + \beta' X_{i,k,0}^{(r)}) \right) + \left( 1 - Y_{i,k,0}^{(r)} \right) \ln \left( 1 - g(\nu'_k + \beta' X_{i,k,0}^{(r)}) \right) \right] + \\ &\quad \frac{1}{n^{(r+e)}} \sum_{k=1}^K \sum_i \left[ Y_{i,k,0}^{(e)} \ln \left( g(\nu'_k + \beta' X_{i,k,0}^{(e)}) \right) + \left( 1 - Y_{i,k,0}^{(e)} \right) \ln \left( 1 - g(\nu'_k + \beta' X_{i,k,0}^{(e)}) \right) \right]. \end{aligned}$$

Here  $\mathcal{O}_n$  is the observed log likelihood of the working model (29), normalized by the factor  $\frac{1}{n^{(r+e)}}$ .

By the law of large numbers and assumptions (B3)-(B1),  $\mathcal{O}_n$  converges in probability to the following function:

$$\begin{aligned}\mathcal{L} = & q_{1,*}^{(r)} \sum_{k=1}^K \pi_k \mathbb{E} \left[ h \left( \nu_k + \eta_k + \beta X_{1,k,1}^{(r)}, \nu'_k + \eta'_k + \beta' X_{1,k,1}^{(r)} \right) \right] + \\ & q_{0,*}^{(r)} \sum_{k=1}^K \pi_k \mathbb{E} \left[ h \left( \nu_k + \beta X_{1,k,0}^{(r)}, \nu'_k + \beta' X_{1,k,0}^{(r)} \right) \right] + \\ & q_{0,*}^{(e)} \sum_{k=1}^K \pi_k \mathbb{E} \left[ h \left( \nu_k + \delta_k + \beta X_{1,k,0}^{(e)}, \nu'_k + \beta' X_{1,k,0}^{(e)} \right) \right],\end{aligned}$$

where  $h(a, b) := g(a) \ln g(b) + (1 - g(a)) \ln(1 - g(b)) = g(a) \cdot b + \ln(1 - g(b))$  and  $g(x) = \frac{1}{1+e^{-x}}$ . Here we emphasize that  $(\nu_{1:K}, \eta_{1:K}, \beta, \delta_{1:K})$  are the parameters of the true data-generating model (32) and  $(\nu'_{1:K}, \eta'_{1:K}, \beta')$  are the parameters of the working model (29) used for MLE to get  $\hat{\theta}_{1:K}^{(r+e)}$ . Intuitively,  $\mathcal{L}$  is the limit of the expectation of the working log likelihood  $\mathcal{O}_n$ , where expectation is taken with respect to the true outcome model (32) and the covariate model (B3). We define  $(\nu_{1:K}^\circ, \eta_{1:K}^\circ, \beta^\circ)$  as the value of  $(\nu'_{1:K}, \eta'_{1:K}, \beta')$  that maximizes  $\mathcal{L}$ .

Because  $\mathcal{O}_n \xrightarrow{p} \mathcal{L}$ , Theorem 2.1 of White (1981) (which holds because of assumption (B4)) implies that the maximizer of  $\mathcal{O}_n$  converges in probability to the maximizer of  $\mathcal{L}$ , i.e.  $(\hat{\nu}_{1:K}^{(r+e)}, \hat{\eta}_{1:K}^{(r+e)}, \hat{\beta}^{(r+e)}) \xrightarrow{p} (\nu_{1:K}^\circ, \eta_{1:K}^\circ, \beta^\circ)$ .

To see how this implies the convergence of  $\hat{\theta}_{1:K}^{(r+e)}$ , recall that

$$\hat{\theta}_k^{(r+e)} = \frac{1}{n_{k,\cdot}^{(r)}} \sum_{i: W_i^{(r)} = k} \left[ g \left( \hat{\nu}_k^{(r+e)} + \hat{\eta}_k^{(r+e)} + \hat{\beta}^{(r+e)\top} X_i^{(r)} \right) - g \left( \hat{\nu}_k^{(r+e)} + \hat{\beta}^{(r+e)\top} X_i^{(r)} \right) \right]. \quad (31)$$

Since (31) is a continuous function of  $(\hat{\nu}_{1:K}^{(r+e)}, \hat{\eta}_{1:K}^{(r+e)}, \hat{\beta}^{(r+e)})$ , the continuous mapping theorem combined with assumption (B3) implies that

$$\hat{\theta}_{1:K}^{(r+e)} \xrightarrow{p} \theta_k^\circ = \int_{\mathcal{X}} (g(\nu_k^\circ + \eta_k^\circ + \beta^\circ x) - g(\nu_k^\circ + \beta^\circ x)) f_k(x) dx.$$

Finally, we show that  $\theta_{1:K}^\circ$  has the desired form in (S3.3.1). When  $\delta_{1:K} = 0_{K \times 1}$ , the MLE model (29) is correctly specified and therefore  $(\nu_{1:K}^\circ, \eta_{1:K}^\circ, \beta^\circ) = (\nu_{1:K}, \eta_{1:K}, \beta)$  by standard maximum likelihood arguments. This also implies that  $\theta_{1:K}^\circ = \theta_{1:K}$  when  $\delta_{1:K} = 0_{K \times 1}$ . Thus using Taylor's theorem at the point  $\delta_{1:K} = 0_{K \times 1}$ , one gets

$$\theta_{1:K}^\circ = \theta_{1:K} + B \delta_{1:K} + r_1(\delta_{1:K}), \quad (\text{S3.3.1})$$

where

$$B = \left. \frac{\partial \theta_{1:K}^\circ}{\partial \delta_{1:K}} \right|_{(\nu_{1:K}, \eta_{1:K}, \beta, 0_{K \times 1})}$$

is the Jacobian matrix of  $\theta_{1:K}^\circ$  with respect to  $\delta_{1:K}$ , evaluated at the point  $(\nu_{1:K}, \eta_{1:K}, \beta, \delta_{1:K} = 0_{K \times 1})$ , and the remainder term  $r_1(\delta_{1:K})$  satisfies

$$\lim_{\delta_{1:K} \rightarrow 0_{K \times 1}} \frac{r_1(\delta_{1:K})}{\|\delta_{1:K}\|_1} = 0_{K \times 1}.$$

Using the chain rule, we may write

$$B = \left. \frac{\partial \theta_{1:K}^\circ}{\partial (\nu_{1:K}, \eta_{1:K}, \beta^\circ)} \right|_{(\nu_{1:K}, \eta_{1:K}, \beta, 0_{K \times 1})} \cdot \left. \frac{\partial (\nu_{1:K}, \eta_{1:K}, \beta^\circ)}{\partial \delta_{1:K}} \right|_{(\nu_{1:K}, \eta_{1:K}, \beta, 0_{K \times 1})}. \quad (36)$$

□

**Proof (Claim S4).** To see that the Jacobian  $\frac{\partial \theta_{1:K}^\circ}{\partial (\nu_{1:K}^\circ, \eta_{1:K}^\circ, \beta^\circ)} \Big|_{(\nu_{1:K}, \eta_{1:K}, \beta, 0_{K \times 1})}$  has the desired form, first recall that when  $\delta_{1:K} = 0_{K \times 1}$

$$\theta_k^\circ = \int_{\mathcal{X}} (g(\nu_k + \eta_k + \beta x) - g(\nu_k + \beta x)) f_k(x) dx.$$

Then we have

$$\begin{aligned} \frac{\partial \theta_k^\circ}{\partial \nu_k^\circ} \Big|_{(\nu_{1:K}, \eta_{1:K}, \beta, 0_{K \times 1})} &= \int_{\mathcal{X}} (g'(\nu_k + \eta_k + \beta x) - g'(\nu_k + \beta x)) f_k^{(r)}(x) dx, \\ \frac{\partial \theta_k^\circ}{\partial \eta_k^\circ} \Big|_{(\nu_{1:K}, \eta_{1:K}, \beta, 0_{K \times 1})} &= \int_{\mathcal{X}} g'(\nu_k + \eta_k + \beta x) f_k^{(r)}(x) dx, \\ \frac{\partial \theta_k^\circ}{\partial \beta^\circ} \Big|_{(\nu_{1:K}, \eta_{1:K}, \beta, 0_{K \times 1})} &= \int_{\mathcal{X}} (g'(\nu_k + \eta_k + \beta x) - g'(\nu_k + \beta x)) x f_k^{(r)}(x) dx, \end{aligned}$$

by interchanging the derivatives and integrals (justified by the Leibniz integral rule since  $g'$  is continuous and the parameter space is compact).

To derive the form of the Jacobian  $\frac{\partial (\nu_{1:K}^\circ, \eta_{1:K}^\circ, \beta^\circ)}{\partial \delta_{1:K}} \Big|_{(\nu_{1:K}, \eta_{1:K}, \beta, 0_{K \times 1})}$ , we use the following strategy. Recall that  $(\nu_{1:K}^\circ, \eta_{1:K}^\circ, \beta^\circ)$  are defined as the maximizers of  $\mathcal{L}$ . This implies that they are the solutions to the system of equations  $\frac{\partial \mathcal{L}}{\partial (\nu'_{1:K}, \eta'_{1:K}, \beta')} \Big|_{(\nu_{1:K}^\circ, \eta_{1:K}^\circ, \beta^\circ)} = 0_{(2K+d) \times 1}$ . Although this system has no analytic solution for  $(\nu_{1:K}^\circ, \eta_{1:K}^\circ, \beta^\circ)$ , we can still use it to compute the Jacobian  $\frac{\partial (\nu_{1:K}^\circ, \eta_{1:K}^\circ, \beta^\circ)}{\partial \delta_{1:K}} \Big|_{(\nu_{1:K}, \eta_{1:K}, \beta, 0_{K \times 1})}$  by applying the implicit function theorem, as we describe next.

Recall that the implicit function theorem says generically, that if  $G(\mathbf{x}, \mathbf{y})$  is a continuously differentiable function and with  $G(\mathbf{a}, \mathbf{b}) = 0_{m \times 1}$  at some point  $(\mathbf{a}, \mathbf{b})$ , then locally around this point  $\mathbf{y}$  is (implicitly) a function of  $\mathbf{x}$  and we can compute the derivative

$$\frac{\partial \mathbf{y}}{\partial \mathbf{x}} \Big|_{\mathbf{x}=\mathbf{a}} = - \frac{\partial G}{\partial \mathbf{y}} \Big|_{\mathbf{x}=\mathbf{a}, \mathbf{y}=\mathbf{b}}^{-1} \cdot \frac{\partial G}{\partial \mathbf{x}} \Big|_{\mathbf{x}=\mathbf{a}, \mathbf{y}=\mathbf{b}}, \quad (\text{S3.3.4})$$

as long as  $\frac{\partial G}{\partial \mathbf{y}} \Big|_{\mathbf{x}=\mathbf{a}, \mathbf{y}=\mathbf{b}}$  is invertible.

To apply the implicit function theorem, we use the notation  $\mathbf{x} = (\nu_{1:K}, \eta_{1:K}, \beta, \delta_{1:K})$  for the parameters of the true data-generating model (32),  $\mathbf{y} = (\nu'_{1:K}, \eta'_{1:K}, \beta')$  for the parameters of the working model (29), and  $G(\mathbf{x}, \mathbf{y}) = \frac{\partial \mathcal{L}}{\partial \mathbf{y}}$  for the gradient of  $\mathcal{L}$  with respect to  $\mathbf{y}$ . When  $\mathbf{y} = (\nu_{1:K}^\circ, \eta_{1:K}^\circ, \beta^\circ)$  we have  $G(\mathbf{x}, \mathbf{y}) = 0_{(2K+d) \times 1}$ . Recall that we wish to evaluate  $\frac{\partial (\nu_{1:K}^\circ, \eta_{1:K}^\circ, \beta^\circ)}{\partial \delta_{1:K}}$  when the true parameters are  $\mathbf{x} = \mathbf{a} = (\nu_{1:K}, \eta_{1:K}, \beta, 0_{K \times 1})$ . In this case the limiting parameters are  $(\nu_{1:K}^\circ, \eta_{1:K}^\circ, \beta^\circ) = \mathbf{b} = (\nu_{1:K}, \eta_{1:K}, \beta)$  by standard MLE arguments (i.e. working model is correctly specified so the MLE converges to the true parameters). Thus computing (S3.3.4) gives us  $\frac{\partial (\nu_{1:K}^\circ, \eta_{1:K}^\circ, \beta^\circ)}{\partial \delta_{1:K}} \Big|_{(\nu_{1:K}, \eta_{1:K}, \beta, 0_{K \times 1})}$  as desired.

The Jacobians in (S3.3.4) are

$$\begin{aligned} - \frac{\partial G}{\partial \mathbf{y}} \Big|_{\mathbf{x}=\mathbf{a}, \mathbf{y}=\mathbf{b}}^{-1} &= \lim_{n \rightarrow \infty} \frac{1}{n^{(r+e)}} \mathbb{E}(M_1^\top D M_1) \quad , \text{ and} \\ \frac{\partial G}{\partial \mathbf{x}} \Big|_{\mathbf{x}=\mathbf{a}, \mathbf{y}=\mathbf{b}} &= \lim_{n \rightarrow \infty} \frac{1}{n^{(r+e)}} \mathbb{E}(M_1^\top D M_2). \end{aligned} \quad (\text{S3.3.5})$$

Heuristically, these Jacobians are limiting values of the expected Fisher information matrices of model (29), since  $\mathcal{L}$  is the limit of the observed log likelihood and  $G$  is its gradient (essentially, the limit of the score function). The Fisher information matrices have the familiar form for GLMs. These formulae

can also be found by tedious direct calculation of the derivatives of  $G$  and using linear algebra to simplify. □

### S3.3.3 Proof of Proposition 5

**Proposition 6.** *If assumption (B1) holds, and the sequence of designs ensures that for any value of  $\delta_{1:k}$  in model (32)*

$$(A3) \quad \hat{\theta}^{(r)} \xrightarrow{p} \pi^\top \theta_{1:K},$$

$$(A4) \quad \hat{\theta}_{1:K}^{(r+e)} \xrightarrow{p} \theta_{1:K} + B\delta_{1:K} + r_1(\delta_{1:K}), \text{ where } r_1(\delta_{1:K}) \text{ satisfies expression (35), and}$$

$$(A5) \quad \hat{\Sigma} \xrightarrow{p} \Sigma, \text{ where } \Sigma \text{ is a positive-definite } K \times K \text{ matrix,}$$

then

$$\hat{\theta}_{1:K}^h \xrightarrow{p} \theta_{1:K} + \left( I_K - u\pi^\top \right) B\delta_{1:K} + r_2(\delta_{1:K}),$$

where the approximation error  $r_2(\delta_{1:K})$  satisfies

$$\lim_{\delta_{1:K} \rightarrow 0_{K \times 1}} \frac{r_2(\delta_{1:K})}{\|\delta_{1:K}\|_1} = 0_{K \times 1}.$$

*Proof.* Because  $\hat{\theta}_{1:K}^h$  is a continuous function of  $\hat{\theta}_{1:K}^{(r+e)}$ ,  $\hat{\theta}^{(r)}$ , and  $\hat{\Sigma}$ , assumptions (B3)-(B5) and the continuous mapping theorem imply that

$$\begin{aligned} \hat{\theta}_{1:K}^h &\xrightarrow{p} \theta_{1:K} + B\delta_{1:K} + r_1(\delta_{1:K}) + u \left[ \pi^\top \theta_{1:K} - \pi^\top (\theta_{1:K} + B\delta_{1:K} + r_1(\delta_{1:K})) \right] \\ &= \theta_{1:K} + B\delta_{1:K} + r_1(\delta_{1:K}) - u\pi^\top (B\delta_{1:K} + r_1(\delta_{1:K})) \\ &= \theta_{1:K} + B\delta_{1:K} - u\pi^\top B\delta_{1:K} + o(\|\delta_{1:K}\|_1) \\ &= \theta_{1:K} + \left( I_K - u\pi^\top \right) B\delta_{1:K} + r_2(\delta_{1:K}), \end{aligned}$$

where we define  $r_2(\delta_{1:K}) = (I_K - u\pi^\top) r_1(\delta_{1:K})$ . By assumption (B4),  $r_2(\delta_{1:K})$  satisfies

$$\lim_{\delta_{1:K} \rightarrow 0_{K \times 1}} \frac{r_2(\delta_{1:K})}{\|\delta_{1:K}\|_1} = 0_{K \times 1}.$$

□

## S3.4 Simulation details for Section 3.2

### S3.4.1 Taking $\Sigma$ as a variance estimate

In defining  $\hat{\theta}_{1:K}^h$ , one strategy to choose  $\Sigma$  is to take it as an estimate of the sampling variance  $\text{Var}(\hat{\theta}_{1:K}^{(r+e)})$ . For the logistic regression setting we can estimate  $\text{Var}(\hat{\theta}_{1:K}^{(r+e)})$  with the delta method as follows:

1. Let  $\hat{V}_{\nu, \eta, \beta}$  be an estimate of the variance-covariance matrix of  $(\hat{\nu}_{1:K}^{(r+e)}, \hat{\eta}_{1:K}^{(r+e)}, \hat{\beta}^{(r+e)})$ . For instance, this may be an observed Fisher information matrix calculation as done by the `glm` function in R.
2. Compute  $W = \frac{\partial \theta_{1:K}}{\partial (\nu_{1:K}, \eta_{1:K}, \beta)} \Big|_{(\hat{\nu}_{1:K}^{(r+e)}, \hat{\eta}_{1:K}^{(r+e)}, \hat{\beta}^{(r+e)})}$  as in (S3.3.2).
3. Take  $\Sigma = W \hat{V}_{\nu, \eta, \beta} W^\top$ .

### S3.4.2 Simulation settings

For the simulations in Section 3.2 we generate outcomes from the logistic regression model

$$\begin{aligned} p\left(Y_i^{(r)} = 1 | W_i^{(r)}, T_i^{(r)}, X_i^{(r)}\right) &= g\left(\nu_{W_i^{(r)}} + \eta_{W_i^{(r)}} T_i^{(r)} + \beta^\top X_i^{(r)}\right), \text{ and} \\ p\left(Y_i^{(e)} = 1 | W_i^{(e)}, X_i^{(e)}\right) &= g\left(\nu_{W_i^{(e)}} + \delta_{W_i^{(e)}} + \beta^\top X_i^{(e)}\right), \end{aligned} \quad (32)$$

where  $g(x) = \frac{1}{1+e^{-x}}$ , and the outcomes are independent. As before we generated a single covariate (i.e.  $d = 1$ ),  $X_i^{(r)} \stackrel{iid}{\sim} N(0, 1)$  for  $i = 1, \dots, n^{(r)}$  in the RCT and  $X_i^{(e)} \stackrel{iid}{\sim} N(2, 1)$  for  $i = 1, \dots, n^{(e)}$  in the EC.

We consider  $K = 5$  subgroups and use the parameters  $\nu_{1:K} = (0, \dots, 0)$ ,  $\eta_{1:K} = (1, 1, 0.5, 0, 0)$ ,  $\beta = 0.2$ . For Figure 5, we take  $\delta_{1:K} = (\delta, \dots, \delta)$  for  $\delta \in [-1, 1]$ . For Figure S5 we take  $\delta_{1:K} = (\delta + 0.5, \delta - 0.5, \delta + 0.5, \delta - 0.5, \delta + 0.5, \delta + 0.5)$  for  $\delta \in [-1, 1]$ . The data set sample sizes are  $n^{(r)} = 200$ ,  $n^{(e)} = 500$ , with equal subgroup proportions  $\pi = (1/5, \dots, 1/5)$  in both the RCT and EC. The RCT has a randomization ratio of 1:1, and randomization is stratified by subgroup as in Section 2.2. For each scenario (each value of  $\delta_{1:K}$ ) we generate 2000 simulated studies.

### S3.4.3 Version of Figure 5 with $\delta_{1:K}$ varying across subgroup

Figure S5 is analogous to Figure 5 in the text but with  $\delta_{1:K}$  varying across subgroups, as described in the previous subsection. Unlike before, the harmonized estimator is now moderately biased, though in terms of RMSE it still outperforms the RCT-only estimator, as well as the pooled estimator when  $\delta_1$  is large. There is slightly less concordance between the two versions of the harmonized estimator ( $\hat{\theta}_1^{h-B}$  vs.  $\hat{\theta}_1^{h-V}$  in Panel C) compared to when  $\delta_{1:K} = 1_{K \times 1}$  (Figure 5), but their performance is very similar (Panel B).

## S3.5 Computation of $B$ for Section 3.3

By arguments nearly identical to before, it can be shown that when  $\hat{\theta}_{1:K}^{(r+e)}$  is estimated by *weighted* maximum likelihood as in Section 3.3, Proposition S2 and Claim S4 still hold with minor variations. In particular, the  $B$  matrix in the Taylor approximation  $\theta_{1:K}^\circ - \theta_{1:K} \approx B\delta_{1:K}$  follows (S3.3.2) exactly and a weighted version of (S3.3.3), with

$$\left. \frac{\partial(\nu_{1:K}^\circ, \eta_{1:K}^\circ, \beta^\circ)}{\partial \delta_{1:K}} \right|_{(\nu_{1:K}, \eta_{1:K}, \beta, 0_{K \times 1})} = \lim_{n \rightarrow \infty} \left[ \mathbb{E} \left( M_1^\top W D M_1 \right) \right]^{-1} \mathbb{E} \left( M_1^\top W D M_2 \right),$$

where  $W$  is a diagonal matrix containing the weights used for each individual. Then we can estimate  $B$  consistently the same way as in Remark S1.

## S3.6 Generalized linear models

*Treatment effect estimates before harmonization.* We consider  $\hat{\theta}_{1:K}^{(r+e)}$  based on a GLM. In particular,  $\hat{\theta}_{1:K}^{(r+e)}$  is obtained (MLE or propensity score weighted MLE) through a model with conditional means

$$\begin{aligned} E\left(Y_i^{(r)} | W_i^{(r)}, T_i^{(r)}, X_i^{(r)}\right) &= g\left(\nu_{W_i^{(r)}} + \eta_{W_i^{(r)}} T_i^{(r)} + \beta^\top X_i^{(r)}\right), \text{ and} \\ E\left(Y_i^{(e)} | W_i^{(e)}, X_i^{(e)}\right) &= g\left(\nu_{W_i^{(e)}} + \beta^\top X_i^{(e)}\right), \end{aligned} \quad (S3.6.1)$$

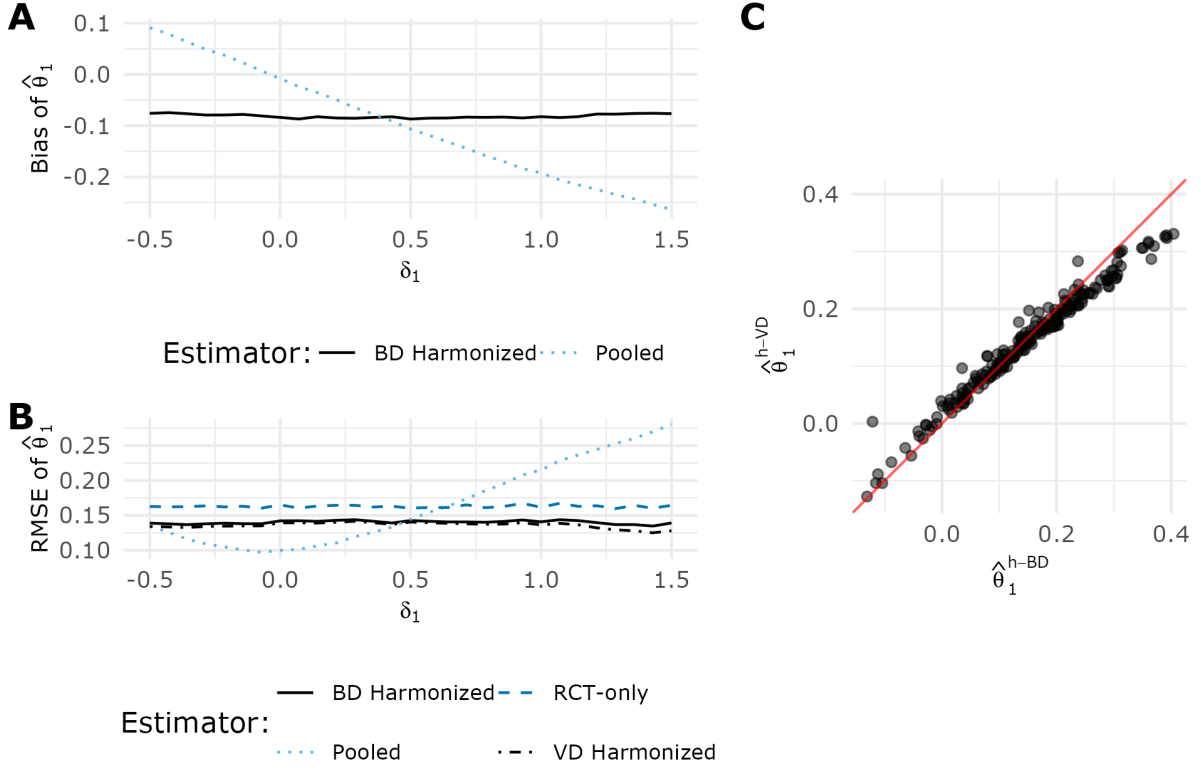

Figure S5: Logistic regression and harmonized estimates. The results are based on 2000 replicates per scenario. Panel A shows the bias when we estimate  $\theta_1$  using the pooled estimator and the BD harmonized estimator as a function of  $\delta_1$ . Panel B shows the root mean squared error of four estimators. Panel C is a scatter plot comparing the BD harmonized (denoted  $\hat{\theta}_1^{h-BD}$ ) estimator and the VD harmonized (indicated as  $\hat{\theta}_1^{h-VD}$ ) estimator across a random subsample of 200 replicates with  $\delta = 1_{K \times 1}$ . The true value was  $\theta_1 = 0.23$ .

where  $g(x)$  is continuously differentiable and monotone. In the GLM, the outcomes  $Y_i^{(r)}$  and  $Y_i^{(e)}$  are independently distributed according to an exponential family (e.g., Poisson) distribution (for all  $i$ ). Let  $\ell_i^{(r)}$  and  $\ell_i^{(e)}$  be the GLM log-likelihood contributions of  $Y_i^{(r)}$  and  $Y_i^{(e)}$  respectively. We compute the estimates  $\left(\hat{\nu}_{1:K}^{(r+e)}, \hat{\eta}_{1:K}^{(r+e)}, \hat{\beta}^{(r+e)}\right)$  that maximize the weighted log-likelihood

$$\tilde{\mathcal{O}}_n = \frac{1}{n^{(r+e)}} \sum_{i=1}^{n^{(r)}} w_i^{(r)} \ell_i^{(r)} + \frac{1}{n^{(r+e)}} \sum_{i=1}^{n^{(e)}} w_i^{(e)} \ell_i^{(e)}.$$

Here  $w_i^{(r)} = 1$  and  $w_i^{(e)}$  are propensity score weights as described in Section 3.3. Finally,

$$\hat{\theta}_k^{(r+e)} = \frac{1}{n_{k,\cdot}^{(r)}} \sum_{i: W_i^{(r)}=k} \left[ g\left(\hat{\nu}_k^{(r+e)} + \hat{\eta}_k^{(r+e)} + \hat{\beta}^{(r+e)\top} X_i^{(r)}\right) - g\left(\hat{\nu}_k^{(r+e)} + \hat{\beta}^{(r+e)\top} X_i^{(r)}\right) \right]. \quad (\text{S3.6.2})$$

*Unknown data distribution.* Similar to Section 3.2, our results (Proposition S2 and Claim S5 below) build on the assumption that the *true* data-generating outcome model is a GLM based on the same exponential family and link function, but with conditional means

$$\begin{aligned} E\left(Y_i^{(r)} | W_i^{(r)}, T_i^{(r)}, X_i^{(r)}\right) &= g\left(\nu_{W_i^{(r)}} + \eta_{W_i^{(r)}} T_i^{(r)} + \beta^\top X_i^{(r)}\right), \\ E\left(Y_i^{(e)} | W_i^{(e)}, X_i^{(e)}\right) &= g\left(\nu_{W_i^{(e)}} + \delta_{W_i^{(e)}} + \beta^\top X_i^{(e)}\right). \end{aligned} \quad (\text{S3.6.3})$$

The parameter of interest is

$$\begin{aligned}\theta_k &= \mathbb{E} \left( Y_i^{(r)} | T_i^{(r)} = 1, W_i^{(r)} = k \right) - \mathbb{E} \left( Y_i^{(r)} | T_i^{(r)} = 0, W_i^{(r)} = k \right) \\ &= \int_{\mathcal{X}} g \left( \nu_k + \eta_k + \beta^\top x \right) f_k^{(r)}(x) dx - \int_{\mathcal{X}} g \left( \nu_k + \beta^\top x \right) f_k^{(r)}(x) dx,\end{aligned}\tag{S3.6.4}$$

with  $X_i^{(r)} | W_i^{(r)} = k \stackrel{iid}{\sim} f_k^{(r)}$  and  $X_i^{(e)} | W_i^{(e)} = k \stackrel{iid}{\sim} f_k^{(e)}$ ,  $k = 1, \dots, K$ .

To prove the subsequent theoretical results, we work with the following mild and convenient technical conditions:

(C1) Both  $n^{(r)} \rightarrow \infty$  and  $n^{(e)} \rightarrow \infty$ . The ratios  $\frac{n_{\cdot,1}^{(r)}}{n^{(r+e)}} \rightarrow q_{1,*}^{(r)} \in (0, 1)$ ,  $\frac{n_{\cdot,0}^{(r)}}{n^{(r+e)}} \rightarrow q_{0,*}^{(r)} \in (0, 1)$ ,  $\frac{n_{\cdot,0}^{(e)}}{n^{(r+e)}} \rightarrow q_{0,*}^{(e)} \in (0, 1)$  for each  $k = 1, \dots, K$ . Also,  $\frac{n_{k,1}^{(r)}}{n_{\cdot,1}^{(r)}} \rightarrow \pi_k$ ,  $\frac{n_{k,0}^{(r)}}{n_{\cdot,0}^{(r)}} \rightarrow \pi_k$ ,  $\frac{n_{k,0}^{(e)}}{n_{\cdot,0}^{(e)}} \rightarrow \pi_k$  for each  $k = 1, \dots, K$ . The convergence of these fractions to  $\pi_k$  simplifies the derivation of Claim S5.

(C2) There exist sequences of limiting weights  $w_{i,*}^{(s)}$  for  $s = r, e$  such that  $\left( w_i^{(s)} - w_{i,*}^{(s)} \right) \ell_i^{(e)} \xrightarrow{p} 0$  as  $n^{(r+e)} \rightarrow \infty$ . Here  $w_i^{(s)}$  may be a function of all  $n^{(r+e)}$  individual pre-treatment covariate vectors and outcomes.

(C3) The covariates are *iid* within each data set and subgroup  $k = 1, \dots, K$ , that is  $X_i^{(r)} | W_i^{(r)} = k \stackrel{iid}{\sim} f_k^{(r)}$  and  $X_i^{(e)} | W_i^{(e)} = k \stackrel{iid}{\sim} f_k^{(e)}$ . Here  $f_k^{(r)}$  and  $f_k^{(e)}$  are densities on  $\mathcal{X}$  such that, jointly with model (S3.6.3),  $E \left| w_{i,*}^{(s)} \ell_i^{(s)} \right| < \infty$  for each  $i$  and  $s = r, e$ , and for all parameter values in (S3.6.3).

(C4) In model (S3.6.3) the parameters  $(\nu_{1:K}, \eta_{1:K}, \beta)$  belong to a compact set.

(C5) The matrix  $\lim_{n \rightarrow \infty} \frac{1}{n^{(r+e)}} \mathbb{E}(M_1^\top D M_1)$  is invertible. Here  $M_1$  is the design matrix corresponding to model (S3.6.1). Also,  $D$  is an  $n^{(r+e)} \times n^{(r+e)}$  diagonal matrix with  $D_{ii} = w_i g'(\nu_{W_i} + \eta_{W_i} T_i + \beta X_i)$  for  $g'(x) = \frac{d}{dx} g(x)$  and  $w_i = 1$  for RCT patients and  $w_i$  equal to the propensity score weight for EC patients. This condition is simply a weighted version of (B5 for Proposition S1).

Together, assumptions (C2)-(C5) are used to ensure that  $\left( \hat{\nu}_{1:K}^{(r+e)}, \hat{\eta}_{1:K}^{(r+e)}, \hat{\beta}^{(r+e)}, \hat{\theta}_{1:K}^{(r+e)} \right)$  converges in probability to some point  $(\nu_{1:K}^\circ, \eta_{1:K}^\circ, \beta^\circ, \theta_{1:K}^\circ)$  (which might differ from the true  $(\nu_{1:K}, \eta_{1:K}, \beta, \theta_{1:K})$ ).

**Proposition S3.** *Under model (S3.6.3) and assumptions (C1)-(C5), there exists a fixed vector  $\theta_{1:K}^\circ$  in  $\mathbb{R}^K$  such that*

$$\hat{\theta}_{1:K}^{(r+e)} \xrightarrow{p} \theta_{1:K}^\circ = \theta_{1:K} + B \delta_{1:K} + r_1(\delta_{1:K}),\tag{S3.6.5}$$

where the remainder term  $r_1(\delta_{1:K})$  satisfies

$$\lim_{\delta_{1:K} \rightarrow 0_{K \times 1}} \frac{r_1(\delta_{1:K})}{\|\delta_{1:K}\|_1} = 0_{K \times 1}.$$

Here  $B = \frac{\partial \theta_{1:K}^\circ}{\partial \delta_{1:K}} \Big|_{(\nu_{1:K}, \eta_{1:K}, \beta, 0_{K \times 1})}$  is the Jacobian matrix of  $\theta_{1:K}^\circ$  with respect to  $\delta_{1:K}$ , evaluated at the point  $(\nu_{1:K}, \eta_{1:K}, \beta, \delta_{1:K} = 0_{K \times 1})$ . Also, we can write

$$B = \frac{\partial \theta_{1:K}^\circ}{\partial (\nu_{1:K}^\circ, \eta_{1:K}^\circ, \beta^\circ)} \Big|_{(\nu_{1:K}, \eta_{1:K}, \beta, 0_{K \times 1})} \cdot \frac{\partial (\nu_{1:K}^\circ, \eta_{1:K}^\circ, \beta^\circ)}{\partial \delta_{1:K}} \Big|_{(\nu_{1:K}, \eta_{1:K}, \beta, 0_{K \times 1})}.\tag{S3.6.6}$$

**Claim S5.** *The first term in (S3.6.6) is given by*

$$\begin{aligned}\left.\frac{\partial \theta_k^\circ}{\partial \nu_k^\circ}\right|_{(\nu_{1:K}, \eta_{1:K}, \beta, 0_{K \times 1})} &= \int_{\mathcal{X}} (g'(\nu_k + \eta_k + \beta x) - g'(\nu_k + \beta x)) f_k^{(r)}(x) dx, \\ \left.\frac{\partial \theta_k^\circ}{\partial \eta_k^\circ}\right|_{(\nu_{1:K}, \eta_{1:K}, \beta, 0_{K \times 1})} &= \int_{\mathcal{X}} g'(\nu_k + \eta_k + \beta x) f_k^{(r)}(x) dx, \\ \left.\frac{\partial \theta_k^\circ}{\partial \beta^\circ}\right|_{(\nu_{1:K}, \eta_{1:K}, \beta, 0_{K \times 1})} &= \int_{\mathcal{X}} (g'(\nu_k + \eta_k + \beta x) - g'(\nu_k + \beta x)) x f_k^{(r)}(x) dx,\end{aligned}\tag{S3.6.7}$$

for  $k = 1, \dots, K$ , where we use the notation  $g'(x) = \frac{d}{dx}g(x)$ . All other partial derivatives in the first term of (S3.6.6) are 0.

The second term in (S3.6.6) is given by

$$\left.\frac{\partial(\nu_{1:K}^\circ, \eta_{1:K}^\circ, \beta^\circ)}{\partial \delta_{1:K}}\right|_{(\nu_{1:K}, \eta_{1:K}, \beta, 0_{K \times 1})} = \lim_{n^{(r+e)} \rightarrow \infty} \left[ \mathbb{E} \left( M_1^\top D M_1 \right) \right]^{-1} \mathbb{E} \left( M_1^\top D M_2 \right), \tag{S3.6.8}$$

where

- $M_1$  is the  $n^{(r+e)} \times (2K + d)$  design matrix for model (S3.6.1), containing columns corresponding to  $(\nu_{1:K}, \eta_{1:K}, \beta)$ , and
- The full design matrix is  $[M_1, M_2]$ , where the  $n^{(r+e)} \times K$  matrix  $M_2$  contains columns corresponding to  $\delta_{1:K}$  (i.e., subgroup-specific indicators of the EC group).

**Remark S3.** The Jacobians in  $B$ ,  $\frac{\partial \theta_{1:K}^\circ}{\partial(\nu_{1:K}^\circ, \eta_{1:K}^\circ, \beta^\circ)}$  and  $\frac{\partial(\nu_{1:K}^\circ, \eta_{1:K}^\circ, \beta^\circ)}{\partial \delta_{1:K}}$ , depend on the unknown parameters  $(\nu_{1:K}, \eta_{1:K}, \beta)$  and the unknown RCT covariate distributions  $f_k^{(r)}$  for  $k = 1, \dots, K$ . Therefore  $B$  is unobserved. However,  $B$  can be estimated consistently using the same plug-in estimation strategy described in Remark S1 (using the weighted definition of  $D$ ).

Proposition S3 and Claim S5 can be proved following the same arguments in Section S3.3.2 with a few variations. In particular, Proposition S3 can be proved following the proof of Proposition S1 with the following changes:

- To show that  $\left(\hat{\nu}_{1:K}^{(r+e)}, \hat{\eta}_{1:K}^{(r+e)}, \hat{\beta}^{(r+e)}, \hat{\theta}_{1:K}^{(r+e)}\right)$  converges in probability to some point  $(\nu_{1:K}^\circ, \eta_{1:K}^\circ, \beta^\circ, \theta_{1:K}^\circ)$ , the definitions of the observed log likelihood function  $\mathcal{O}_n$  and the limiting log likelihood  $\mathcal{L}$  should be updated to:
  - include the weights (i.e.,  $w_i^{(r)}, w_i^{(e)}$  in  $\mathcal{O}_n$  and  $w_{i,*}^{(r)}, w_{i,*}^{(e)}$  in  $\mathcal{L}$ ), and
  - use the generic exponential family likelihood function instead of the binomial likelihood function.
- The Taylor expansion of  $\theta_{1:K}^\circ$  at  $\delta_{1:K} = 0_{K \times 1}$  (i.e., expression (S3.6.5)) is based on the same arguments as before.

In addition, Claim S5 can be proved following the proof of Claim S1 but with the updated definition of  $D$  (including the weights and the generic link function  $g$ ) because (i) the first Jacobian in (S3.6.6) only depends on the definition of the difference of means  $\theta_{1:K}$  (expression (S3.6.3)), and (ii) the second Jacobian in (S3.6.6) only depends on Fisher information matrices, which have the same generic form in GLMs.

### S3.7 Supplementary simulations for additional input estimators $\hat{\theta}_{1:K}^{(r+e)}$

#### S3.7.1 Bayesian causal forests

In the setting of Section 3.1 (continuous outcome with covariates), we define  $\hat{\theta}_{1:K}^{(r+e)}$  using Bayesian causal forests. In particular, we consider

1. the Bayesian causal forest model in Hahn et al. (2020),

$$\begin{aligned} E\left(Y_i^{(r)}|W_i^{(r)}, T_i^{(r)}, X_i^{(r)}\right) &= \mu\left(X_i^{(r)}, W_i^{(r)}, w_i^{(r)}\right) + \tau\left(X_i^{(r)}, W_i^{(r)}, w_i^{(r)}\right) T_i^{(r)}, \\ E\left(Y_i^{(e)}|W_i^{(e)}, X_i^{(e)}\right) &= \mu\left(X_i^{(e)}, W_i^{(e)}, w_i^{(e)}\right), \end{aligned} \quad (\text{S3.7.1})$$

where  $\mu$  and  $\tau$  are nonparametric functions that are given independent BART (Bayesian additive regression tree) priors and  $w_i$  denote propensity scores as defined in Section 3.3. We assume that the outcomes  $Y_i^{(r)}$  and  $Y_i^{(e)}$  share the same control mean function  $\mu$  in (S3.7.1) and are Gaussian with variance  $\phi^2$  noise. We use the prior suggested in Hahn et al. (2020) and the R package ‘bcf’.

2. the subgroup-specific treatment effects

$$\theta_k = \frac{1}{n_{k,\cdot}^{(r)}} \sum_{i=1}^{n_{k,\cdot}^{(r)}} E\left(Y_i^{(r)}|W_i^{(r)} = k, T_i^{(r)} = 1, X_i^{(r)}\right) - \frac{1}{n_{k,\cdot}^{(r)}} \sum_{i=1}^{n_{k,\cdot}^{(r)}} E\left(Y_i^{(r)}|W_i^{(r)} = k, T_i^{(r)} = 0, X_i^{(r)}\right)$$

and compute the posterior distribution of  $\theta_k$  under model (S3.7.1). The estimates  $\hat{\theta}_{1:K}^{(r+e)}$  are the posterior mean of  $\theta_{1:K}$ .

3. the RCT-only primary analysis is identical as in Section 3.1.

We harmonize  $\hat{\theta}_{1:K}^{(r+e)}$  to  $\hat{\theta}^{(r)}$  using  $\lambda = \infty$  and  $\Sigma$  equal to the posterior covariance matrix of  $\theta_{1:K}$ .

We conducted simulations using the same data-generating models as in Section 3.1 (see the description of Figure 4). Figure S6 shows the standard deviation, bias, and root mean squared error (RMSE) of the estimates of  $\theta_1$ , averaging over 1,000 replicates per scenario. Discordance is defined as  $E\left|\pi^\top \hat{\theta}_{1:K} - \hat{\theta}^{(r)}\right|$ . We can see that the Bayesian causal forest estimator is typically biased, and when the SDM assumption is met (Scenarios 1 and 2) harmonization reduces its bias and RMSE. In addition, harmonization is able to completely reduce the discordance between the Bayesian causal forest estimator and  $\hat{\theta}^{(r)}$ .

#### S3.7.2 Bayesian logistic regression with borrowing across subgroups

We consider the same setting of Section 3.2 with binary outcomes. There are several approaches to borrow information across subgroups that allow one to leverage external data, including multi-source exchangeability models (Kotalik et al., 2021), commensurate priors (Hobbs et al., 2012), semi-parametric causal forest models (Hahn et al., 2020), and hierarchical random effects models (Jones et al., 2011) among others. Here we define  $\hat{\theta}_{1:K}^{(r+e)}$  using a hierarchical Bayesian model with exchangeable random effects for (i) subgroup-specific control parameters, (ii) subgroup-specific treatment effects, and (iii) subgroup-specific parameters in the external population. In particular, in our simulations:

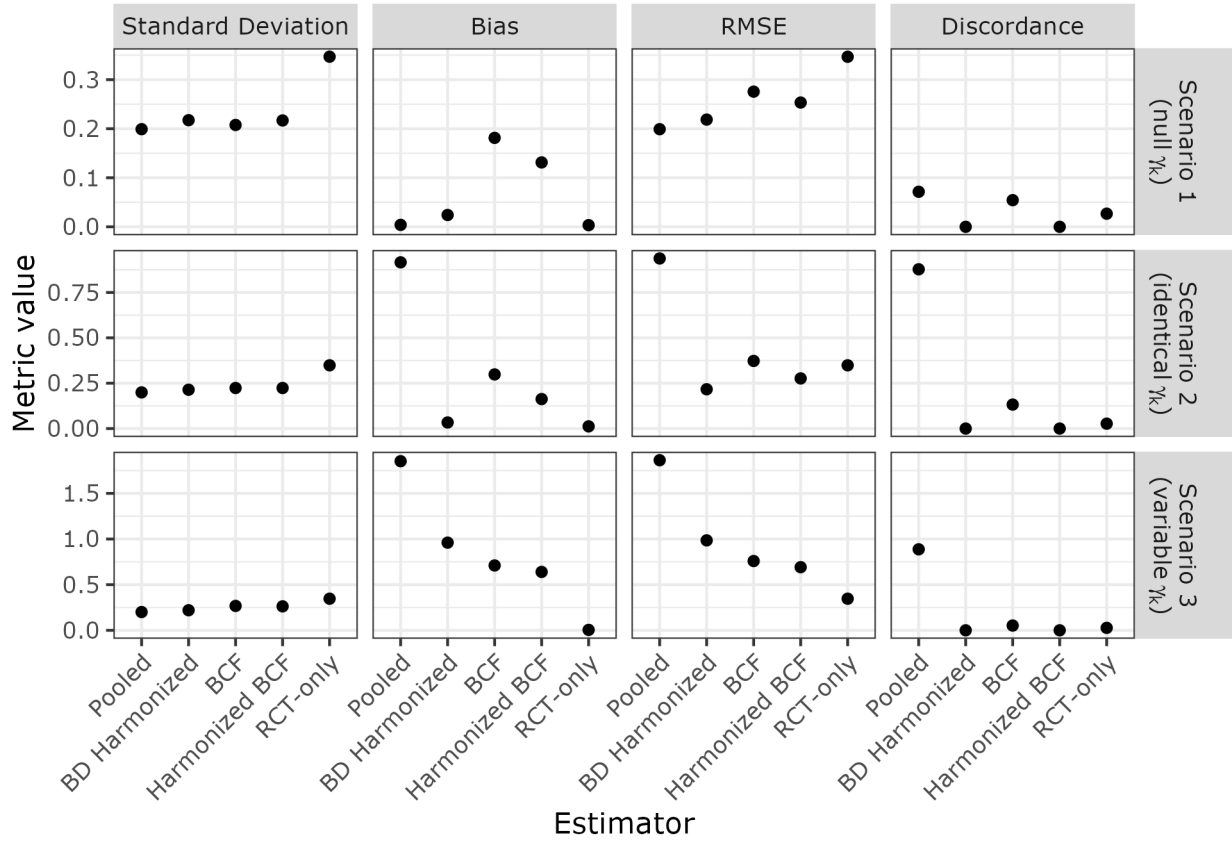

Figure S6: Supplementary simulation study in the linear model setting (Section 3.1). Metrics of interest: Bias, MSE, discordance, standard deviation. Estimators: (1) “Pooled”, as defined in Section 3.1, (2) “BD Harmonized”, the BD harmonized estimator in Section 3.1, (3) “BCF”, the Bayesian causal forest estimator, (4) “Harmonized BCF”, a harmonized version of the causal forest estimator, and (5) “RCT-only”, the RCT-only estimator in Section 3.1.

1. Similarly to Jones et al. (2011), we use the Bayesian hierarchical model

$$\begin{aligned}
p\left(Y_i^{(r)} = 1 | W_i^{(r)}, T_i^{(r)}, X_i^{(r)}\right) &= g\left(\nu_{W_i^{(r)}} + \eta_{W_i^{(r)}} T_i^{(r)} + \beta^\top X_i^{(r)}\right), \\
p\left(Y_i^{(e)} = 1 | W_i^{(e)}, X_i^{(e)}\right) &= g\left(\nu_{W_i^{(e)}} + \delta_{W_i^{(e)}} + \beta^\top X_i^{(e)}\right), \\
\begin{bmatrix} \nu_k \\ \delta_k \\ \eta_k \end{bmatrix} &\stackrel{iid}{\sim} N\left(\begin{bmatrix} m_\nu \\ m_\delta \\ m_\eta \end{bmatrix}, S\right), \quad k = 1, \dots, K,
\end{aligned} \tag{S3.7.2}$$

where  $g(x) = \frac{1}{1+e^{-x}}$  and the exchangeable prior on  $\nu_{1:K}$ ,  $\delta_{1:K}$ , and  $\eta_{1:K}$  induces borrowing of information across subgroups (for the RCT control parameters, the EC distortion parameters, and treatment effects). Model (S3.7.2) is completed with a weakly informative prior on  $m_\nu$ ,  $m_\delta$ ,  $m_\eta$ ,  $\beta \stackrel{iid}{\sim} N(0, 2.5)$  and the prior for the covariance matrix  $S$  is specified following the approach in Goodrich et al. (2020). This model expresses an a priori belief that the RCT control parameters, the EC distortion parameters, and the treatment effects are similar but not identical across subgroups. As previously discussed in the literature, when there is high heterogeneity across subgroups (of  $\nu_k$ ,  $\delta_k$ , or  $\eta_k$ ) estimation may be biased (Jones et al., 2011). More sophisticated approaches to borrow across subgroups and include EC data are possible with other models, for example Kotalik et al. (2021).

We approximate the posterior of model (S3.7.2) using the `rstanarm` R package (Goodrich et al., 2020).

2. We defined the subgroup-specific treatment effects  $\theta_k$  in equation (30) (i.e., the difference of mean outcome probabilities in the RCT population under treatment and control therapies). Then for  $\hat{\theta}_{1:K}^{(r+e)}$  we report the posterior mean of  $\theta_{1:K}$ . We harmonize  $\hat{\theta}_{1:K}^{(r+e)}$  to  $\hat{\theta}^{(r)}$  using  $\lambda = \infty$  and  $\Sigma$  equal to the posterior covariance matrix of  $\theta_{1:K}$  under model (S3.7.2).

In the simulations we have the same data-generating process as in Section 3.2 (logistic model (32), with  $K = 5$  subgroups, and the covariates' distributions used to simulate trials identical to those used for Figure 5). Similarly to the results described in Section 3.2, Figure S7 illustrates that harmonization reduces bias and MSE of the hierarchical Bayesian estimator  $\hat{\theta}_{1:K}^{(r+e)}$  when the SDM assumption holds. We note that in Scenario 1, with identical data distribution in the control arm and the external control group, the hierarchical Bayesian estimator ("HB") is biased as expected due to borrowing of information across subgroups; this bias is reduced through harmonization. The same reduction is observed in Scenarios 2 and 3 and contributes to the MSE reduction in the third column of Figure S7. Across all scenarios, harmonization eliminates discordance between  $\hat{\theta}_{1:K}^{(r+e)}$  and  $\hat{\theta}^{(r)}$ , as expected since  $\lambda = \infty$ .

### S3.7.3 The propensity score adjusted power prior method

Here we consider harmonization of another dynamic borrowing method, the propensity score adjusted power prior method of Lin et al. (2019). We follow the work of Lin et al. (2019) and define  $\hat{\theta}_{1:K}^{(r+e)}$  as follows:

1. For each patient in the RCT and EC, we compute the propensity score  $\hat{p}\left(W_i^{(r)}, X_i^{(r)}\right)$  or

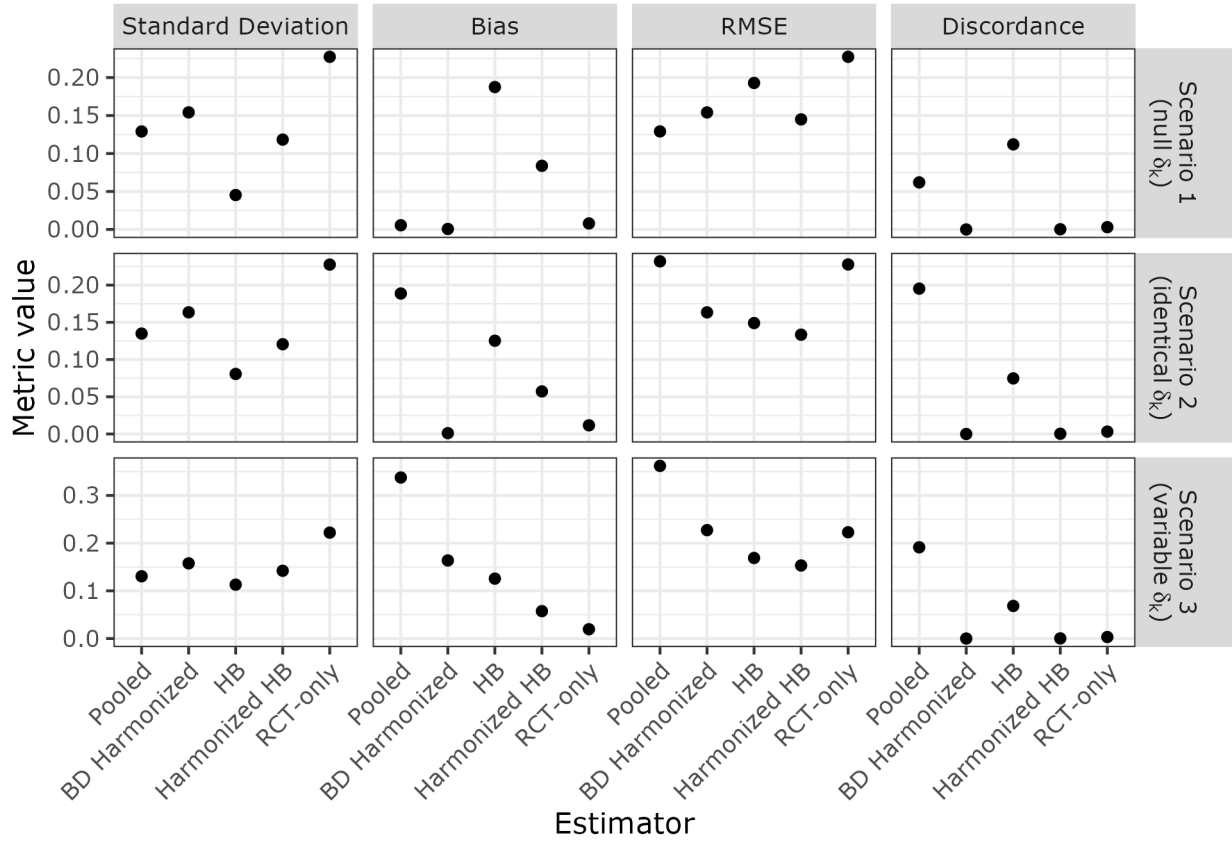

Figure S7: Supplementary simulation study in the logistic model setting (Section 3.2). Metrics of interest: Bias, MSE, discordance, standard deviation. Estimators: (1) “Pooled”, as defined in Section 3.2, (2) “BD Harmonized”, the BD harmonized estimator in Section 3.2, (3) “HB”, the hierarchical Bayesian estimator with borrowing across subgroups, (4) “Harmonized HB”, a harmonized version of the hierarchical Bayesian estimator, and (5) “RCT-only”, the RCT-only estimator in Section 3.2.

$\hat{p}(W_i^{(e)}, X_i^{(e)})$  respectively. Here  $\hat{p}$  is a regression function giving values between 0 and 1 that expresses the relative density of any  $(w, x)$  combination in the RCT population compared to the EC group. We used the same binary regression procedure as in McCaffrey et al. (2004). This is implemented in the twang package in R.

2. Matching is used to select a list of patients  $E'$  from the  $EC$  group (Lin et al., 2019).

3. We consider the likelihood components

$$l_i^{(r)}(\eta_{1:K}, \nu_{1:K}, \beta) = \left[ g\left(\nu_{W_i^{(r)}} + \eta_{W_i^{(r)}} T_i^{(r)} + \beta^\top X_i^{(r)}\right) \right]^{Y_i^{(r)}} \left[ 1 - g\left(\nu_{W_i^{(r)}} + \eta_{W_i^{(r)}} T_i^{(r)} + \beta^\top X_i^{(r)}\right) \right]^{1-Y_i^{(r)}},$$

where  $g(x) = \frac{1}{1+e^{-x}}$ , and

$$l_i^{(e)}(\eta_{1:K}, \nu_{1:K}, \beta) = \left[ g\left(\nu_{W_i^{(e)}} + \beta^\top X_i^{(e)}\right) \right]^{Y_i^{(e)}} \left[ 1 - g\left(\nu_{W_i^{(e)}} + \beta^\top X_i^{(e)}\right) \right]^{1-Y_i^{(e)}}.$$

Like our model (29) in Section 3.2, the unknown parameters are  $(\eta_{1:K}, \nu_{1:K}, \beta)$ . Building on the power prior ideas discussed in Ibrahim et al. (2015)) and Lin et al. (2019)), inference is based on the following distribution

$$p(\eta_{1:K}, \nu_{1:K}, \beta | D^{(r)}, D^{(e)}) \propto \left( \prod_{i=1}^{n^{(r)}} l_i^{(r)}(\eta_{1:K}, \nu_{1:K}, \beta) \right) \times p(\eta_{1:K}, \nu_{1:K}, \beta) \prod_{i \in E'} l_i^{(e)}(\eta_{1:K}, \nu_{1:K}, \beta)^{\hat{p}_i^{(e)}}, \quad (\text{S3.7.3})$$

where  $p(\eta_{1:K}, \nu_{1:K}, \beta)$  is a prior distribution. We sampled from (S3.7.3) using the JAGS software.

4. We define the subgroup-specific treatment effects  $\theta_k$  as in equation (30) (i.e., the difference of mean outcome probabilities in the RCT population under treatment and control therapies). Then for  $\hat{\theta}_{1:K}^{(r+e)}$  we report the posterior mean of  $\theta_{1:K}$ . For  $\hat{\theta}_{1:K}^h$ , we harmonize  $\hat{\theta}_{1:K}^{(r+e)}$  to  $\hat{\theta}^{(r)}$  (as in Section 3.2) using  $\lambda = \infty$  and  $\Sigma$  equal to the posterior covariance matrix of  $\theta_{1:K}$  based on (S3.7.3).

To assess this propensity score adjusted power prior method before and after harmonization, we conducted simulations, using the scenarios in Section 3.2 (logistic model (32),  $K = 5$  subgroups). The distributions used to simulate trials are identical to those used for Figure 5. We computed  $\hat{\theta}_{1:K}^{(r+e)}$  and  $\hat{\theta}_{1:K}^h$  using the outlined procedure. Figure S8 summarizes the results. As for other methods (the Bayesian causal forest and the Bayesian hierarchical model), harmonization of the propensity score adjusted power prior method can reduce bias, RMSE, and discordance between  $\hat{\theta}^{(r)}$  and the subgroup-specific estimates in plausible scenarios.

### S3.8 Testing the systematic distortion mechanism (SDM) assumption

Several approaches can be used to test the SDM assumption. Here we describe an easy to interpret procedure:

1. Specify a model for the RCT and EC data that includes subgroup-specific distortion parameters.

For example

$$Y_i^{(r)} | W_i^{(r)}, T_i^{(r)}, X_i^{(r)} \stackrel{\text{ind.}}{\sim} N\left(\mu_{W_i^{(r)}} + \theta_{W_i^{(r)}} T_i^{(r)} + \beta^\top X_i^{(r)}, \phi^2\right),$$

$$Y_i^{(e)} | W_i^{(e)}, X_i^{(e)} \stackrel{\text{ind.}}{\sim} N\left(\mu_{W_i^{(e)}} + \gamma_{W_i^{(e)}} + \beta^\top X_i^{(e)}, \phi^2\right),$$

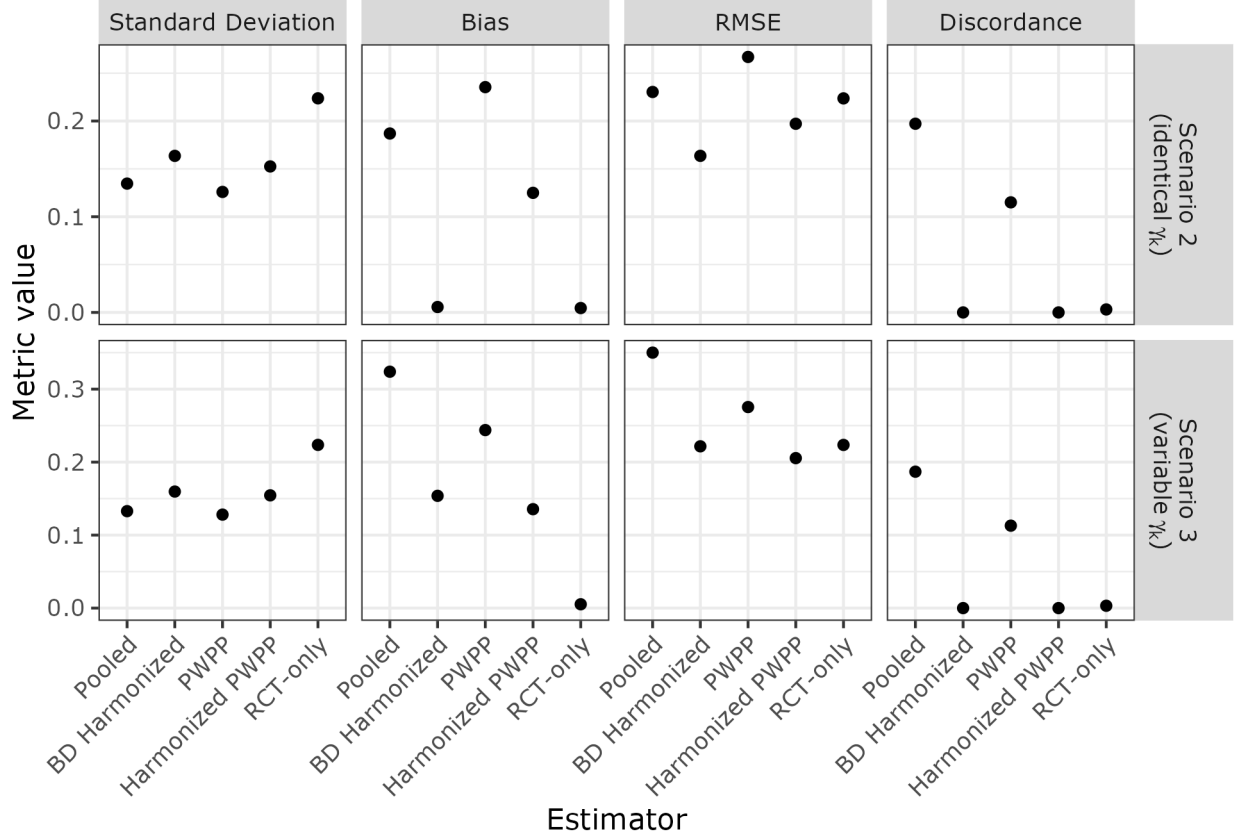

Figure S8: Supplementary simulations. Metrics of interest: Bias, MSE, discordance, and standard deviation. Estimators: (1) “Pooled”, as defined in Section 3.2, (2) “BD Harmonized”, the BD harmonized estimator in Section 3.2, (3) “PWPP”, the propensity score adjusted power prior estimator, (4) the harmonized version of the propensity score adjusted power prior estimator, and (5) the RCT-only estimator, as defined in Section 3.2. Simulation scenarios are identical to those described in Section 3.2. We considered 1,000 replicates per scenario.

where  $\gamma_{1:K}$  is the subgroup-specific distortion parameter, as in Section 3.1, or a GLM (e.g., model (32) in Section 3.2).

2. Conduct (A) a likelihood ratio test or (B) a bootstrap test of the null hypothesis that the distortion parameter is constant across subgroups. In other words, test the null hypothesis  $H_0 : \gamma_1 = \gamma_2 = \dots \gamma_K = \gamma$  for some  $\gamma \in \mathbb{R}$ .
3. If the test rejects  $H_0$  at a desired level  $\alpha$ , evidence against the SDM assumption is reported.

### S3.9 A bootstrap procedure to estimate and remove the bias $\psi_{1:K}$ of a pooled estimator

In addition to BD harmonization, there are other ways to estimate and subtract the bias  $\psi_{1:K}$ . For example, to analyze datasets  $(D^{(r)}, D^{(e)})$  with binary outcomes, the investigator can consider the following procedure (similar to parametric bootstrap):

1. Using the original datasets  $(D^{(r)}, D^{(e)})$ , estimate by MLE the regression model

$$\begin{aligned} p(Y_i^{(r)} = 1 | W_i^{(r)}, T_i^{(r)}, X_i^{(r)}) &= g(\nu_{W_i^{(r)}} + \eta_{W_i^{(r)}} T_i^{(r)} + \beta^\top X_i^{(r)}), \\ p(Y_i^{(e)} = 1 | W_i^{(e)}, X_i^{(e)}) &= g(\nu_{W_i^{(e)}} + \delta + \beta^\top X_i^{(e)}), \end{aligned} \quad (\text{S3.9.1})$$

where  $g(x) = \frac{1}{1+e^{-x}}$ , and the outcomes are independent. This model includes a SDM.

2. Estimate the bias of  $\hat{\theta}_{1:K}^{(r+e)}$  (defined by equation (31)) as follows:
  - (a) For replicates  $a = 1, \dots, R$ , sample new datasets  $(D_a^{(r)}, D_a^{(e)})$  with identical  $(X, W, T)$  patient profiles as in the actual datasets  $(D^{(r)}, D^{(e)})$  and patient outcomes  $Y$  sampled from the estimated regression model with SDM (S3.9.1).
  - (b) For each replicate  $a$ , compute the pooled estimate  $\hat{\theta}_{1:K,a}^{(r+e)}$  based on  $(D_a^{(r)}, D_a^{(e)})$  and the assumption  $\delta = 0$ .
  - (c) Compute the bias estimate  $\hat{\psi}_{1:K} = R^{-1} \sum_{a=1}^R \hat{\theta}_{1:K,a}^{(r+e)} - \tilde{\theta}_{1:K}^{(SDM)}$ , where  $\tilde{\theta}_{1:K}^{(SDM)}$  is the value of the treatment effect (defined in equation (30)) under model (S3.9.1) with the MLE parametrization (from the 1st step of the procedure).
3. Compute the bias-corrected estimate  $\hat{\theta}_{1:K}^{sub} = \hat{\theta}_{1:K}^{(r+e)} - \hat{\psi}_{1:K}$ .

Importantly,  $\hat{\theta}_{1:K}^{sub}$  does not achieve the paper goal of harmonization (i.e.,  $\pi^\top \hat{\theta}_{1:K}^{sub} \neq \hat{\theta}^{(r)}$ ). Similarly, a treatment effect estimate based directly on model (S3.9.1) does not achieve harmonization.

We illustrate simulations in which we computed  $\hat{\theta}_{1:K}^{sub}$  as well as the BD harmonized estimator  $\hat{\theta}_{1:K}^h$ . The simulation scenarios are identical to those described in Section 3.2 (logistic regression). Figure S9(A) shows that these two estimators present a high correlation of  $> 0.9$ . Figure S9(B) shows that they are based on closely related bias corrections. Figure S9(C) shows that, unlike the harmonized estimator, with  $\hat{\theta}_{1:K}^{sub}$  we have  $\pi^\top \hat{\theta}_{1:K}^{sub} \neq \hat{\theta}^{(r)}$ .

### S3.10 BD harmonization of semiparametric and nonparametric estimators

We illustrate how to compute a BD harmonized estimator in the absence of analytic results (e.g. equation (24)) to derive or estimate the bias  $\psi_{1:K} = E(\hat{\theta}_{1:K}^{(r+e)}) - \theta_{1:K}$ . The idea is to (i) estimate

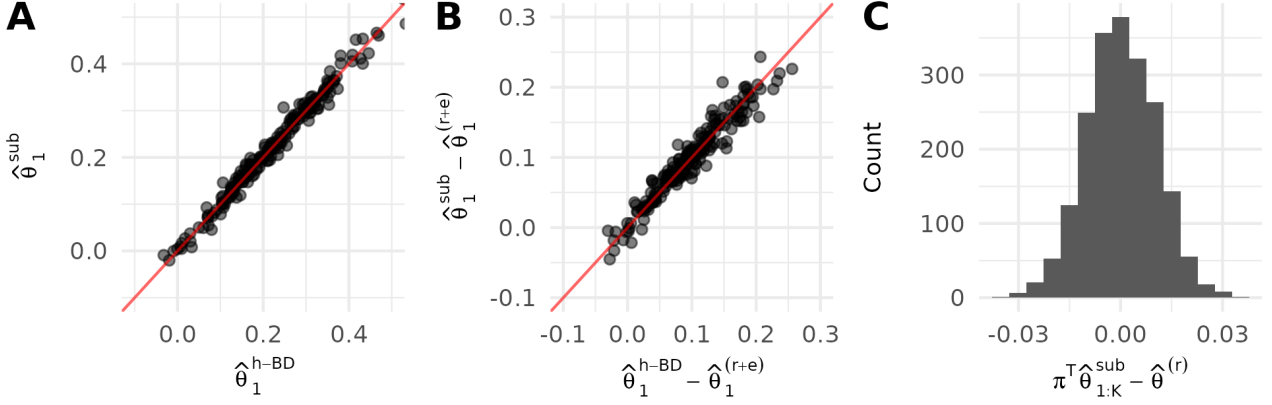

Figure S9: Comparison between  $\hat{\theta}_{1:K}^{sub}$  and  $\hat{\theta}_{1:K}^{h-BD}$  in Section 3.2 (logistic regression). (A) Scatterplot of 200 replicates of the estimates  $\hat{\theta}_{1:K}^{h-BD}$  and  $\hat{\theta}_{1:K}^{sub}$ . (B) Scatterplot of 200 replicates of the bias corrections  $\hat{\theta}_{1:K}^{h-BD} - \hat{\theta}_{1:K}^{h-BD(r+e)}$  and  $\hat{\theta}_{1:K}^{sub} - \hat{\theta}_{1:K}^{h-BD(r+e)}$ . (C) Histogram of 2,000 replicates of the discrepancy  $\pi^\top \hat{\theta}_{1:K}^{sub} - \hat{\theta}^{(r)}$ .

the conditional distributions of  $Y_i^{(r)}$  and  $Y_i^{(e)}$  under the SDM assumption, (ii) resample the outcomes from these distributions and recompute  $R$  times the estimates  $\hat{\theta}_{1:K}^{(r+e)}$ , and (iii) calculate the average difference between these  $R$  estimates and the treatment effect in the resampling model.

For example, consider  $\hat{\theta}_{1:K}^{(r+e)}$ , the MLE of  $\theta_{1:K}$  (see equation (30)) based on the model

$$\begin{aligned} Y_i^{(r)} &= \mu_{W_i^{(r)}} + \theta_{W_i^{(r)}} T_i^{(r)} + f(X_i^{(r)}) + \epsilon_i^{(r)}, \\ Y_i^{(e)} &= \mu_{W_i^{(e)}} + f(X_i^{(e)}) + \epsilon_i^{(e)}, \end{aligned} \quad (\text{S3.10.1})$$

where  $\epsilon_i^{(r)}, \epsilon_i^{(e)} \stackrel{iid}{\sim} N(0, \phi^2)$  and the function  $f$  is a natural cubic spline with fixed knots.

There are several possible ways to estimate the bias vector  $\psi_{1:K}$  caused by SDMs. One approach is to:

1. Estimate the conditional distributions  $Y_i^{(r)} | X_i^{(r)}, W_i^{(r)}, T_i^{(r)}$  and  $Y_i^{(e)} | X_i^{(e)}, W_i^{(e)}$  under the assumption that

$$E(Y_i^{(r)} | X_i^{(r)}, W_i^{(r)} = k, T_i^{(r)} = 0) - E(Y_i^{(e)} | X_i^{(e)}, W_i^{(e)} = k) = \gamma,$$

for some  $\gamma \in \mathbb{R}$ . In particular, we can fit the model

$$\begin{aligned} Y_i^{(r)} &= \mu_{W_i^{(r)}} + \theta_{W_i^{(r)}} T_i^{(r)} + f(X_i^{(r)}) + \epsilon_i^{(r)}, \\ Y_i^{(e)} &= \mu_{W_i^{(e)}} + f(X_i^{(e)}) + \gamma + \epsilon_i^{(e)}, \end{aligned} \quad (\text{S3.10.2})$$

where  $\epsilon_i^{(r)}, \epsilon_i^{(e)} \stackrel{iid}{\sim} N(0, \phi^2)$  and  $f$  is a cubic spline with fixed knots. Alternatively, one can consider using neural networks, Gaussian processes, or tree-based models for  $f$ .

2. For replicates  $a = 1, \dots, R$ , sample new datasets  $(D_a^{(r)}, D_a^{(e)})$  with identical  $(X, W, T)$  patient triplets as in the actual datasets  $(D^{(r)}, D^{(e)})$  and patient outcomes  $Y$  sampled from the estimated SDM model (S3.10.2). For each replicate, compute the estimate  $\hat{\theta}_{1:K,a}^{(r+e)}$  based on  $(D_a^{(r)}, D_a^{(e)})$  and model (S3.10.1).

3. Compute the bias estimate  $\hat{\psi}_{1:K} = R^{-1} \sum_{a=1}^R \hat{\theta}_{1:K,a}^{(r+e)} - \tilde{\theta}_{1:K}^{(SDM)}$ , where  $\tilde{\theta}_{1:K}^{(SDM)}$  is the MLE of  $\theta_{1:K}$  based on model (S3.10.2) and the actual data  $(D^{(r)}, D^{(e)})$ .

Then we can harmonize  $\hat{\theta}_{1:K}^{(r+e)}$  using  $\lambda = \infty$  and choosing a  $\Sigma$  matrix that satisfies  $\Sigma \pi \propto \hat{\psi}_{1:K}$ .

### Sampling distributions of the estimators

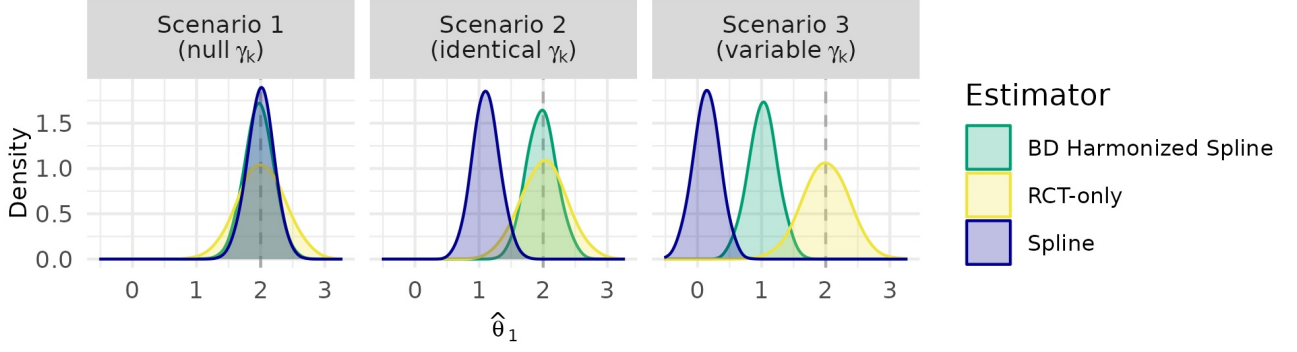

Figure S10: Replication of Figure 4, for alternate estimators defined by model (S3.10.1) (“Spline”) and a BD harmonized version (steps i.-iii., “BD Harmonized Spline”).

We illustrate this strategy by simulating data from the same Scenarios 1-3 as in Section 3.1, but using the spline model (S3.10.1) (with knots at the quintiles of  $X_i$ ) to define  $\hat{\theta}_{1:K}^{(r+e)}$  and steps (i)-(iii) to choose  $\Sigma$ . Figure S10 is nearly identical to Figure 4 in the paper, with the only difference that here  $\hat{\theta}_{1:K}^{(r+e)}$  is based on the spline model (S3.10.1). BD harmonizing has similar effects as those described through Figure 4 when  $\hat{\theta}_{1:K}^{(r+e)}$  is based on the linear model (21).

## S4 Additional material for Section 4

### S4.1 Imputation of censored 12-month survival outcomes

Let  $T_i^{(r)}$  and  $T_i^{(e)}$  be the overall survival (OS) times (in days) for patients in the trial and real world data sets respectively.

In the trial data set, roughly 3% of patients had their OS time censored before 12 months of follow up. In the real world data set roughly 9% of patients were similarly censored. We singly imputed the 12-month overall survival status for these patients as follows:

1. Separately for each data set  $s = r, e$  estimate the Cox model

$$h(t|X_i^{(s)}) = h_0(t) \exp\{\beta^\top X_i^{(s)}\},$$

where  $h(t|X_i^{(s)})$  is the conditional hazard at time  $t$ ,  $h_0(t)$  is the baseline hazard at time  $t$ , and  $X_i^{(s)}$  is a covariate vector including patient  $i$ ’s age, sex, Karnofsky performance status, MGMT methylation status, and extent of resection. We use the `coxph` function in R to fit the models.

2. Separately for each data set estimate the survival function  $P(T_i^{(s)} > t|X_i^{(s)})$ , using the fitted Cox model from step 1 and the Kalbfleisch-Prentice method (via the `survfit` function in R).
3. For a patient  $i$  in study  $s$  censored at time  $t_0 < 365$ , the probability that their true overall survival time  $T_i^{(s)}$  is

$$p_i^{(s)} = \frac{P(T_i^{(s)} > 365|X_i^{(s)})}{P(T_i^{(s)} > t_0|X_i^{(s)})}.$$

4. For censored patients, set their missing 12-month overall survival status  $Y_i^{(s)} = 1$  with probability

$p_i^{(s)}$  and  $Y_i^{(s)} = 0$  otherwise.

## S4.2 Detailed results

|                    | Pooled | Weighted | Harmonized | RCT-Only |
|--------------------|--------|----------|------------|----------|
| <b>Subgroup 1</b>  |        |          |            |          |
| Bias               | -0.040 | -0.016   | 0.016      | 0.011    |
| Standard Deviation | 0.083  | 0.092    | 0.097      | 0.131    |
| RMSE               | 0.092  | 0.094    | 0.098      | 0.131    |
| <b>Subgroup 2</b>  |        |          |            |          |
| Bias               | -0.118 | -0.086   | -0.012     | -0.002   |
| Standard Deviation | 0.053  | 0.060    | 0.081      | 0.086    |
| RMSE               | 0.129  | 0.105    | 0.082      | 0.086    |
| <b>Subgroup 3</b>  |        |          |            |          |
| Bias               | -0.084 | -0.042   | -0.027     | -0.001   |
| Standard Deviation | 0.107  | 0.118    | 0.119      | 0.173    |
| RMSE               | 0.136  | 0.125    | 0.122      | 0.173    |
| <b>Subgroup 4</b>  |        |          |            |          |
| Bias               | -0.017 | -0.015   | 0.022      | -0.002   |
| Standard Deviation | 0.058  | 0.063    | 0.069      | 0.087    |
| RMSE               | 0.061  | 0.065    | 0.073      | 0.087    |

Table S1: Operating characteristics of the four estimators in the simulations of Section 4. Results are based on 1,000 *in silico* GBM trials/EC data sets simulated as described in Section 4.

## S5 Harmonization in the presence of omitted variable bias

*Importance of the definition of  $\hat{\theta}_{1:K}^{(r+e)}$ .* First, we note that the influence of model misspecification on treatment effect's estimates depends on the definition of  $\hat{\theta}_{1:K}^{(r+e)}$ . Some subgroup analysis procedures, including approaches developed in the causal inference literature over the past few decades (Cole and Hernan, 2008; Tipton, 2013), may be more robust to various types of model misspecification compared to MLEs. As we emphasize in Supplementary Section S3.7, harmonization can be applied to any subgroup analysis estimator  $\hat{\theta}_{1:K}^{(r+e)}$ .

*An example of harmonization when  $\hat{\theta}_{1:K}^{(r+e)}$  is based on a misspecified model.* To illustrate how harmonization performs when  $\hat{\theta}_{1:K}^{(r+e)}$  is based on a misspecified model, we conduct simulations in a setting similar to the one in Section 3.1 (linear model) but with a quadratic term in the true data-generating model. The quadratic component is not included in the working model used to compute  $\hat{\theta}_{1:K}^{(r+e)}$ . For simplicity,  $K = 2$  and we have only a single covariate  $X$ . The true data-generating model has conditional moments

$$\begin{aligned}
E\left(Y_i^{(r)}|W_i^{(r)}, T_i^{(r)}, X_i^{(r)}\right) &= \mu_{W_i^{(r)}} + \theta_{W_i^{(r)}} T_i^{(r)} + \beta_1 X_i^{(r)} + \beta_2 X_i^{(r)2}, \\
E\left(Y_i^{(e)}|W_i^{(e)}, X_i^{(e)}\right) &= \mu_{W_i^{(e)}} + \gamma_{W_i^{(e)}} + \beta_1 X_i^{(e)} + \beta_2 X_i^{(e)2}, \text{ and} \\
Var\left(Y_i^{(r)}|W_i^{(r)}, T_i^{(r)}, X_i^{(r)}\right) &= Var\left(Y_i^{(e)}|W_i^{(e)}, X_i^{(e)}\right) = 1,
\end{aligned} \tag{S5.0.1}$$

that is the mean functions are quadratic, not linear, in  $X$ . The distribution of  $X$  depends on both the subgroup and data source (RCT or external), with  $\log X_i^{(r)} | \left[W_i^{(r)} = k\right] \stackrel{iid}{\sim} N\left(\frac{k}{5}, 0.25^2\right)$  in the RCT

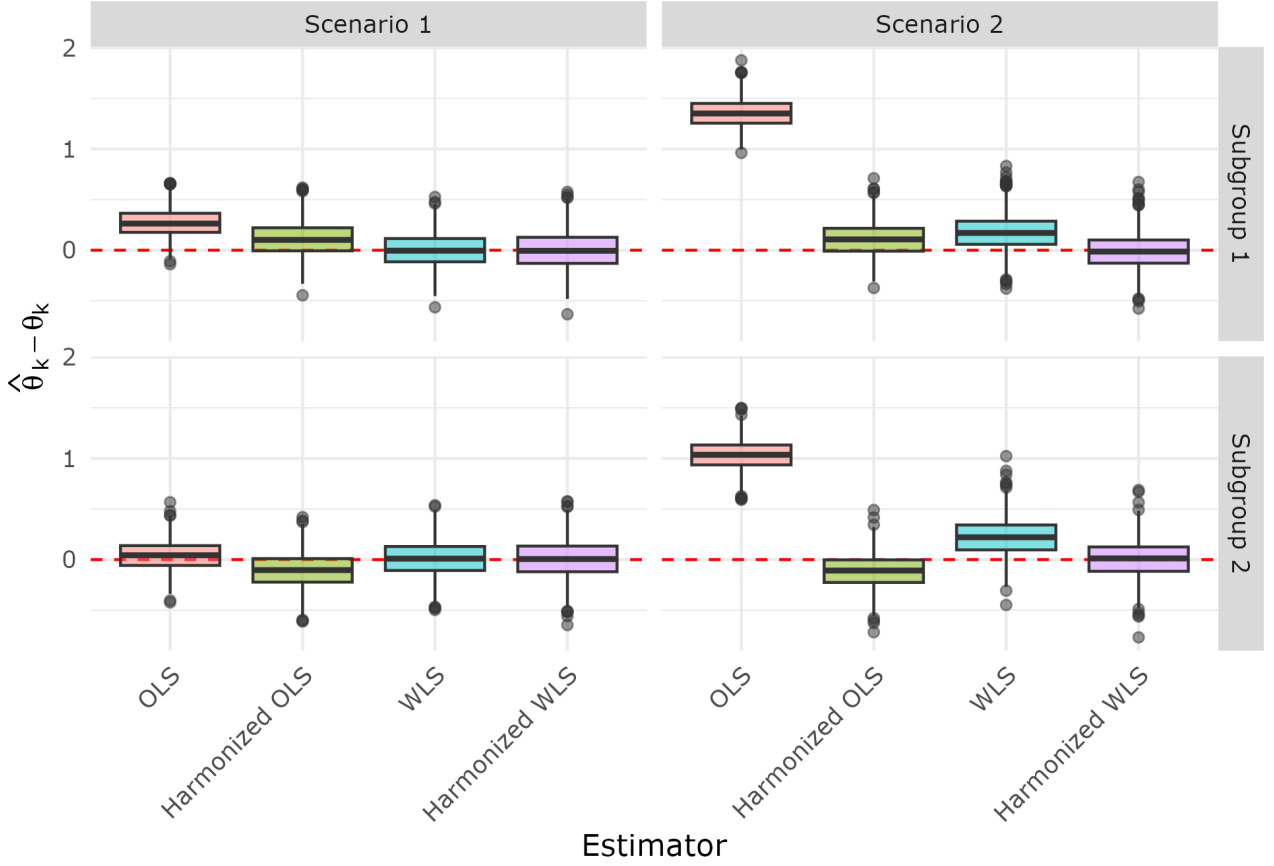

Figure S11: An example with model misspecification. Sampling distributions (boxplots, from 2,000 simulation replicates) of four subgroup estimators. The distributions used to generate the data have been described in the previous paragraphs. We include (i) a pooled OLS estimator as in (21) with only a linear term for  $X$ , (ii) a weighted least squares (WLS) estimator with only a linear term for  $X$  but propensity score weighting as defined in Section 3.3, and (iii-iv) BD-harmonized versions of the pooled OLS and WLS estimators (see Proposition 2).

and  $\log X_i^{(e)} | [W_i^{(e)} = k] \stackrel{iid}{\sim} N(\frac{1}{2} + \frac{k}{5}, 0.25^2)$  in the EC. Also, the RCT control group intercepts are  $\mu_{1:2} = (0, 2)$ , the treatment effects are  $\theta_{1:2} = (0, 2)$ , and the regression coefficients are  $\beta_1 = \beta_2 = 0.5$ . We consider a “Scenario 1” where the EC data have no distortion mechanism with  $\gamma_{1:2} = (0, 0)$  and a “Scenario 2” where there is a systematic distortion mechanism with  $\gamma_{1:2} = (-2, -2)$ . The RCT has sample sizes  $n_{1,1}^{(r)} = n_{2,1}^{(r)} = 100$  and  $n_{1,0}^{(r)} = n_{2,0}^{(r)} = 50$  (i.e. 2:1 randomization), while the EC has sample sizes  $n_{1,0}^{(e)} = n_{2,0}^{(e)} = 150$ .

In Figure S11 we show the sampling distributions (obtained by simulations) of four estimators of  $\theta_{1:2}$ : (i) a pooled OLS estimator as in (21) with only a linear term for  $X$ , (ii) a BD-harmonized version of the OLS estimator (see Proposition 2), (iii) a weighted least squares (WLS) estimator with just a linear term for  $X$  but propensity score weighting as defined in Section 3.3, and (iv) a BD-harmonized version of the WLS estimator (see Proposition 2). Even in Scenario 1, where the EC data have no distortions, the misspecified OLS estimator can have moderate bias ( $= 0.27$  in subgroup  $k = 1$ ). In contrast, WLS estimator using propensity scores is more robust to a misspecified outcome regression and the bias is negligible in Scenario 1. In both scenarios harmonization tends to reduce the bias of the OLS and WLS estimates  $\hat{\theta}_{1:K}^{(r+e)}$ .

*An analytic result.* We focus on a class of scenarios that includes the the previous example and

potential unmeasured confounders. We discuss with analytic expressions the bias before and after harmonization. The estimators  $\hat{\theta}_{1:K}^{(r+e)}$  and  $\hat{\theta}_{1:K}^h$  are defined exactly as in Section 3.1. In other words,  $\hat{\theta}_{1:K}^{(r+e)}$  is the OLS estimator under model (21) and  $\hat{\theta}_{1:K}^h$  is the BD harmonized version of  $\hat{\theta}_{1:K}^{(r+e)}$ , which is computed assuming model (21) and the SDM assumption ( $\gamma_1 = \dots = \gamma_K$ ).

We assume that the true data-generating model has conditional moments

$$\begin{aligned} E\left(Y_i^{(r)}|W_i^{(r)}, T_i^{(r)}, X_i^{(r)}, Z_i^{(r)}\right) &= \mu_{W_i^{(r)}} + \theta_{W_i^{(r)}} T_i^{(r)} + \beta^\top X_i^{(r)} + \xi^\top Z_i^{(r)}, \\ E\left(Y_i^{(e)}|W_i^{(e)}, X_i^{(e)}, Z_i^{(e)}\right) &= \mu_{W_i^{(e)}} + \gamma_{W_i^{(e)}} + \beta^\top X_i^{(e)} + \xi^\top Z_i^{(e)}, \text{ and} \\ \text{Var}\left(Y_i^{(r)}|W_i^{(r)}, T_i^{(r)}, X_i^{(r)}, Z_i^{(r)}\right) &= \text{Var}\left(Y_i^{(e)}|W_i^{(e)}, X_i^{(e)}, Z_i^{(e)}\right) = \phi^2. \end{aligned} \quad (\text{S5.0.2})$$

Here  $Z_i^{(r)}$  and  $Z_i^{(e)}$  are vectors of unmeasured confounders. The design matrix for model (S5.0.2) may be written as  $M = \begin{bmatrix} M_1 & M_2 & M_3 \end{bmatrix}$ , where:  $M_1$  contains the columns corresponding to  $\mu_{1:K}$ ,  $\theta_{1:K}$ , and  $\beta$  (i.e., those in the working model used to compute  $\hat{\theta}_{1:K}^{(r+e)}$ );  $M_2$  contains the columns corresponding to  $\gamma_{1:K}$  (i.e., the EC distortion mechanism); and  $M_3$  contains the columns corresponding to  $\xi$  (i.e., omitted covariates). Note that the simulation example (S5.0.1) above is a special case of (S5.0.2).

Under model (S5.0.2), when the SDM assumption holds ( $\gamma_k = \gamma$  for all  $k = 1, \dots, K$  and some  $\gamma \in \mathbb{R}$ ) the pooled estimator has bias

$$\text{Bias}\left(\hat{\theta}_{1:K}^{(r+e)}, \theta_{1:K}\right) = \gamma b + \epsilon_{1:K}, \quad \text{with} \quad (\text{S5.0.3})$$

$$b = \begin{bmatrix} 0_{K \times K} & I_K & 0_{K \times d} \end{bmatrix} \left(M_1^\top M_1\right)^{-1} M_1^\top M_2 \mathbf{1}_{K \times 1}, \quad \text{and}$$

$$\epsilon_{1:K} = \begin{bmatrix} 0_{K \times K} & I_K & 0_{K \times d} \end{bmatrix} \left(M_1^\top M_1\right)^{-1} M_1^\top M_3 \xi.$$

This result can be derived through linear algebra, very similarly to the derivations in Supplementary Section S3.1.1. Here  $\gamma b$  is the bias when there are no omitted covariates (see equation (24) when  $\gamma_1 = \dots = \gamma_K = \gamma$ ) and  $\epsilon_{1:K}$  is the additional bias in  $\hat{\theta}_{1:K}^{(r+e)}$  due to the omitted covariates (note that  $\hat{\theta}_{1:K}^{(r+e)} = 0_{K \times 1}$  when the omitted covariate regression coefficient  $\xi$  is null).

Since harmonization is a linear transformation of  $\hat{\theta}_{1:K}^{(r+e)}$  and  $\hat{\theta}^{(r)}$  we can derive the bias of  $\hat{\theta}_{1:K}^h$ :

$$\text{Bias}\left(\hat{\theta}_{1:K}^h, \theta_{1:K}\right) = \epsilon_{1:K} - \left(\frac{\pi^\top \epsilon_{1:K}}{\pi^\top \gamma b}\right) \gamma b. \quad (\text{S5.0.4})$$

Similar expressions for the bias can be obtained when the subjects are weighted using propensity score arguments, though the results would be asymptotic. The asymptotic bias would be the same as (S5.0.3) except the terms  $M_1^\top M_1$ ,  $M_1^\top M_2$ , and  $M_1^\top M_3$  need to be replaced by  $M_1^\top D M_1$ ,  $M_1^\top D M_2$ , and  $M_1^\top D M_3$ , where  $D$  is a diagonal matrix of asymptotic weights (see Supplementary Section S3.6 where we explain the role of the weights  $D$ ).

From the bias expressions (S5.0.3) and (S5.0.4) we can see that harmonization can either reduce or increase the bias of  $\hat{\theta}_k^{(r+e)}$ . The comparison between the biases before and after harmonization depends primarily on (a) the joint distribution of the omitted covariates and the variables in the model used to compute  $\hat{\theta}_{1:K}^{(r+e)}$  (i.e.,  $M_1^\top M_3$ ) and (b) the magnitude of the omitted covariate coefficients  $\xi$ . The expressions (S5.0.3) and (S5.0.4) can be useful to explore the sensitivity of the estimators  $\hat{\theta}_{1:K}^{(r+e)}$  and  $\hat{\theta}_{1:K}^h$ .

## References

- S. R. Cole and M. A. Hernan. Constructing Inverse Probability Weights for Marginal Structural Models. *American Journal of Epidemiology*, 168(6):656–664, July 2008. ISSN 0002-9262, 1476-6256. doi: 10.1093/aje/kwn164. URL <https://academic.oup.com/aje/article-lookup/doi/10.1093/aje/kwn164>.
- Ben Goodrich, Jonah Gabry, Imad Ali, and Sam Brilleman. *rstanarm*: Bayesian applied regression modeling via Stan., 2020. URL <https://mc-stan.org/rstanarm>.
- P. Richard Hahn, Jared S. Murray, and Carlos M. Carvalho. Bayesian Regression Tree Models for Causal Inference: Regularization, Confounding, and Heterogeneous Effects (with Discussion). *Bayesian Analysis*, 15(3), September 2020. ISSN 1936-0975. doi: 10.1214/19-BA1195. URL <https://projecteuclid.org/journals/bayesian-analysis/volume-15/issue-3/Bayesian-Regression-Tree-Models-for-Causal-Inference--Regularization-Confounding/10.1214/19-BA1195.full>.
- Brian P. Hobbs, Daniel J. Sargent, and Bradley P. Carlin. Commensurate Priors for Incorporating Historical Information in Clinical Trials Using General and Generalized Linear Models. *Bayesian Analysis*, 7(3), September 2012. ISSN 1936-0975. doi: 10.1214/12-BA722. URL <https://projecteuclid.org/journals/bayesian-analysis/volume-7/issue-3/Commensurate-Priors-for-Incorporating-Historical-Information-in-Clinical-Trials-Using/10.1214/12-BA722.full>.
- Joseph G. Ibrahim, Ming-Hui Chen, Yeongjin Gwon, and Fang Chen. The power prior: theory and applications. *Statistics in Medicine*, 34(28):3724–3749, December 2015. ISSN 0277-6715. doi: 10.1002/sim.6728. URL <https://onlinelibrary.wiley.com/doi/10.1002/sim.6728>.
- Hayley E Jones, David I Ohlssen, Beat Neuenschwander, Amy Racine, and Michael Branson. Bayesian models for subgroup analysis in clinical trials. *Clinical Trials*, 8(2):129–143, April 2011. ISSN 1740-7745, 1740-7753. doi: 10.1177/1740774510396933. URL <http://journals.sagepub.com/doi/10.1177/1740774510396933>.
- Ales Kotalik, David M Vock, Eric C Donny, Dorothy K Hatsukami, and Joseph S Koopmeiners. Dynamic borrowing in the presence of treatment effect heterogeneity. *Biostatistics*, 22(4):789–804, October 2021. ISSN 1465-4644, 1468-4357. doi: 10.1093/biostatistics/kxz066. URL <https://academic.oup.com/biostatistics/article/22/4/789/5715612>.
- Junjing Lin, Margaret Gamalo-Siebers, and Ram Tiwari. Propensity-score-based priors for Bayesian augmented control design. *Pharmaceutical Statistics*, 18(2):223–238, March 2019. ISSN 1539-1604, 1539-1612. doi: 10.1002/pst.1918. URL <https://onlinelibrary.wiley.com/doi/10.1002/pst.1918>.
- D. V. Lindley and A. F. M. Smith. Bayes Estimates for the Linear Model. *Journal of the Royal Statistical Society Series B: Statistical Methodology*, 34(1):1–18, September 1972. ISSN 1369-7412,

1467-9868. doi: 10.1111/j.2517-6161.1972.tb00885.x. URL <https://academic.oup.com/jrsssb/article/34/1/1/7027158>.

Daniel F. McCaffrey, Greg Ridgeway, and Andrew R. Morral. Propensity Score Estimation With Boosted Regression for Evaluating Causal Effects in Observational Studies. *Psychological Methods*, 9(4):403–425, December 2004. ISSN 1939-1463, 1082-989X. doi: 10.1037/1082-989X.9.4.403. URL <https://doi.apa.org/doi/10.1037/1082-989X.9.4.403>.

Elizabeth Tipton. Improving Generalizations From Experiments Using Propensity Score Subclassification: Assumptions, Properties, and Contexts. *Journal of Educational and Behavioral Statistics*, 38(3):239–266, June 2013. ISSN 1076-9986, 1935-1054. doi: 10.3102/1076998612441947. URL <http://journals.sagepub.com/doi/10.3102/1076998612441947>.

Halbert White. Consequences and Detection of Misspecified Nonlinear Regression Models. *Journal of the American Statistical Association*, 76(374):419–433, June 1981. ISSN 0162-1459, 1537-274X. doi: 10.1080/01621459.1981.10477663. URL <http://www.tandfonline.com/doi/abs/10.1080/01621459.1981.10477663>.
